# Supplementary material for: Generating Novel Scene Compositions from Single Images and Videos
Source: arXiv:2103.13389 source file (2023-12-13)
Supplement: Supplementary file 1 [file DR.tex]

\section{Additional analysis of diversity regularization}
\label{sec:app_DR}

\subsection{Ablation on the strength of the proposed diversity regularization}
\label{supp:lambda_dr}

The proposed diversity regularization (DR) is an essential component for SIV-GAN to achieve high diversity among generated samples. For all our experiments in the main paper we used DR with $\lambda=0.15$. In Table \ref{table:lambda_dr}, we show the effect of setting different $\lambda$ for DR in the Single Image setting, changing the strength of the diversity regularization. We note a general quality-diversity trade-off which is present for the Single Image setting. While diversity metrics favour diverse multi-modal outputs, the image quality metrics, such as SIFID, are computed based on similarity to the training frame, so they penalize variations from the original image \citep{Robb2020FewShotAO}. 
%We thus use SIFID at the lowest scale ($\frac{H \times W}{16}$), which corresponds to the low-level quality, such as textures, irrespective to variations in high-level patterns, such as layouts. 
Table \ref{table:lambda_dr} illustrates that setting the multiplier too high ($\lambda=0.50$) leads to good diversity, but harms image quality, while setting small values ($\lambda=[0.00, 0.05]$) is beneficial for quality, but deteriorates diversity. We observed that using $\lambda = 0.15$ leads to a good trade-off, resulting in a high diversity among generated samples, while not corrupting the quality of textures and the global layout coherency, so we picked this value for the final version of the model.

\input{supplementary/tables/lambdas_dr}

\subsection{Effect of the proposed diversity regularization on other GAN models}
\label{supp:DR_others}

To examine the effect of the proposed DR on other models, we trained SinGAN, ConSinGAN and FastGAN with the DR added to the GAN objective. Following our design, this loss was computed in the feature space, as in Eq. \ref{loss_DR}. When training the multi-stage single-image GANs from \cite{Shaham2019SinGANLA, Hinz2020ImprovedTF}, we applied the DR during training of each stage. To select $\lambda$, we tested the models with the values from Table \ref{table:lambda_dr} $(0.05, 0.15, 0.50)$, and chose the highest coefficient that improved diversity but did not lead to a very high SIFID, indicating reduced low-level quality of generated images. 

The performance of the models with DR, as well as our selected $\lambda$ values are included to Table \ref{table:other_with_DR}. As seen from the table, DR plays the biggest role in combination with SIV-GAN, while applying DR to other methods leads only to minor improvement in diversity ($0.01-0.03$ MS-SSIM). For the single image GANs \citep{Shaham2019SinGANLA, Hinz2020ImprovedTF} this is explained by their multi-stage training schemes: their discriminators already overfit to all possible patches at a given scale, so the DR does not help to learn more diverse combinations. Single branch discriminator of the few-shot model \citep{anonymous2021towards} overfits easily when trained with very little data, and DR alone cannot correct this. We conclude that our two-branch discriminator is crucial to leverage the benefit of the proposed diversity regularization.

\begin{table}
	\vspace{-0.5em}
	\setlength{\tabcolsep}{0.35em}
	
	\centering
	\caption{Effect of DR applied to different GAN models in the Single Image setting on DAVIS-YFCC100M.}
	\vspace{0.5em}
	\begin{tabular}{cc|c|c|c|c|c}
		\multirow{2}{*}{{} Method} & {{DR} } & \multirow{2}{*}{{} SIFID~$\downarrow$} & \multirow{2}{*}{{} LPIPS~$\uparrow$ } & \multirow{2}{*}{{} MS-SSIM~$\downarrow$} & {{} Pixel ~$\uparrow$} & {Dist.}  \tabularnewline
		& {$\lambda$} & & & & {} Diversity & to train \tabularnewline
		
		\hline 	\hline 	
		
		{{} \multirow{2}{*}{SinGAN }} & { -} &  \textbf{{{0.13}}}  &  \textbf{{0.26}} & {0.69} &  {0.54} &  {0.24} \tabularnewline
		 & { 0.15} &  {{0.15}}  &   \textbf{{0.26}} &  \textbf{{0.68}} &  \textbf{{0.55}}  &  \textbf{0.26} \tabularnewline 	\hline

		{{} \multirow{2}{*}{ConSinGAN }} & { -} &  \textbf{{{0.09}}}  &   {0.29} &  {0.65} &  {0.59}  &  {0.25} \tabularnewline
& { 0.05} &  {{0.11}}  &   \textbf{{0.30}} &  \textbf{{0.63}} &  \textbf{{0.60}}  &  \textbf{0.28}  \tabularnewline 	\hline 
		
		{{} \multirow{2}{*}{FastGAN  }} & { -} &  \textbf{{{0.13}}}  &   {0.18} &  {0.77} &{0.49}  &  {0.08}  \tabularnewline
& { 0.15} &  {{0.14}}  &   \textbf{{0.21}} &  \textbf{{0.74}} &  \textbf{{0.52}}  &  \textbf{0.13}  \tabularnewline 	\hline 
	
		{{} \multirow{2}{*}{SIV-GAN  }} & { -} &  \textbf{{{0.05}}}  &  {0.04} & {0.95} & {0.33}  &  {0.06}  \tabularnewline
& { 0.15} &  {{0.08}}  &  \textbf{{0.33}} & \textbf{{0.63}} &  \textbf{{0.66}}  &  \textbf{0.31} \tabularnewline 
		
	\end{tabular}
	%\vspace{-0.5em}
	\label{table:other_with_DR} %
	\vspace{-1em}
\end{table}
