# Supplementary material for: Generating Novel Scene Compositions from Single Images and Videos
Source: arXiv:2103.13389 source file (2023-12-13)
Supplement: Supplementary file 2 [file architecture.tex]

\section{Detailed description of the architecture and training details}
\label{sec:architecture}

\subsection{Analysis of strategies to generate images of rectangular shapes}
\label{supp:interpolations}

Commonly used state-of-the-art GAN models, such as \citep{Brock2019, karnewar2019msg}, generate images of square shapes. In our studied settings, single images or video frames can be rectangular, having resolutions of different horizontal and vertical aspect ratios. In contrast, we design our model to be compatible with images of different resolutions. In this section, we analyse two possible strategies to achieve this.

\begin{wrapfigure}{R}{0.5\textwidth}
	\begin{centering}
		\setlength{\tabcolsep}{0.0em}
		
		\par\end{centering}
	\begin{centering}
		\vspace{-1em}
		%\hfill{}%
		\begin{tabular}{@{}c@{\hskip 0.01in}c@{\hskip 0.05in}c@{}}
		 &\multicolumn{2}{c}{\hspace{-0.1in} \small Progressive upsampling}  
			\tabularnewline	
	 \multirow{-2}{*}{\begin{tabular}{c}  Training image \\ 	\includegraphics[width=0.3\linewidth, height=0.07\textheight]{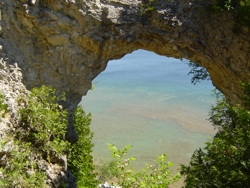}\end{tabular}  } & 
			\includegraphics[width=0.3\linewidth, height=0.07\textheight]{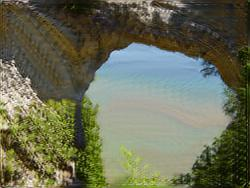} & 
			\includegraphics[width=0.3\linewidth, height=0.07\textheight]{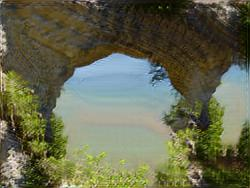} 	\tabularnewline
			& \multicolumn{2}{c}{ \hspace{-0.1in}  \small Adjusted noise} \tabularnewline
			
			& \includegraphics[width=0.3\linewidth, height=0.07\textheight]{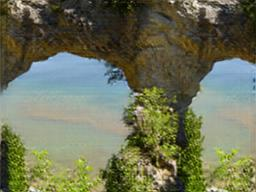} & 
			\includegraphics[width=0.3\linewidth, height=0.07\textheight]{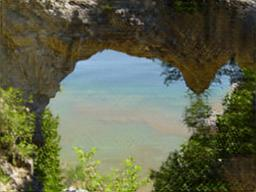}
		% & 	\includegraphics[width=0.3\linewidth]{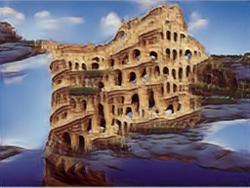}
			
			\tabularnewline

		\end{tabular}\hfill{}
		\par\end{centering}
	\vspace{-0.5em}
	\caption{\label{fig:interpolations} Different strategies to achieve rectangular shapes. Using progressive upsampling, as in \citep{Shaham2019SinGANLA}, leads to artifacts in textures (e.g. chequered "waves" on the rock). Controlling output image resolution through adjusting noise shape helps to overcome this issue and generate textures of good quality.
		%	As the middle and latest stages cannot correct the layout decision of the first scale generators, without a careful balancing the model falls into producing images of very low diversity or generating incoherent layouts.
	}
	\vspace{-1em}
\end{wrapfigure}

\begin{table}[b]

	\setlength{\tabcolsep}{0.2em}
	
	\centering
	\caption{Effect of different strategies to match the rectangular shape of the original training image on the DAVIS-YFCC100M dataset. }
	\vspace{0.5em}	
	\begin{tabular}{c|c|c||c|c}
		 \multirow{2}{*}{ Interpolation} & \multicolumn{2}{c||}{Single Image}  & \multicolumn{2}{c}{Single Video}  
		\tabularnewline
		 \small{} & {{} SIFID~$\downarrow$}  & {{} LPIPS~$\uparrow$ } &  {{} SIFID~$\downarrow$} & {{} LPIPS~$\uparrow$ } \tabularnewline

		\hline 	\hline 	
		
		 {} Progressive upsampling & {{0.11}} &  {0.32} &  {0.65} &  {0.42}  \tabularnewline

		 {} Adjusted noise & \textbf{{{0.08}}}  &  \textbf{{0.33}} &  \textbf{{0.55}} &  \textbf{{0.43}}  \tabularnewline
	
		\end{tabular}
	\vspace{-0.5em}

\label{table:interpolations} %

\end{table}

One possible strategy is to follow the design of SinGAN \citep{Shaham2019SinGANLA}, which has several training stages. Such model proposes to reach the final resolution following a geometric progression, where the image is upsampled after each training stage. In this scheme, the progression multiplier is computed based on the image size, the number of stages, and a predefined image size at first model stage. Typically, this multiplier is non-integer and is different for horizontal and vertical axes. For SIV-GAN, we adopted such scheme by progressively upsampling the image after each generator block, starting from noise of shape $(4\times 4)$ and reaching the exact image shape by the final generator layers. In our experiments, such upsampling scheme leads to texture artefacts in generated images (see Fig. \ref{fig:interpolations}). We observed that the artefacts are caused by non-integer interpolation between layers: backpropagation through such transformation causes a "grid" effect, which is hard to correct during training of the generator. The difference in the texture quality in comparison to \cite{Shaham2019SinGANLA, Hinz2020ImprovedTF} is explained by the fact that these models are trained in multiple stages, without requiring backpropagation through upsampling layers. In contrast, our SIV-GAN is a single stage model, and gradients cannot bypass the interpolation.

To avoid corruptions of textures, we therefore select an alternative solution. As discussed in App. \ref{supp:architecture}, we propose to follow the architecture of \cite{Brock2019}, employing x2 upsampling after each residual block, but modifying the shape of input noise, adjusting it to fit better to the final image resolution. Note that for this approach the final resolution of generated images is an even multiple of the input noise shape, which can sometimes not precisely fit to the resolution of an original image (for example, in case when the training image has an odd number of pixels in one of the dimensions). Nevertheless, with such approach the shape of an image is preserved better, compared to generating square images as in \citep{Brock2019, karnewar2019msg}. As seen from Fig.~\ref{fig:interpolations}, adjusting the noise shape leads to better quality of images, overcoming the interpolation problem. 

Table \ref{table:interpolations} confirms our analysis. We observe that using the progressive upsampling, as in \cite{Shaham2019SinGANLA}, leads to decreased quality of images, as measured by SIFID. Moreover, such approach produces slightly lower diversity. Therefore, for our final model design, we choose to adjust input noise shape, as it leads to better performance.

\subsection{Architecture and training details}
\label{supp:architecture}

Architecture details of our SIV-GAN are summarized in Tables \ref{table:g_arch} and \ref{table:d_arch}. Our model has a generator $G$ and a discriminator $D$ consisting of three parts: low-level feature extractor $D_{low-level}$, layout branch $D_{layout}$, and content branch $D_{content}$. Our design mainly follows the one of BigGAN \citep{Brock2019}, applying ResNet blocks at both the generator and the discriminator. Following MSG-GAN \citep{karnewar2019msg}, we use skip-connections between $G$ and $D$. We thus generate images at different resolutions and pass them to discriminator at different scales. In contrast to \citep{karnewar2019msg}, our discriminator is not symmetric to generator, as after $N_{low-level}$ discriminator blocks we apply branching. Therefore, we generate images only at $N_{low-level}$ highest resolutions, and then pass them at each block of $D_{low-level}$. To incorporate generated images at intermediate $D$ blocks, we apply a $1\times 1$ convolution, and concatenate the obtained tensor to the current $D$ features (strategy $\phi_{lin\_cat}$ from \citep{karnewar2019msg}.)

The branches $D_{layout}$ and $D_{content}$ are formed by usual $D$ ResNet blocks, with two modifications. First, as the content branch has $1\times 1$ spatial dimensions, the used convolutions have kernel size ($1\times 1$) and are technically equivalent to a fully-connected layer. Secondly, the layout branch has $1$ channel, so its convolutions always have the number of channels equal to $1$. To form a binary real-fake decision tensor, after each $D$ block we use a $1\times 1$ convolution, which maps the current features to a one-channel map with logits. 

In order to fit better to the training image size, we change the resolution of the input noise. We keep the noise resolution around $(4\times4)$, adjusting it to different ratios to fit shapes of training images closer. For example, the input noise in our experiments was resized to $(3\times 4), (3\times 5)$ or $(4\times 4)$, depending on the final image resolution. For evaluation, we bilinearly resized generated images to the resolution of original training image.
Tables \ref{table:g_arch} and \ref{table:d_arch} present an example for input noise of resolution $3\times5$, which correspond to the frames from the DAVIS video dataset \citep{pont20172017}.

We train our model with ADAM \citep{adamopt} optimizer, using a batch size of 5, momentums $(\beta_1, \beta_2) = (0.5, 0.999)$, learning rates $0.0002$ for both the generator and the discriminator. All our experiments were conducted on a single GTX 1080 GPU with 12 GB RAM memory.

\begin{table}[h!]
	
	\setlength{\tabcolsep}{0.25em}
	
	\centering
	\centering
	\caption{The SIV-GAN generator. In this example, the configuration is presented for the input noise of size $(3\times 5)$ and the final resolution of $(192\times320)$, corresponding to training on the DAVIS-YFCC100M dataset in the Single Video setting.}
	
	\vspace{0.5em}
	\begin{tabular}{l|l l|l l}
		 Operation  & Input  & Size &  Output  & Size  \tabularnewline
		\hline
		\hline
{ConvTransp2D} & \texttt{z} & (64,1,1)          & {\texttt{up\_0}}  & {(256,3,5)}\\ \hline
		{ResBlock-Up} & \texttt{up\_0}  & (256,3,5)   & {\texttt{up\_1}} & {(256,3,5)} \\ 
		\hline
		{ResBlock-Up} & \texttt{up\_1}  & (256,3,5)   & {\texttt{up\_2}} & {(256,6,10)} \\ 
		\hline
		{ResBlock-Up} & \texttt{up\_2}  & (256,6,10)   & {\texttt{up\_2}} & {(256,12,20)} \\ 
		\hline
		{ResBlock-Up} & \texttt{up\_3}  & (256,12,20)   & {\texttt{up\_3}} & {(256,24,40)} \\ \hline
		{ResBlock-Up} & \texttt{up\_4}  & (256,24,40)   & {\texttt{up\_4}} & {(256,48,80)} \\ \hline
        {ResBlock-Up} & \texttt{up\_5}  & (256,48,80)   & {\texttt{up\_5}} & {(128,96,160)} \\ \hline
		{ResBlock-Up} & \texttt{up\_6}  & (128,96,160)   & {\texttt{up\_6}} & {(64,192,320)} \\ \hline \hline
		Conv2D, TanH           & \texttt{up\_5} & (128,48,80)     & \texttt{image\_2}  & (3,48,80)\\\hline
		Conv2D, TanH           & \texttt{up\_6} & (64,96,160)     & \texttt{image\_1}  & (3,96,160)\\\hline
		Conv2D, TanH           & \texttt{up\_7} & (32,192,320)     & \texttt{image\_0}  & (3,192,320)\\\hline

	\end{tabular}

\label{table:g_arch} %

\end{table}

\begin{table}[h!]
	\setlength{\tabcolsep}{0.25em}

\centering
\centering
	\caption{The SIV-GAN discriminator. In this example, the configuration is presented for the input noise of size $(3\times 5)$ and the final resolution of $(192\times320)$, corresponding to training on the DAVIS-YFCC100M dataset in the Single Video setting.}

\vspace{0.5em}

	\begin{tabular}{l|l l|l l}
		 Operation  & Input  & Size &  Output  & Size  \tabularnewline
		\hline
		\hline
		\multicolumn{5}{c}{Low-level features $D_{low-level}$} \\ \hline
		Conv2D & \texttt{image\_0} & (3,192,320)              & \texttt{feat\_0}  & (32,192,320)\\\hline 
		Conv2D & \texttt{image\_1} & (3,96,160)              & \texttt{feat\_1}  & (8,96,160)\\\hline 
		Conv2D & \texttt{image\_2} & (3,48,80)              & \texttt{feat\_2}  & (16,48,80)\\\hline 		
{ResBlock-Down} & 
		\texttt{feat\_0} & (32,192,320) & {\texttt{down\_0}} & {(64,96,160)} \\ \hline
		\multirow{2}{*}{ResBlock-Down} & \texttt{down\_0} & (64,96,160) & \multirow{2}{*}{\texttt{down\_1}} & \multirow{2}{*}{(128,48,80)} \\
& \texttt{feat\_1} & (8, 96, 160) & & \\ \hline
		\multirow{2}{*}{ResBlock-Down} & \texttt{down\_1} & (128,48,80) & \multirow{2}{*}{\texttt{F}} & \multirow{2}{*}{(256,24,40)} \\
& \texttt{feat\_2} & (16,48, 80) & & \\ \hline \hline
		\multicolumn{5}{c}{Content branch $D_{content}$} \\ \hline
		AvgPool & \texttt{F} & (256,24,40)   & \texttt{F\_con} & (256,1,1) \\\hline
		ResBlock-Down & \texttt{F\_con} & (256,1,1)   & \texttt{cont\_0} & (256,1,1) \\\hline
		ResBlock-Down & \texttt{cont\_0} & (256,1,1)   & \texttt{cont\_1} & (256,1,1) \\\hline
		ResBlock-Down & \texttt{cont\_1} & (256,1,1)   & \texttt{cont\_2} & (256,1,1) \\\hline
		ResBlock-Down & \texttt{cont\_2} & (256,1,1)     & \texttt{cont\_3} & (256,1,1) \\ \hline \hline
		\multicolumn{5}{c}{Layout branch $D_{layout}$} \\ \hline
		Conv2D & \texttt{F} & (256,24,40)   & \texttt{F\_lay} & (1,24,40) \\\hline
	ResBlock-Down & \texttt{F\_lay} & (1,24,40)   & \texttt{lay\_0} & (1,12,20) \\\hline
	ResBlock-Down & \texttt{lay\_0} & (1,12,20)   & \texttt{lay\_1} & (1,6,10) \\\hline
	ResBlock-Down & \texttt{lay\_1} & (1,6,10)   & \texttt{lay\_2} & (1,3,5) \\\hline
	ResBlock-Down & \texttt{lay\_2} & (1,3,5)     & \texttt{lay\_3} & (1,3,5) \\ \hline \hline

	\end{tabular}
\centering

\label{table:d_arch} %

%\end{minipage}%
%\hfill
%\begin{minipage}{.42\linewidth}
%\vspace{-1em}
%\hfill
%\includegraphics[width=0.43\textwidth]{figures/colors-textures/texture_pdf6}
%\hfill
%\vspace{0.2em}
%\captionof{figure}{{Histogram distances to real data.}}	\label{fig:color-texture} %
%\end{minipage}%

		%	\vspace{-0.5em}
\end{table}
