# Supplementary material for: Generating Novel Scene Compositions from Single Images and Videos
Source: arXiv:2103.13389 source file (2023-12-13)
Supplement: Supplementary file 3 [file discriminator.tex]

\section{Additional analysis of the SIV-GAN discriminator}
\label{sec:app_D}

%\subsection{Qualitative results for ablations study on the discriminator structure}
\subsection{Effect of the two branches in the discriminator}
\label{supp:qual_ablations_d}

\input{supplementary/figures/qual_ablations_d}
\begin{figure}[t]
\begin{centering}
\setlength{\tabcolsep}{0.1em}

\par\end{centering}
\begin{centering}
\vspace{-1em}
\hfill{}%
\begin{tabular}{@{\hskip -0.05in}c@{\hskip 0.05in}c@{\hskip 0.05in}c@{\hskip 0.05in}c@{\hskip 0.05in}|c@{\hskip 0.05in}c@{\hskip 0.05in}c@{\hskip 0.05in}c}

\rotatebox{90}{ \hspace{0.5ex}\begin{tabular}{c} \small Video \\ \small frames\end{tabular}} &  \multicolumn{3}{c|}{\hspace{-2.05ex} \includegraphics[width=0.463\linewidth, height=0.075\textheight]{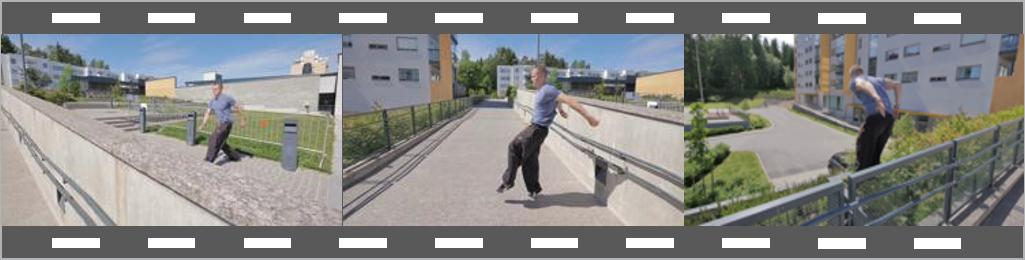} } &
\multicolumn{3}{c}{\includegraphics[width=0.463\linewidth, height=0.075\textheight]{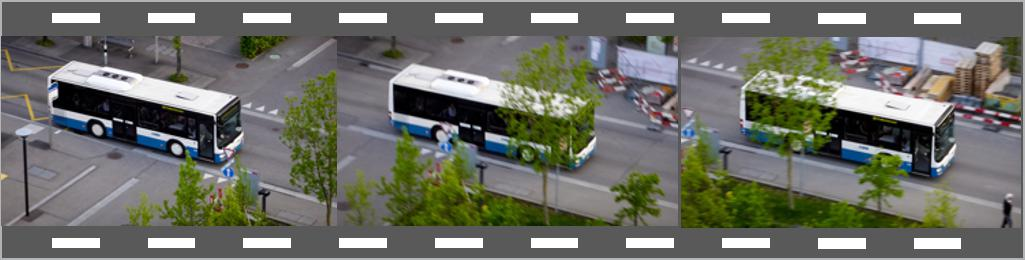}} \tabularnewline

\rotatebox{90}{\hspace{-.9ex}\begin{tabular}{c} \small No \\ \small branches \end{tabular}}&
\includegraphics[width=0.15\linewidth, height=0.06\textheight]{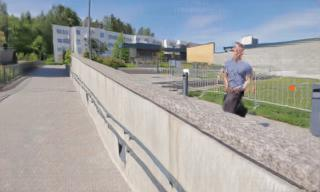} &
\includegraphics[width=0.15\linewidth, height=0.06\textheight]{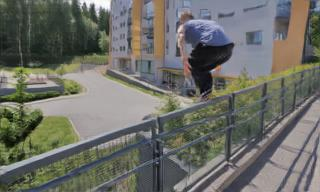} & 
\includegraphics[width=0.15\linewidth, height=0.06\textheight]{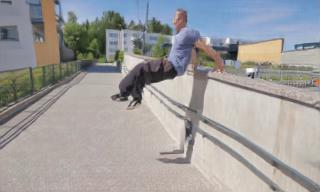} & 
\includegraphics[width=0.15\linewidth, height=0.06\textheight]{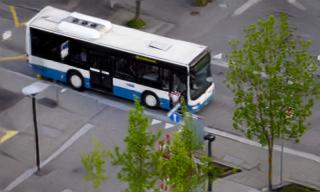} &
\includegraphics[width=0.15\linewidth, height=0.06\textheight]{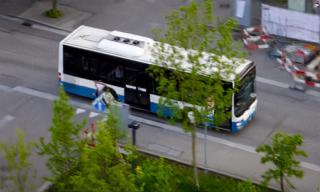} & 
\includegraphics[width=0.15\linewidth, height=0.06\textheight]{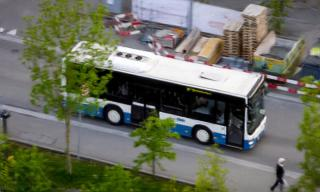} \tabularnewline

\rotatebox{90}{\hspace{-.7ex}\begin{tabular}{c} \small No \\ \small layout \end{tabular}}&
\includegraphics[width=0.15\linewidth, height=0.06\textheight]{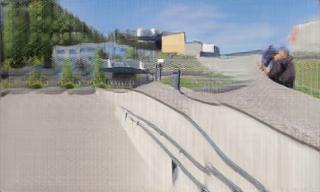} & 
\includegraphics[width=0.15\linewidth, height=0.06\textheight]{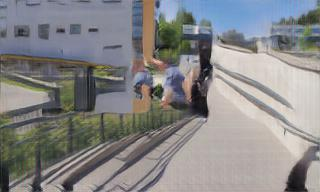} & 
\includegraphics[width=0.15\linewidth, height=0.06\textheight]{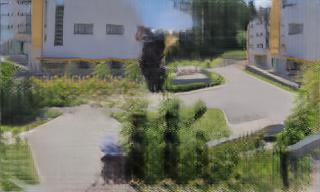} &
\includegraphics[width=0.15\linewidth, height=0.06\textheight]{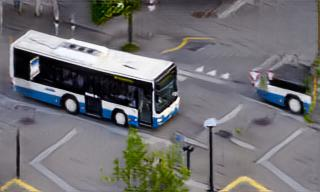} & 
\includegraphics[width=0.15\linewidth, height=0.06\textheight]{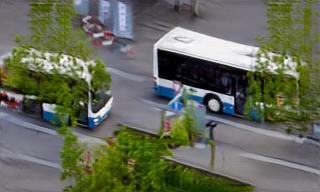} &
\includegraphics[width=0.15\linewidth, height=0.06\textheight]{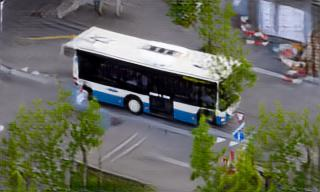}\tabularnewline

\rotatebox{90}{\hspace{-.8ex}\begin{tabular}{c} \small No \\\small content \end{tabular}}&
\includegraphics[width=0.15\linewidth, height=0.06\textheight]{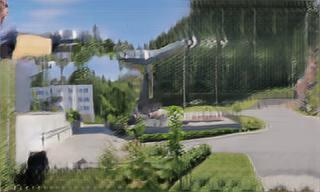} & 
\includegraphics[width=0.15\linewidth, height=0.06\textheight]{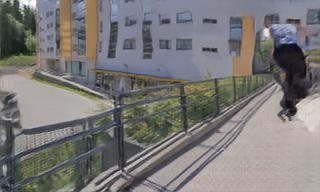} & 
\includegraphics[width=0.15\linewidth, height=0.06\textheight]{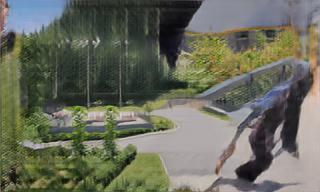} & 
\includegraphics[width=0.15\linewidth, height=0.06\textheight]{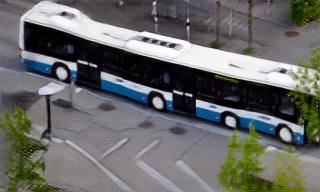} &
\includegraphics[width=0.15\linewidth, height=0.06\textheight]{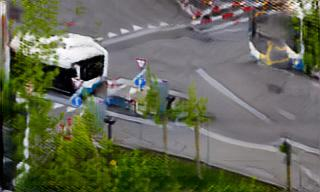} & 
\includegraphics[width=0.15\linewidth, height=0.06\textheight]{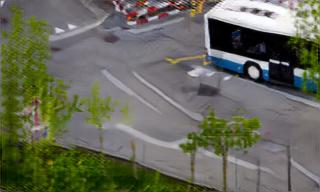}\tabularnewline

\rotatebox{90}{\hspace{-.7ex}\begin{tabular}{c} \small Both \\ \small branches \end{tabular}}&
\includegraphics[width=0.15\linewidth, height=0.06\textheight]{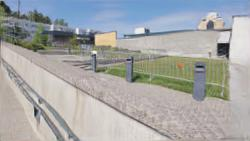} & 
\includegraphics[width=0.15\linewidth, height=0.06\textheight]{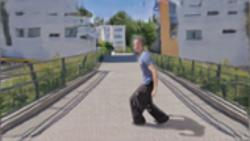} & 
\includegraphics[width=0.15\linewidth, height=0.06\textheight]{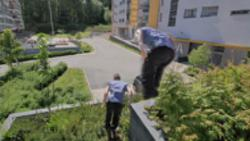} &
\includegraphics[width=0.15\linewidth, height=0.06\textheight]{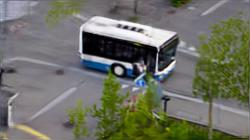} & 
\includegraphics[width=0.15\linewidth, height=0.06\textheight]{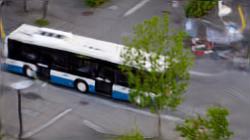} &
\includegraphics[width=0.15\linewidth, height=0.06\textheight]{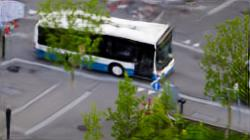}\tabularnewline

\end{tabular}\hfill{}
\par\end{centering}
\vspace{-0.5em}
\caption{\label{fig:qual_abl_video} Visual effects of using content and layout branches in the discriminator in the Single Video setting. 
The model with a standard GAN discriminator (No branches) memorizes the training video frames. The model without the layout branch is prone to cutting objects' contours, generating globally incoherent layouts. The absence of the content branch leads to failures in appearances of objects, such as trees. Finally, the model with both branches generates diverse images maintaining realistic content and layouts.
See Table \ref{table:main_ablation} for qualitative comparison and App.~\ref{supp:qual_ablations_d} for the discussion.
%\anna{add here description of the visual results}
 }
\vspace{-1.0em}
\end{figure}

In Fig. \ref{fig:qual_ablations_d} and \ref{fig:qual_abl_video} we showcase the visual effect of using content and layout branches in the SIV-GAN discriminator. Following the ablation Table \ref{table:main_ablation} in the main paper, we separately show qualitative results for our full discriminator model with content and layout branches, the discriminator without the layout branch, without the content branch, and for a model without both branches, corresponding to a standard GAN discriminator. The visual results illustrate the concepts of "layout" and "content" learnt by the respective branches. Applying the content branch, without the layout branch, leads to the generation of different objects in various combinations, but the model often fails to reproduce correct positioning of objects or globally-coherent layouts. For example, there might be a horizon discontinuity, or air balloons may follow unrealistically structured positions in a grid. In contrast, a model, trained with the layout branch, but without the content branch, generates images with more realistic layouts, but does not preserve the content distribution of the training image, removing objects, distorting their appearance or perturbing their shapes. Behaviour of such models corresponds to high diversity scores and poor low-level SIFID in Table \ref{table:main_ablation}. Employing none of the branches, which corresponds to using a standard GAN discriminator, leads to memorization of the training image, so the model just reproduces the training data (low distance to training set in Table \ref{table:main_ablation}). Finally, our full model with a two-branch discriminator generates plausible diverse images, varying both the image content and the global layout of the scene (0.33 LPIPS and SIFID at scale $\frac{H \times W}{16}$ of 16.3 in the Single Image setting, see Table \ref{table:main_ablation}).

%\subsection{Feature distances between video frames in the content and layout embeddings}
\label{supp:con_lay_embeddings}

To illustrate further our intuition on the discriminator's branches learning content and layout, we analyse the feature distances between real images in the content and layout embeddings of the trained SIV-GAN discriminator. For this, we take the discriminators trained on single ``bus'' and ``parkour'' videos from the DAVIS dataset \citep{pont20172017}. The video sequences have notably different variability in layouts: while there is a significant camera direction movement for the ``parkour'' video, the ``bus'' video captures the vehicle always from the same angle. This leads to a much smaller perceptual differences in layouts for the bus video compared to the parkour video.

\begin{figure}[t]
	%\vspace{-1.5em}
	%\hfill{}%
	\begin{tabular}{@{}c@{\hskip 0.005in}c@{}}	
		\includegraphics[width=0.99\linewidth]{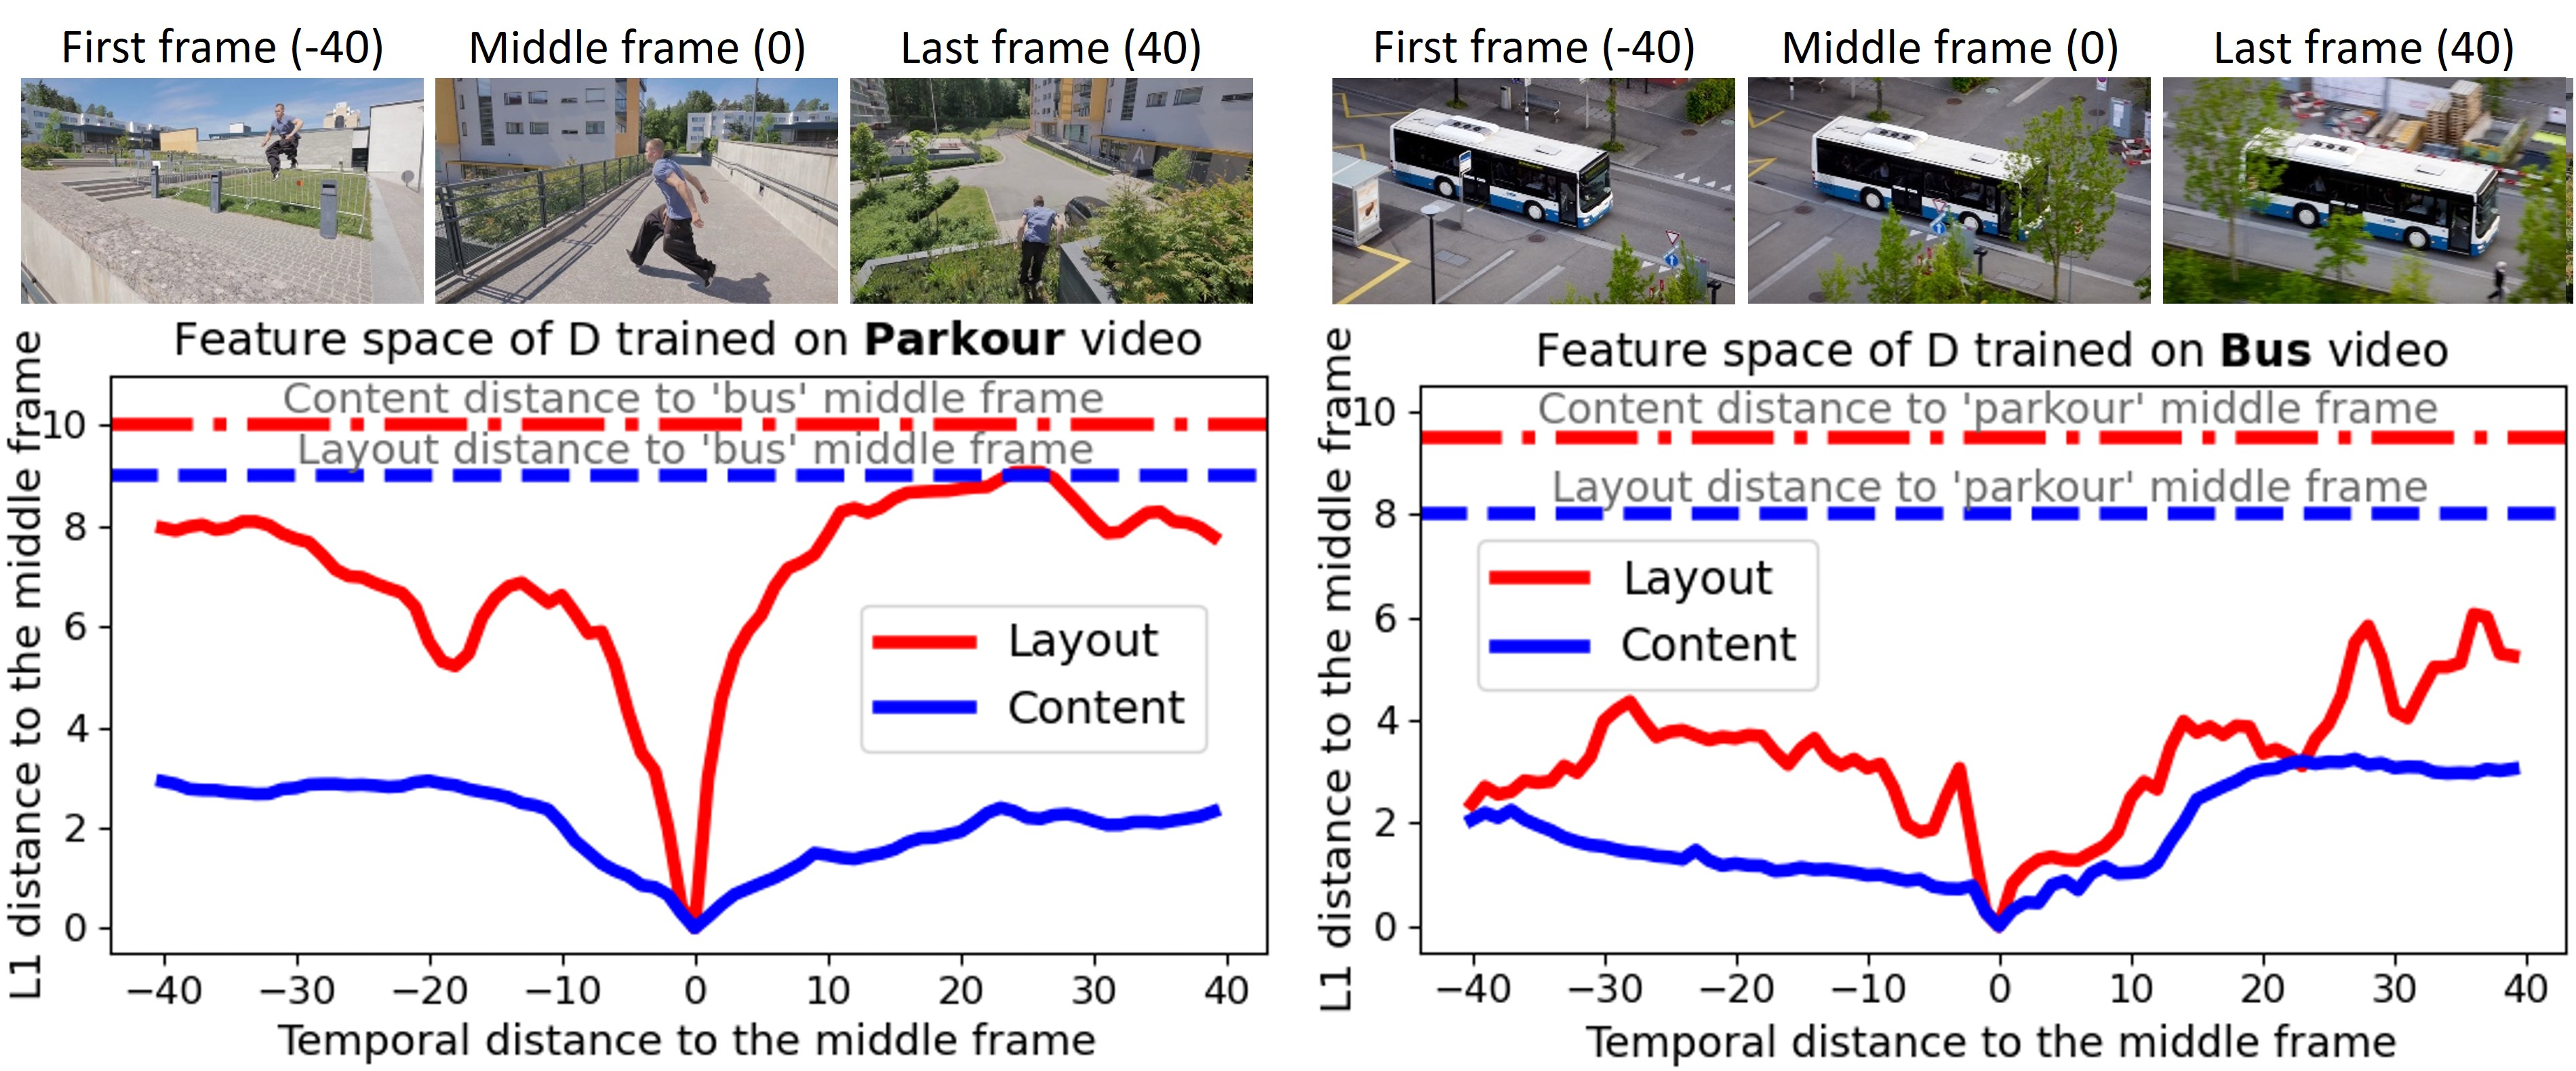} 
	\end{tabular}
	\vspace{-0.8ex}
	\caption{\label{fig:con_lay_embeddings} Feature distances from video frames to middle frame. The layout embedding distances (solid red) between “bus” frames are lower than for the “parkour” video. The content embedding distances between frames of the same sequence (solid blue) are significantly lower than the distance between middle frames of different videos (dashed blue).}
	\vspace{-1.7em}
\end{figure}

In Fig. \ref{fig:con_lay_embeddings} we show the feature distances in the embeddings of SIV-GAN content and layout branches, measured between the middle frame and other frames of the same video sequence. 
We observe that the illustrated distances correlate well with our intuition of $D$ branches learning content and layout. 
Firstly, as nearby frames have very similar content and layouts, the lowest distances both in the content and layout embeddings are between adjacent frames, while increasing the temporal distance from the middle frames leads to higher content and layout feature distances.
Secondly, the embedding differences are consistent with our perceptual judgement: the layout embedding distances (solid red) between ``bus'' frames are notably lower than for the ``parkour'' video. 
%At the same time, the difference between most decorrelated ``parkour'' frames comes almost to the same values as between middle frames of different sequences, highlighting high layout variability for the this video.
Finally, as video frames inside the short videos depict similar content (e.g.  same objects), the content embedding distances between frames of the same sequence (solid blue) are significantly lower than to middle frames of two different videos (dashed blue).

\subsection{Ablation on the number of blocks used before branching}
\label{supp:N_low_level}

\input{supplementary/figures/N_low_level}
\input{supplementary/tables/N_low_level}

The proposed SIV-GAN discriminator has two branches, preceded by a low-level feature extractor. As discussed in Sec. \ref{sec: train_det}, the discriminator consists of 7 ResNet blocks, using 3 ResNet blocks before the branching for $D_{low\text{-}level}$, and 4 ResNet blocks for the both branches $D_{content}$ and $D_{layout}$. In Table \ref{table:N_low_level} and Fig. \ref{fig:N_low_level} we analyse the effect of applying branching at an earlier or a later discrimination stage, keeping the overall depth of the networks equal to 7 ResNet block. The results indicate that the branching should be applied neither too early nor too late. Using too few ResNet blocks (1-2) before the branching leads to a reduced capacity of the low-level feature extractor $D_{low\text{-}level}$, so this network becomes unable to provide the branches with descriptive content and layout representations of an image. As seen from Fig. \ref{fig:N_low_level}, such model learns the color distribution of an image, but cannot produce a globally-coherent scene and generate textures of good quality. In Table \ref{table:N_low_level} this effect is indicated by a very high SIFID. On the other hand, using too many blocks before the branching (5-6) leads to increased capacity of the feature extractor $D_{low\text{-}level}$, so the network can remember the whole image. In this case the model suffers from a memorization effect, reproducing the training image (see Fig. \ref{fig:N_low_level}), and scoring low at diversity metrics (low LPIPS in Table \ref{table:N_low_level}). Finally, we found that using 3 ResNet blocks before the branching leads to an optimal quality-diversity trade-off in both the Single Image and Single Video settings, allowing the generation of high diversity, while preserving the context of original samples.

\subsection{Effect of the number of channels in the layout branch}
\label{supp:layout_width}

In this section we study the effect of varying the number of channels in the layout branch feature representation. For all experiments in the main paper, the layout branch representation is obtained from an intermediate representation by a convolutional layer with one output channel. Table \ref{table:layout_width} shows the effect of using the layout representation with 3, 5, and 10 channels. An increased number of channels in the layout branch results in a more powerful network that can easier memorize the layout representations extracted from real images. Thus, increasing the number of channels results in reduced diversity of samples, as indicated by the smaller LPIPS scores in Table \ref{table:layout_width}. 

\begin{table}[h!]

	\setlength{\tabcolsep}{0.2em}
	
	\centering
	
	\caption{Ablation on the number of channels used for the layout branch feature representation on the DAVIS-YFCC100M dataset. }
	\vspace{0.5em}
	\begin{tabular}{c|c|c||c|c}
		 $F_{layout}$ & \multicolumn{2}{c||}{Single Image}  & \multicolumn{2}{c}{Single Video}  
		\tabularnewline
		 {} channels & {{} SIFID~$\downarrow$}  & {{} LPIPS~$\uparrow$ } &  {{} SIFID~$\downarrow$} & {{} LPIPS~$\uparrow$ } \tabularnewline

		\hline 	\hline

		 1 & {{0.08}}  &  \textbf{{0.33}} &  {0.55} &  \textbf{{0.43}}  \tabularnewline
		 
		 3 & {{0.07}}  &  {0.28} &  {0.54} &  {0.41}  \tabularnewline
		 
		 5 & \textbf{{{0.06}}}  &  {0.25} &  {0.50} &  {0.40}  \tabularnewline
		 
		 10 & \textbf{{0.06}}  &  {0.24} &  \textbf{{0.49}} &  {0.40}  \tabularnewline

		\end{tabular}
%	\vspace{-0.5em}

\label{table:layout_width} %

\end{table}

\subsection{Effect of the low-level loss}
\label{supp:low-level}

\begin{table}
	\vspace{-1.0em}
	\setlength{\tabcolsep}{0.2em}
	
	\centering
	\caption{Ablation on the low-level loss $\mathcal{L}_{D_{low\text{-}level}}$ on DAVIS-YFCC100M dataset. }
	\vspace{0.5em}
	\begin{tabular}{c|c|c||c|c}
		 {} Low-level & \multicolumn{2}{c||}{Single Image}  & \multicolumn{2}{c}{Single Video}  
		\tabularnewline
		 {} loss & {\small{} SIFID~$\downarrow$}  & {{} LPIPS~$\uparrow$ } &  {{} SIFID~$\downarrow$} & {{} LPIPS~$\uparrow$ } \tabularnewline

		\hline 	\hline 	
		
		 \xmark & \textbf{{{0.08}}}  &  {0.27} &  {0.58} &  {0.40}  \tabularnewline
		
		 \cmark & \textbf{{{0.08}}}  &  \textbf{{0.33}} &  \textbf{{0.55}} &  \textbf{{0.43}}  \tabularnewline
	
		\end{tabular}
%	\vspace{-0.5em}

\label{table:low_level_loss} %

\end{table}

In this section we provide an ablation on the low-level discriminator loss $\mathcal{L}_{D_{low\text{-}level}}$. According to Eq.~\ref{eq:loss_d_1} and \ref{eq:loss_d_2}, the loss of the SIV-GAN discriminator is computed after each ResNet block before branching, which means that the attention of the discriminator is shared across different layers, corresponding to image realism at different low-level scales. Without this loss, the discriminator judges images only after branching, paying attention mostly to the high-level image realism. The low-level loss changes the discriminator's task and shifts its attention towards earlier layers, thus increasing its attention to low-level details, e.g., such as textures. As seen from Table \ref{table:low_level_loss}, this property helps to reduce overfitting and allows synthesis of higher diversity, both in the Single Image and Single Video settings.
