# Supplementary material for: Generating Novel Scene Compositions from Single Images and Videos
Source: arXiv:2103.13389 source file (2023-12-13)
Supplement: Supplementary file 4 [file few-shot.tex]

\section{Results on few-shot image synthesis}
\label{sec:app_fewshot}

\subsection{Standard few-shot image synthesis benchmarks}
\label{sec:supp_fewshot_standard}

In addition to the Single Image and Single Video settings, we conduct experiments also for few-shot image synthesis. Under this scenario, the task is to train a generative model on a small dataset, typically containing up to several hundreds of images. We experiment on the commonly used 100-shot datasets from \citep{Zhao2020DifferentiableAF} (Obama, Grumpy Cat, Panda) and on 160- and 389-shot datasets from \citep{si2011learning} (Face-Cat, Face-Dog). 
These datasets have same image resolution of 256x256 and share a common object-centric structure, depicting faces of humans or animals which are centred in all images.

Many methods address few-shot image synthesis in the paradigm of few-shot adaptation, adopting GAN models pre-trained on larger datasets \citep{Wang2018TransferringGG, Mo2020FreezeDA, Noguchi2019ImageGF, Wang2020MineGANEK}). 
Another line of work proposes to stabilize few-shot GAN training from scratch, 
by utilizing differentiable image augmentation (DA) and LeCam consistency regularization (CR) \citep{tseng2021regularizing}, or by using a skip-layer excitation module (SLE) for faster learning of the generator with a self-supervised discriminator \citep{anonymous2021towards}). The two most recent studies, LeCam CR \citep{tseng2021regularizing} and FastGAN \citep{anonymous2021towards}, demonstrated that it is possible to outperform few-shot adaptation methods by using GAN models without pre-training, achieving significantly better performance on the standard few-shot image synthesis benchmarks (see Table \ref{table:few-shot}). We select FastGAN \citep{anonymous2021towards} as our main comparison model as it is the state-of-the-art model with the official implementation code available in open source \footnote{https://github.com/odegeasslbc/FastGAN-pytorch}.

To demonstrate the benefit of the SIV-GAN model design on the few-shot image synthesis task we apply the following modifications.
Since in the few-shot setting the training set contains multiple data instances, we need to increase the capacity of our generator by increasing its depth by one ResNet block and increasing the channel multiplier (overall increasing to $\sim$30M parameters from the original 5M). In order to enable a fast learning of the larger generator we adopt the SLE module of \citet{anonymous2021towards}.
We make two changes to the configuration of our discriminator. Firstly, to closer match the learning capacity of a more heavy-weight generator, we increase the width of our discriminator by doubling the channel multiplier in all layers. This step results in an increase of trainable parameters count from 1.6M to 5M. Secondly, we move the branching point to a later stage, setting $N_{\text{low-level}} = 6$. This step is necessary to follow the structure of object-centric few-shot datasets. As objects in such datasets cover whole images, we observed that the layout decision should be taken at a more global scale (4x4 instead of the previous 32x32 spatial resolution for the layout representation), while the content representation should have a large enough receptive field to see the complete object. Finally, in line with \citep{anonymous2021towards}, we keep the self-supervision loss for discriminator, as we found it to stabilize the training in the few-shot data regime. Further we refer to our extended model as SIV-GAN+.

\begin{table}
	\setlength{\tabcolsep}{0.4em}
	
	\centering

	\caption{Results on the few-shot image synthesis task. The FID is computed between 5000 generated images and the whole training set.  \textbf{Bold} and \underline{underlined} indicate first and second best scores. Our SIV-GAN+ achieves better FID scores compared to FastGAN on all few-shot datasets, also outperforming the model from LeCam~\citep{tseng2021regularizing} on four out of five datasets.}
	\vspace{0.5em}
	\begin{tabular}{l|l|c@{\hskip 0.10in}c@{\hskip 0.10in}c@{\hskip 0.10in}c@{\hskip 0.10in}c}
%	  & \multicolumn{5}{c}{FID~$\downarrow$}  \tabularnewline		\cline{2-6}

	 \multirow{2}{*}{FID~$\downarrow$} & \multicolumn{1}{c|}{ Dataset:} & {} Obama & {} Grumpy Cat & {} Panda & {} Face Cat & {} Face Dog  \tabularnewline \cline{2-7}
	 
	& \multicolumn{1}{c|}{ Number of images:} & {} 100 & {} 100  & {} 100  & {} 160  & {} 389   \tabularnewline
	\hline \hline 
		
		\multicolumn{2}{l|}{Scale/Shift \citep{Noguchi2019ImageGF} \hfill $\circlearrowright$}  &  {50.72}  &  {34.20} & {21.38} &  {54.83} &  {83.04}  \tabularnewline
		\multicolumn{2}{l|}{MineGAN  \citep{Wang2020MineGANEK} \hfill $\circlearrowright$}  &  {50.63}  &  {34.54} & {14.84} &  {54.45} &  {93.08}  \tabularnewline
		\multicolumn{2}{l|}{TransferGAN \citep{Wang2018TransferringGG} \hfill $\circlearrowright$}  &  {48.73}  &  {34.06} & {23.20} &  {52.61} &  {82.38}  \tabularnewline
		%{} TransferGAN + DA  & {} \cmark &  {39.85}  &  {29.77} & {17.12} &  {49.10} &  {65.57}  \tabularnewline
		\multicolumn{2}{l|}{FreezeD \citep{Mo2020FreezeDA} \hfill $\circlearrowright$}  &  {41.87}  &  {31.22} & {17.95} &  {47.70} &  {70.46}  \tabularnewline \hline
		%{} TransferGAN + DA  & {} \cmark &  {35.75}  &  {29.32} & {14.50} &  {46.07} &  {61.03}  \tabularnewline
		%\hline 
		%{} StyleGANv2  &  &  {80.45}  &  {48.63} & {34.07} &  {69.84} &  {129.9}  \tabularnewline
		%{} StyleGANv2 + DA  &  &  {47.09}  &  {27.21} & {12.13} &  {42.40} &  {58.47}  \tabularnewline
		\multicolumn{2}{l|}{LeCam \citep{tseng2021regularizing}}  &  \textbf{{33.16}}  &  \underline{{24.93}} & {10.16} &  {34.18} &  {54.88}  \tabularnewline
		 
		\multicolumn{2}{l|}{FastGAN \citep{anonymous2021towards}}   &  {38.59}  &  {27.08} & \underline{{9.63}} &  \underline{{33.50}} &  \underline{{53.39}}  \tabularnewline
		\multicolumn{2}{l|}{SIV-GAN+}  &  \underline{{35.10}}  &  \textbf{{23.79}} & \textbf{{9.22}} &  \textbf{{31.24}} &  \textbf{{50.05}}  \tabularnewline
		\multicolumn{7}{r}{$\circlearrowright$ - models which use pre-training}
		
	\end{tabular}
	\vspace{-1.5em}
	\label{table:few-shot} %
\end{table}

\begin{figure}[t]
\begin{centering}
\setlength{\tabcolsep}{0.1em}

\par\end{centering}
\begin{centering}

\hfill{}%
\begin{tabular}{l@{\hskip 0.05in}l@{\hskip 0.05in}l@{\hskip 0.12in}l@{\hskip 0.05in}l@{\hskip 0.05in}l}
	
\multicolumn{3}{c}{FastGAN, trained on \textbf{full dataset} (389 images)} &
\multicolumn{3}{c}{SIV-GAN+, trained on \textbf{full dataset} (389 images)}
\tabularnewline
 
\includegraphics[width=0.157\linewidth]{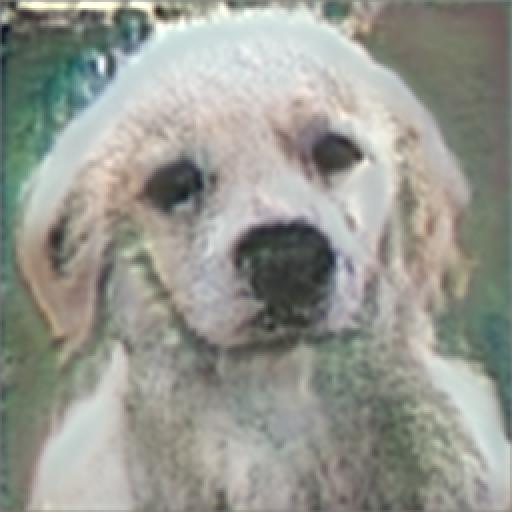} &
\includegraphics[width=0.157\linewidth]{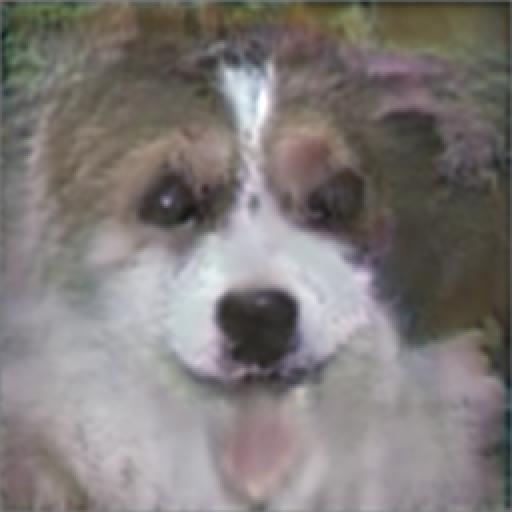} &
\includegraphics[width=0.157\linewidth]{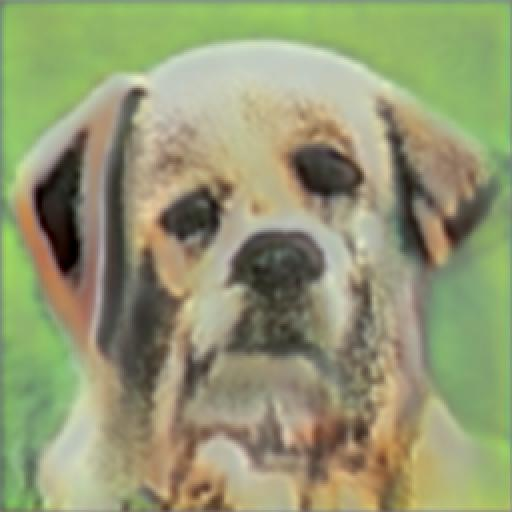} &
\includegraphics[width=0.157\linewidth]{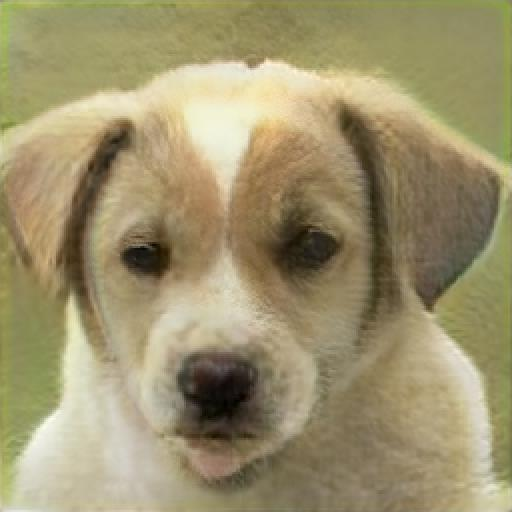} &
\includegraphics[width=0.157\linewidth]{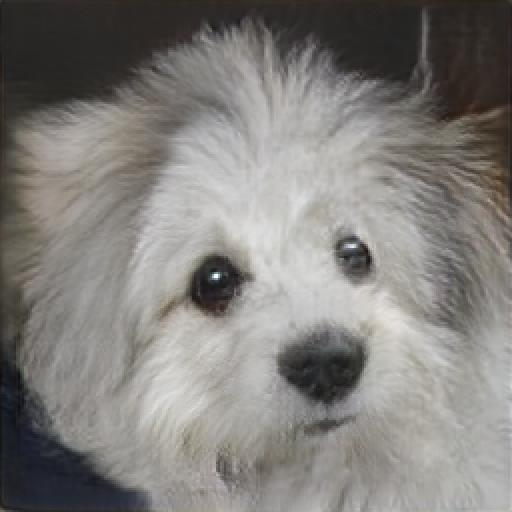} &
\includegraphics[width=0.157\linewidth]{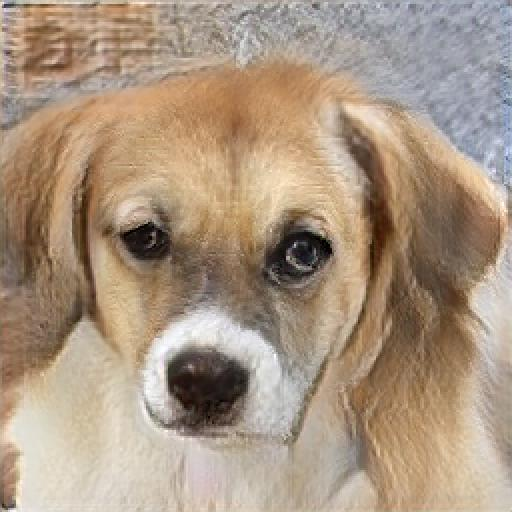} 
\tabularnewline

\includegraphics[width=0.157\linewidth]{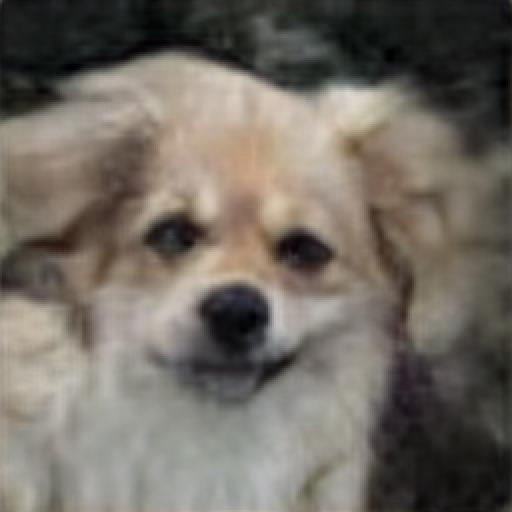} &
\includegraphics[width=0.157\linewidth]{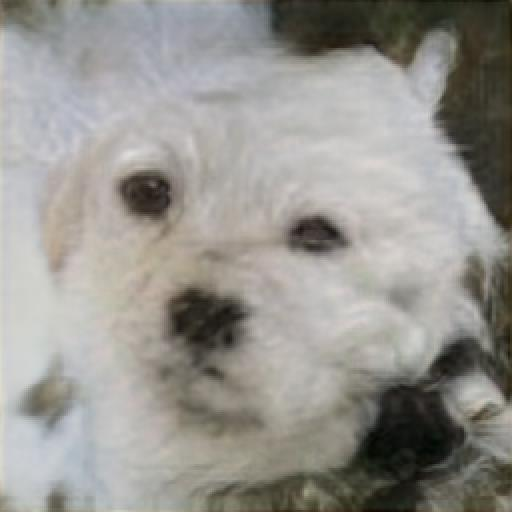} &
\includegraphics[width=0.157\linewidth]{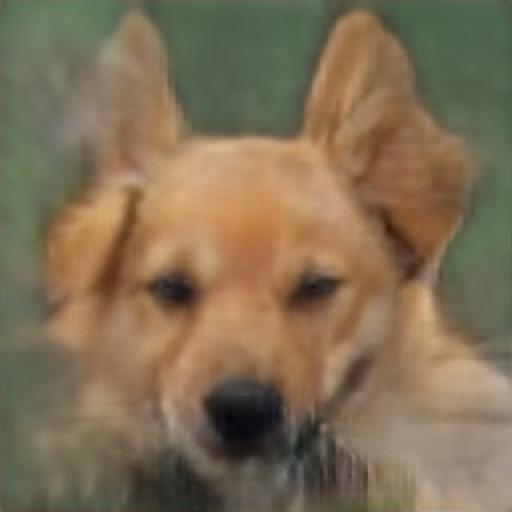} &
\includegraphics[width=0.157\linewidth]{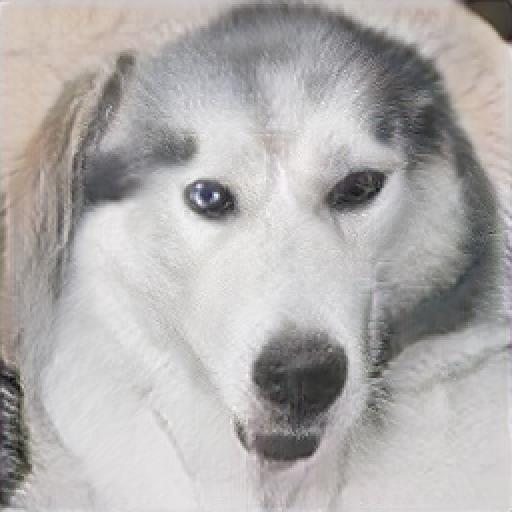} &
\includegraphics[width=0.157\linewidth]{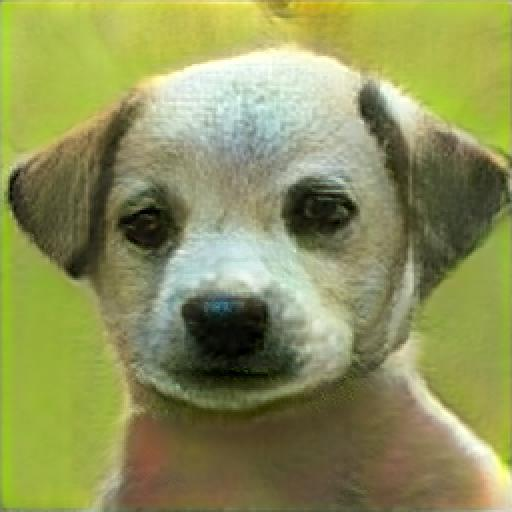} &
\includegraphics[width=0.157\linewidth]{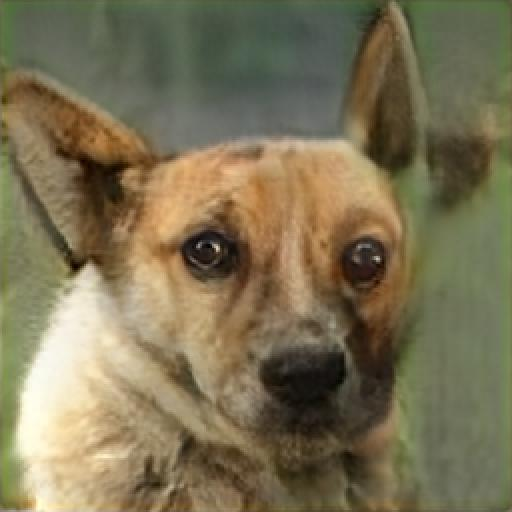} 
\tabularnewline
 
\includegraphics[width=0.157\linewidth]{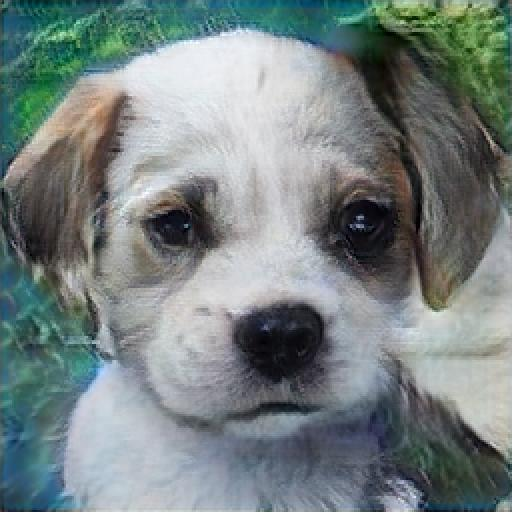} &
\includegraphics[width=0.157\linewidth]{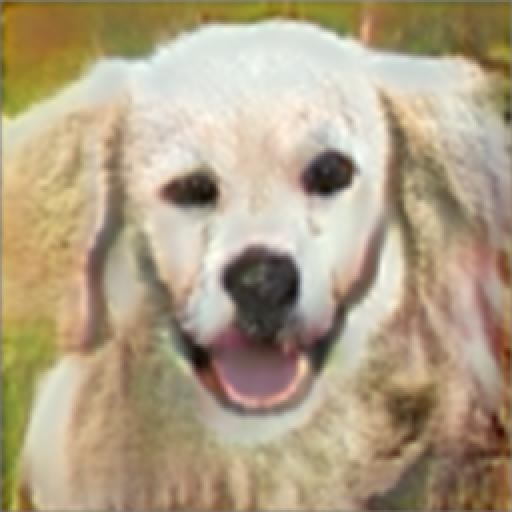} &
\includegraphics[width=0.157\linewidth]{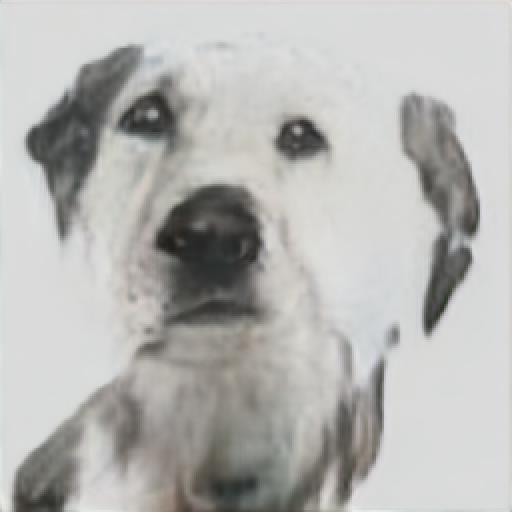} &
\includegraphics[width=0.157\linewidth]{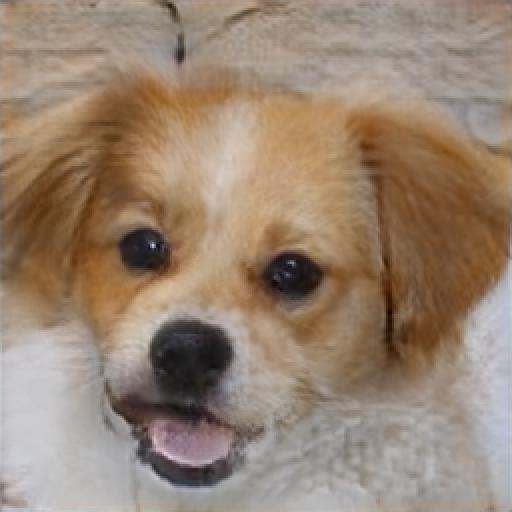} &
\includegraphics[width=0.157\linewidth]{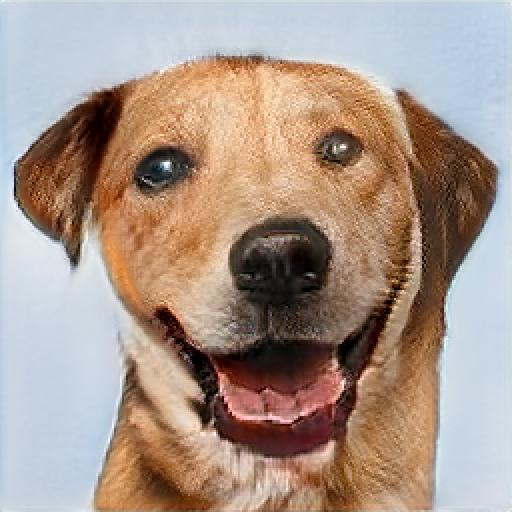} &
\includegraphics[width=0.157\linewidth]{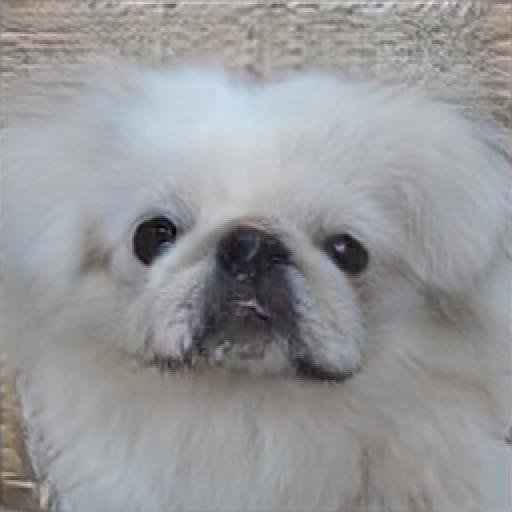} 

\tabularnewline
\tabularnewline

\multicolumn{3}{c}{FastGAN, trained on \textbf{25\% of data} (98 images)} &
\multicolumn{3}{c}{SIV-GAN+, trained on \textbf{25\% of data} (98 images)}
\tabularnewline

\includegraphics[width=0.157\linewidth]{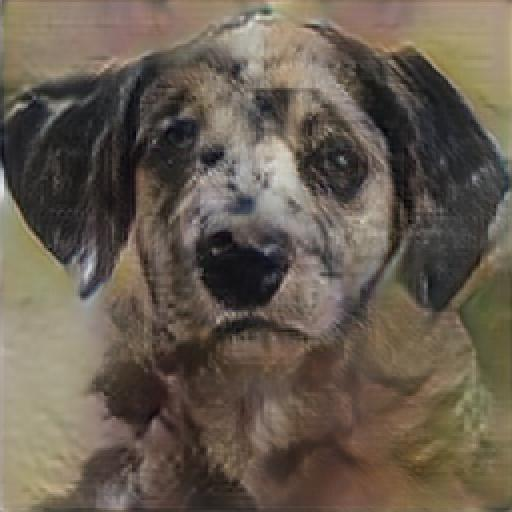} &
\includegraphics[width=0.157\linewidth]{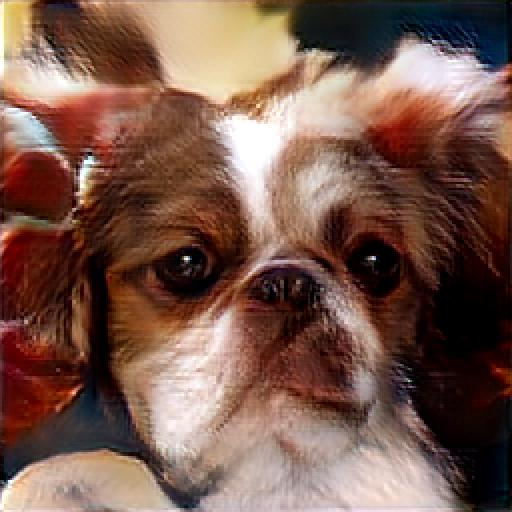} &
\includegraphics[width=0.157\linewidth]{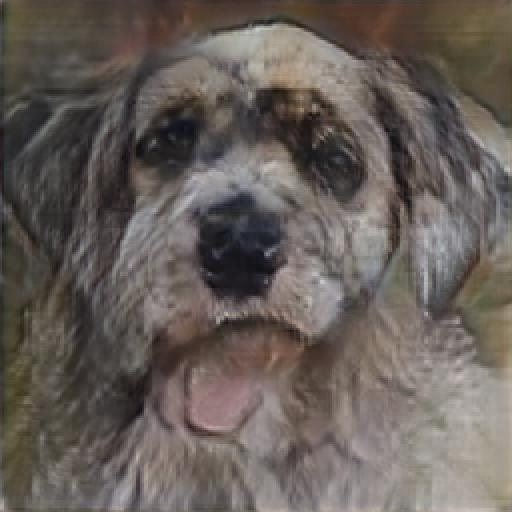} &
\includegraphics[width=0.157\linewidth]{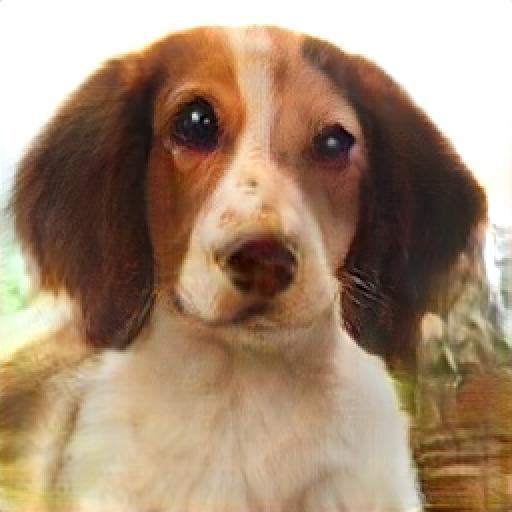} &
\includegraphics[width=0.157\linewidth]{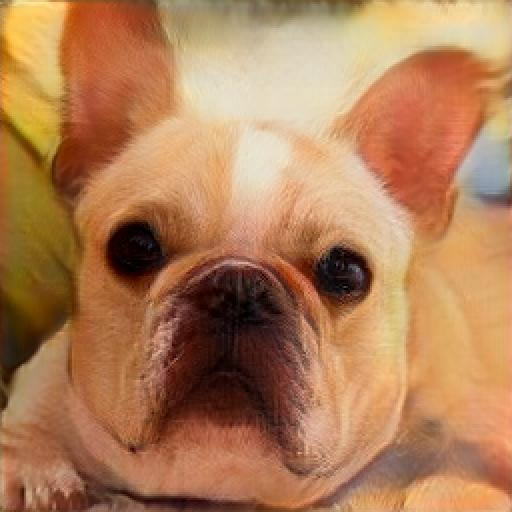} &
\includegraphics[width=0.157\linewidth]{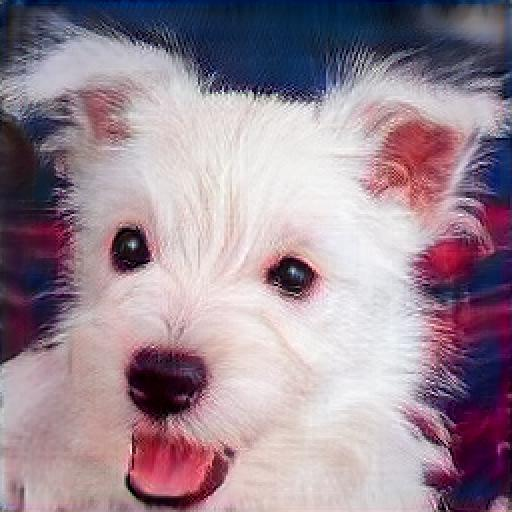} 
\tabularnewline

\includegraphics[width=0.157\linewidth]{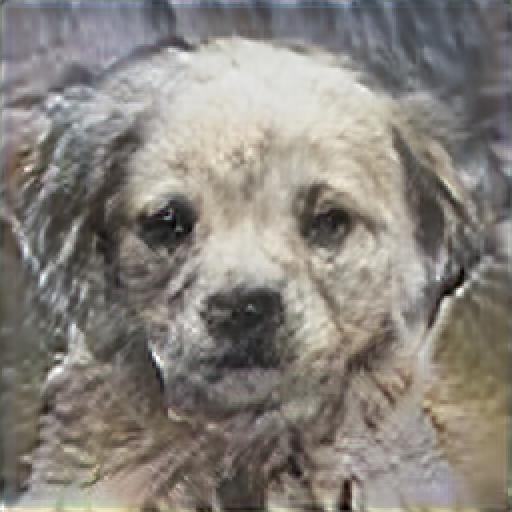} &
\includegraphics[width=0.157\linewidth]{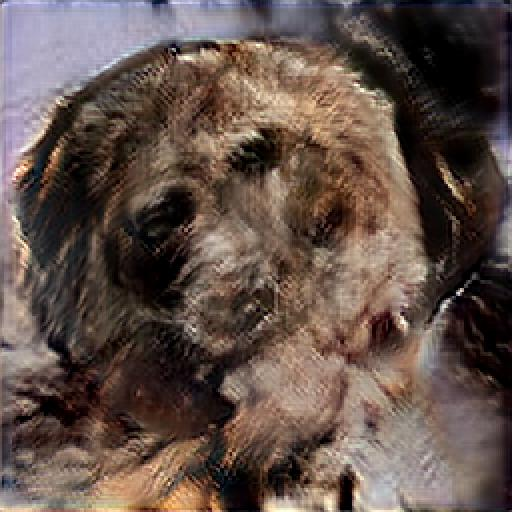} &
\includegraphics[width=0.157\linewidth]{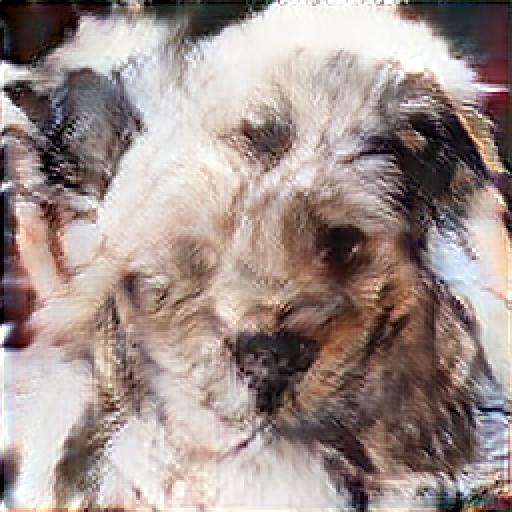} &
\includegraphics[width=0.157\linewidth]{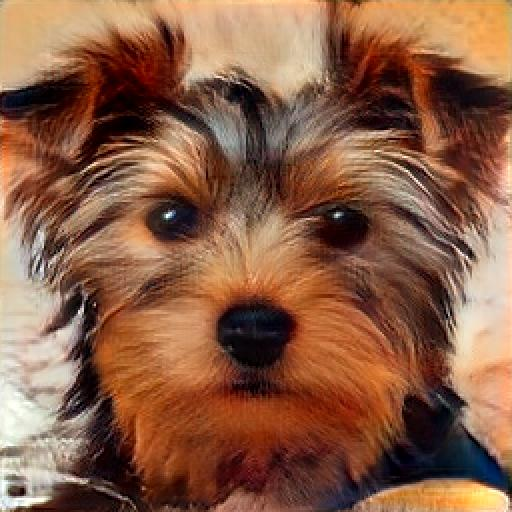} &
\includegraphics[width=0.157\linewidth]{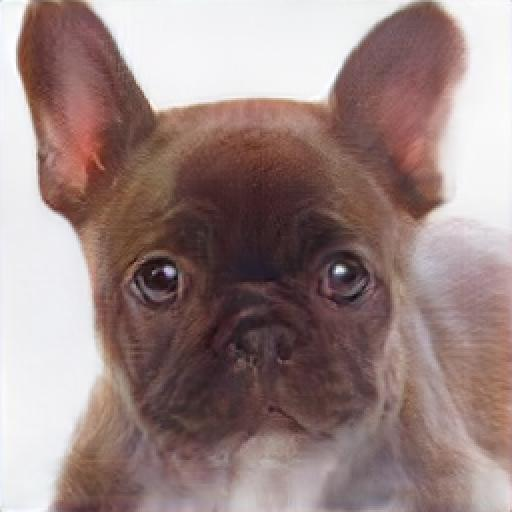} &
\includegraphics[width=0.157\linewidth]{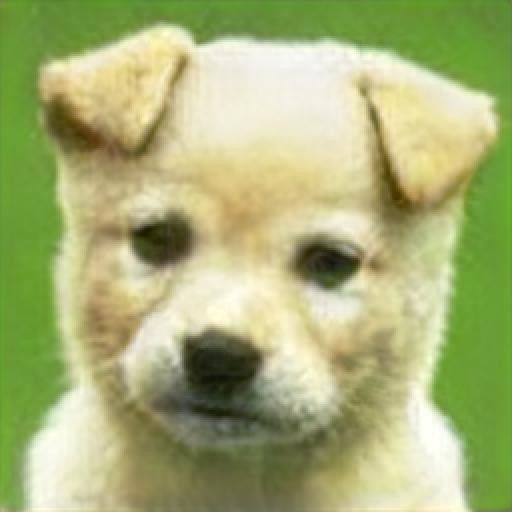} 
\tabularnewline

\includegraphics[width=0.157\linewidth]{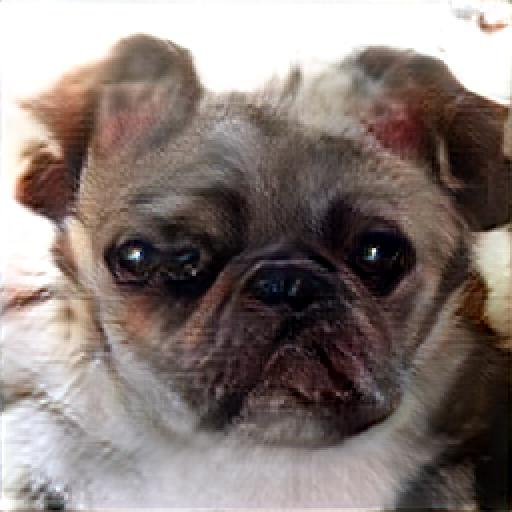} &
\includegraphics[width=0.157\linewidth]{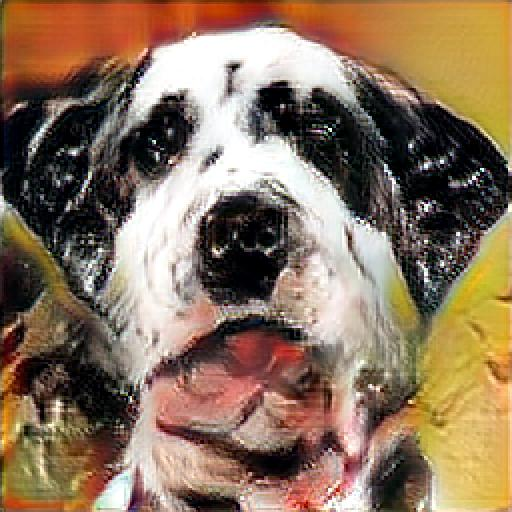} &
\includegraphics[width=0.157\linewidth]{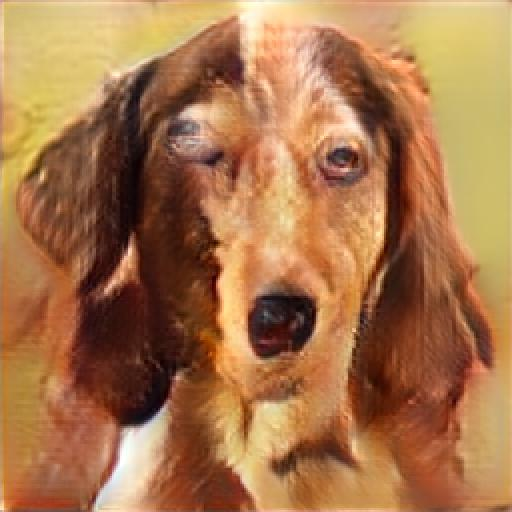} &
\includegraphics[width=0.157\linewidth]{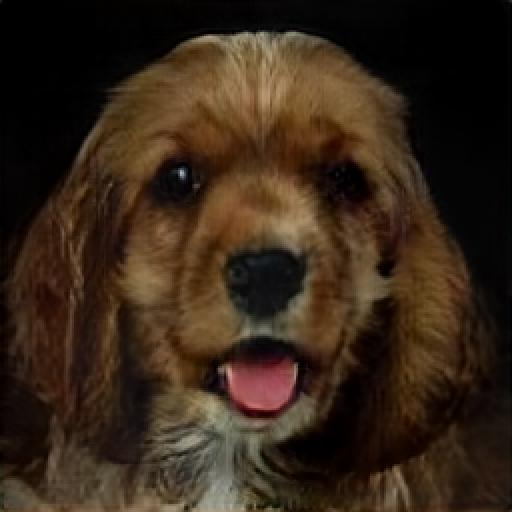} &
\includegraphics[width=0.157\linewidth]{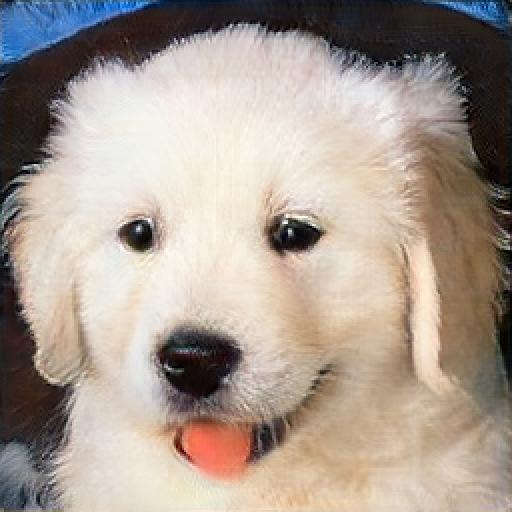} &
\includegraphics[width=0.157\linewidth]{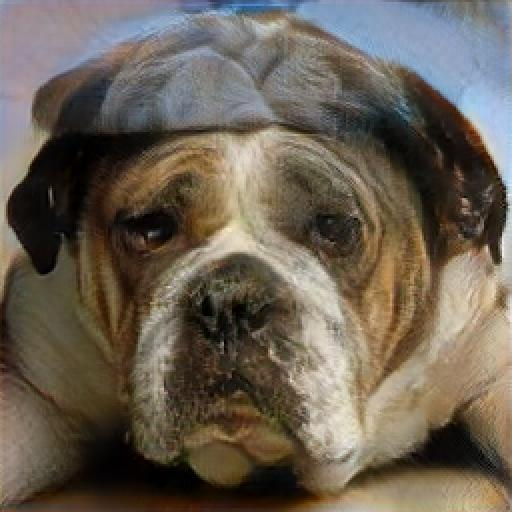}

\end{tabular}\hfill{}
\par\end{centering}
\caption{Visual results in the few-shot setting on the Face Dog dataset. The two upper blocks show generated images for the models trained on the full dataset (389 images), while the two bottom blocks show the results from training only using 25\% of data (98 images). SIV-GAN+ demonstrates not only superior performance on the standard few-shot setting, but also successfully deals with an extreme few-shot scenario (25\% of data), where FastGAN has a significant drop in performance.}
\label{fig:few-shot} 
\end{figure}

We train FastGAN and SIV-GAN+ for 100k iterations. We save the checkpoints every 10k iterations during training and report the best FID across all the checkpoints. The FID is computed between 5000 generated images and the whole reference dataset. The results are shown in Table \ref{table:few-shot}. We generally manage to reproduce the FID performance of FastGAN reported in \citep{anonymous2021towards}, obtaining slightly better results for all datasets. Table \ref{table:few-shot} shows that our SIV-GAN+ model outperforms FastGAN, achieving an average improvement of 8\% in FID across all datasets. Moreover, SIV-GAN+ also shows better results than the recent GAN model of \citet{tseng2021regularizing}, yielding the best FID on four out of five commonly used few-shot image synthesis datasets.
We show the visual comparison of our model with FastGAN in Fig. \ref{fig:few-shot} (two upper rows). Our model achieves a notably higher-quality synthesis on the Dog Face dataset, where FastGAN suffers from instabilities, having problems in generating good textures and correct shapes of dog faces.

%\anna{add 1 sentence about the results}

\subsection{Extremely low few-shot setting}
\label{sec:supp_fewshot_extreme}

\begin{table}
	\setlength{\tabcolsep}{0.044in}
	
	\centering
	\caption{Results in the extremely low few-shot data setting, where the models are trained only on subsets of standard few-shot datasets. Our model outperforms the baseline in all data regimes both in quality and diversity, and does not suffer from training instabilities even in extreme cases, such as using only 25\% of the training set. Collapsed runs with a high FID for Fast-GAN are shown in red.}
	\vspace{0.5em}
	
	\begin{tabular}{l|cc|cc|cc|cc|cc|cc}

	 \multirow{3}{*}{Method} & \multicolumn{6}{c|}{Panda (100)} & \multicolumn{6}{c}{Face Dog (389)}  \tabularnewline
	 
	 & \multicolumn{2}{c|}{100\%} & \multicolumn{2}{c|}{50\%} & \multicolumn{2}{c|}{25\%} &  \multicolumn{2}{c|}{100\%} & \multicolumn{2}{c|}{50\%} & \multicolumn{2}{c}{25\%}
	 \tabularnewline		
	 
	 & \small{FID} &  \small{LPIPS}  &  \small{FID} &  \small{LPIPS} & \small{FID} & \small{LPIPS} &  \small{FID} &  \small{LPIPS} &  \small{FID} & \small{LPIPS}  &  \small{FID} & \small{LPIPS} \tabularnewline
	
		\hline 	\hline 	
		
	FastGAN  & {9.63} & {0.48}   &  {13.97} &  {0.49} & \color{darkred} {16.08} & {0.47} & {53.39} &   {0.62} &  {77.57} &  {0.61} &  \color{darkred} {96.86} &  {0.61}  \tabularnewline

	SIV-GAN+  & \textbf{{9.22}} &  \textbf{{0.51}}  &  \textbf{{11.57}} &  \textbf{{0.51}} & \textbf{{9.58}} & \textbf{{0.50}} &  \textbf{{50.05}} &  \textbf{{0.63}} &  \textbf{{64.21}} &  \textbf{{0.62}} &  \textbf{{62.61}} &  \textbf{{0.62}} \tabularnewline

	\end{tabular}

	\label{table:few-shot_extreme} %
\end{table}

Training GANs in low data regimes is challenging, because a GAN discriminator is prone to overfitting and memorization effects, which can result in the divergence of the training progress. Existing state-of-the-art few-shot models \citep{tseng2021regularizing, anonymous2021towards} were demonstrated to succeed in this task on datasets containing at least 100 images (see App.~\ref{sec:supp_fewshot_standard}). In this section, we investigate more extreme scenarios with datasets consisting of less than 100 images. We construct  ``extremely low'' few-shot learning regimes by selecting subsets of Obama and Face-Dog datasets containing only 50\% and 25\% of original training images. 

The quantitative results for the extremely low few-shot settings are shown in Table \ref{table:few-shot_extreme}, while the visual results on 25\%-subsets is shown in Fig. \ref{fig:few-shot} (two bottom rows). As seen from the figure, the FastGAN model experiences a drop in performance in the more extreme data setting, when using less than 100 images for training, producing unrealistic textures or incoherent shapes of dog faces. In Table \ref{table:few-shot_extreme} this effect is reflected in high FID scores (highlighted in red). In contrast, SIV-GAN+ shows good image quality uniformly across settings, reaching good FID even on training sets containing very few images. Importantly, the gain in FID is not achieved at the cost of diversity: our model has a higher LPIPS diversity score in all data regimes compared to the baseline. Moreover, Table \ref{table:few-shot_extreme} shows similar diversity scores for SIV-GAN+ in various settings, indicating that our model can be successfully scaled to various extremely low-data regimes maintaining similar levels of synthesis diversity. Overall, the results demonstrate that our proposed two-branch discriminator helps to mitigate discriminator overfitting in few-shot regimes, stabilizing the training, and thus helping to maintain good quality and diversity even when the model is trained on datasets with very few images.

\subsection{Non-object-centric few-shot image synthesis}
\label{sec:supp_fewshot_outdoor}

As mentioned in App. \ref{sec:supp_fewshot_standard}, standard few-shot image synthesis benchmarks include only object-centric datasets, such as centred faces of people or animals. Such datasets have very limited variability in layouts, having very similar locations of face parts in all images. In this section, we explore few-shot image synthesis on datasets with more complex structures. For this, we construct subsets of the ADE-Outdoors \citep{zhou2017scene} and LSUN-Church \citep{yu15lsun} datasets, consisting of 100 images with resolution 256x256. Such datasets form a more difficult task, because the models have to learn how to combine objects with different semantics from different images preserving the global scene layout. 

\begin{figure}[t]
\begin{centering}
\setlength{\tabcolsep}{0.1em}

\par\end{centering}
\begin{centering}

\hfill{}%
\begin{tabular}{cc@{\hskip 0.15in}cc}

SIV-GAN+ & Nearest  & SIV-GAN+  & Nearest  
\tabularnewline
generated images & training frames & generated images & training frames
\tabularnewline

\includegraphics[width=0.28\linewidth]{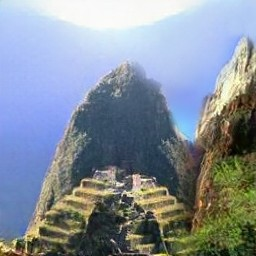} &
\includegraphics[width=0.138\linewidth]{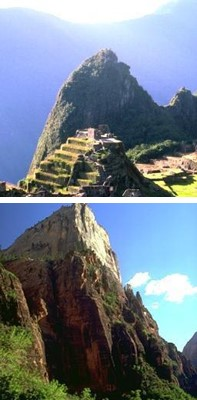} &

\includegraphics[width=0.28\linewidth]{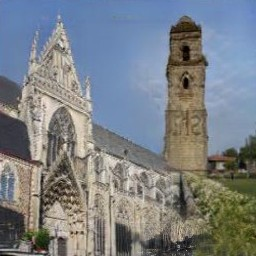} &
\includegraphics[width=0.138\linewidth]{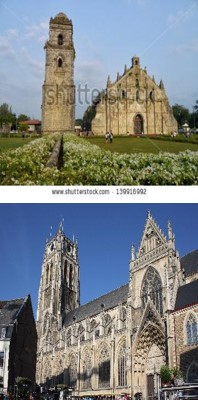} 
\tabularnewline

%\includegraphics[width=0.28\linewidth]{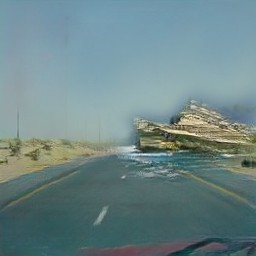} &
%\includegraphics[width=0.138\linewidth]{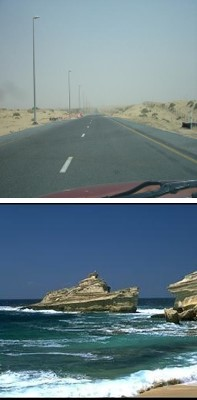} &

%\includegraphics[width=0.28\linewidth]{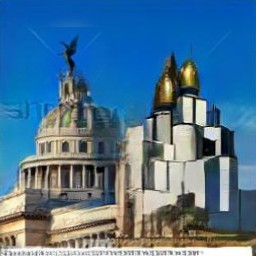} &
%\includegraphics[width=0.138\linewidth]{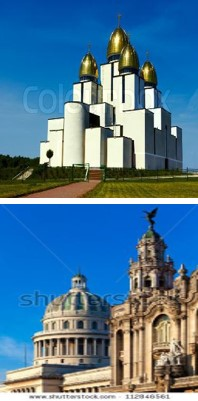} 
%\tabularnewline

\tabularnewline 

\multicolumn{4}{c}{SIV-GAN+ generated images}
\tabularnewline
\multicolumn{4}{c}{
	
	~\includegraphics[width=0.14\linewidth]{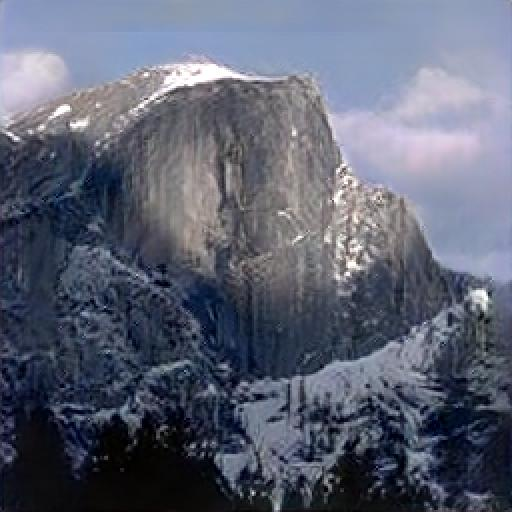}~
	\includegraphics[width=0.14\linewidth]{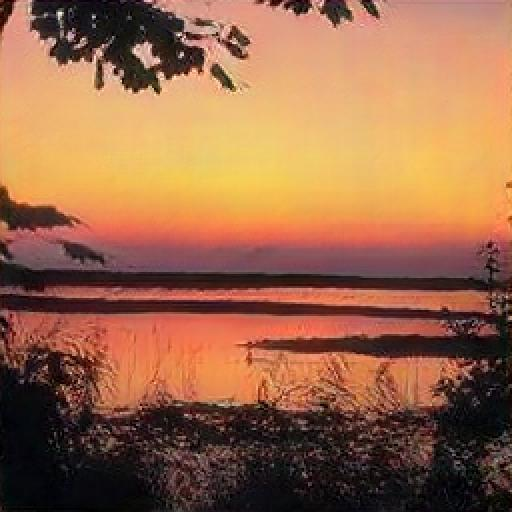}~
	\includegraphics[width=0.14\linewidth]{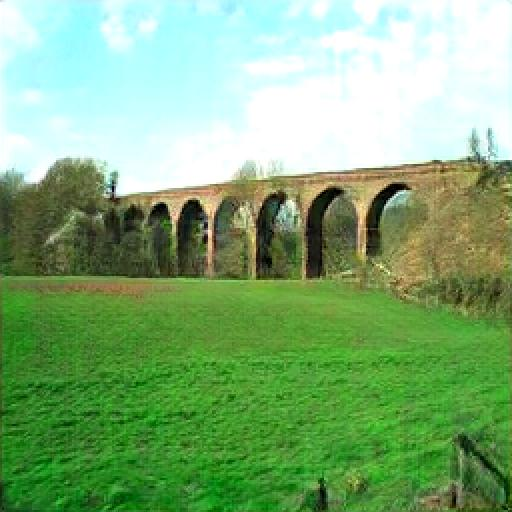}~~
	\includegraphics[width=0.14\linewidth]{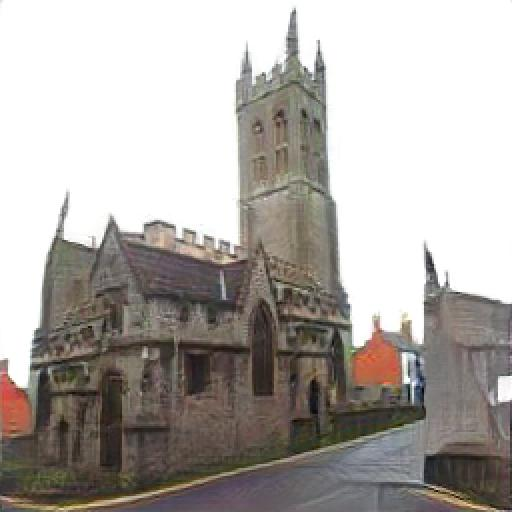}~
	\includegraphics[width=0.14\linewidth]{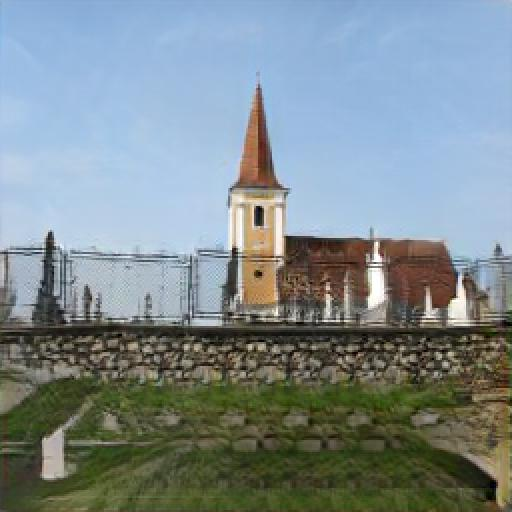}~
	\includegraphics[width=0.14\linewidth]{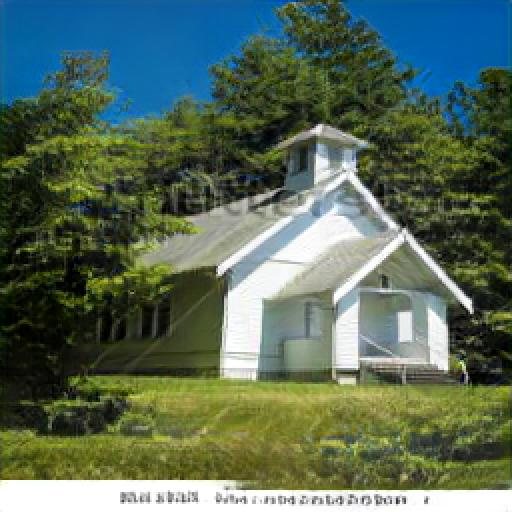}~~
} \tabularnewline \tabularnewline

\multicolumn{4}{c}{FastGAN generated images}
\tabularnewline
\multicolumn{4}{c}{
	
	~\includegraphics[width=0.14\linewidth]{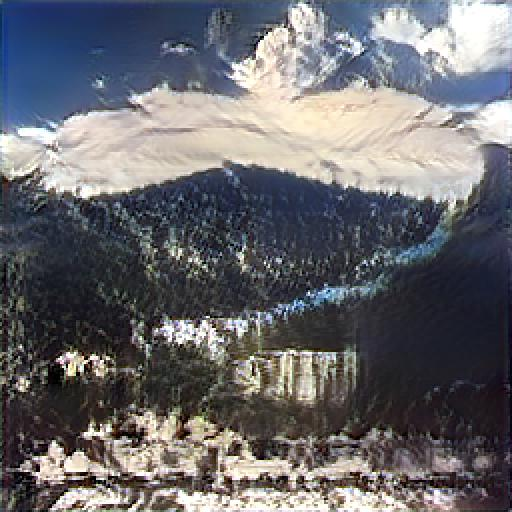}~
	\includegraphics[width=0.14\linewidth]{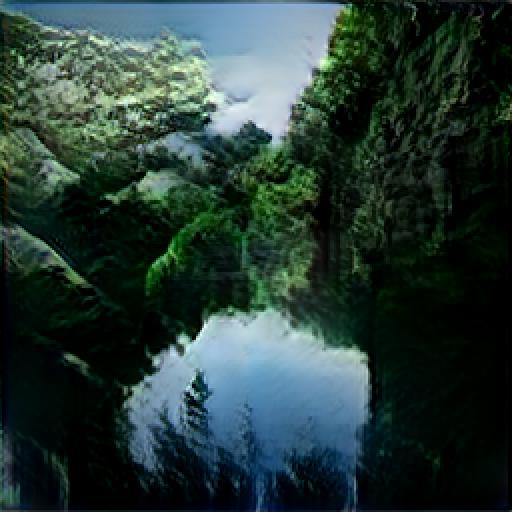}~
	\includegraphics[width=0.14\linewidth]{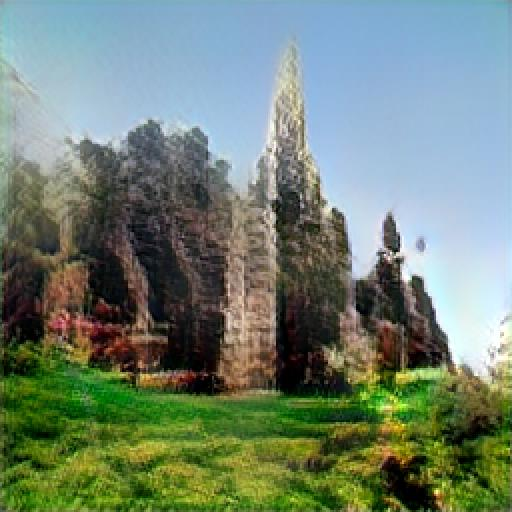}~~
	\includegraphics[width=0.14\linewidth]{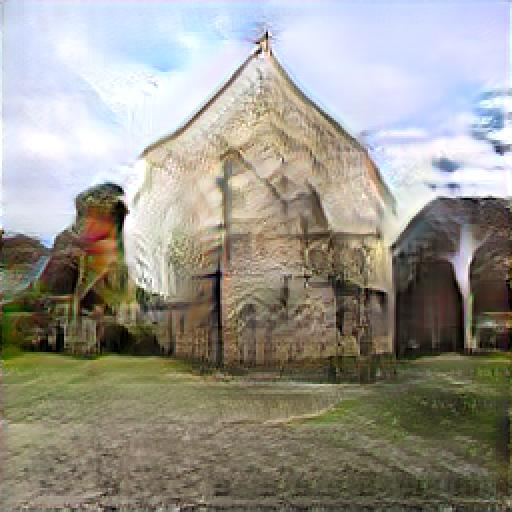}~
	\includegraphics[width=0.14\linewidth]{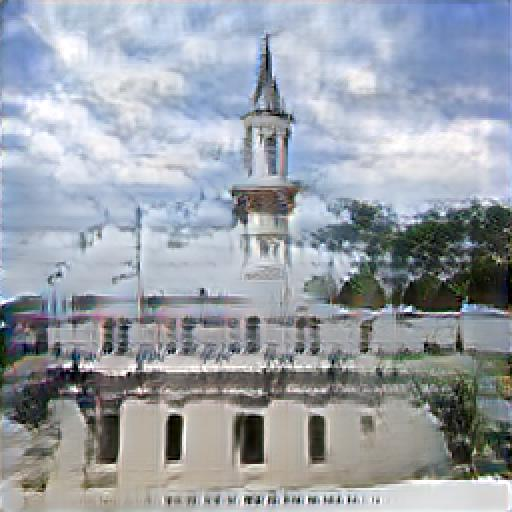}~
	\includegraphics[width=0.14\linewidth]{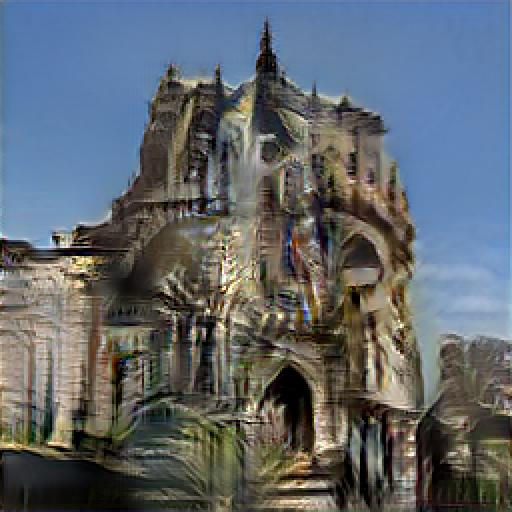}~~
}

\end{tabular}\hfill{}
\par\end{centering}
\caption{Visual examples in the few-shot setting on the ADE-Outdoors and LSUN Church datasets. Despite being trained only on 100 images, SIV-GAN+ does not suffer from memorization issues and achieves an astonishing capability to combine objects from different training images, preserving the global coherency of scenes. In contrast, FastGAN does not achieve high-quality synthesis, struggling to generate coherent images with fine textures.}
%Next to each generated example, two perceptually closest images from the training set are shown.
\label{fig:few-shot_outdoor} 
\end{figure}
\begin{table}[t]
	\setlength{\tabcolsep}{0.038in}

	\centering
	
	\caption{Results on few-shot datasets with a non-object-centric structure. Our model outperforms FastGAN both in quality and diversity on both datasets.}
	\vspace{0.5em}
	
	\begin{tabular}{l|cc|cc|cc|cc|cc|cc}

	\multirow{3}{*}{Method} & \multicolumn{6}{c|}{ADE-Outdoor (100)} & \multicolumn{6}{c}{LSUN Church (100)}  \tabularnewline
	
	& \multicolumn{2}{c|}{100\%} & \multicolumn{2}{c|}{50\%} & \multicolumn{2}{c|}{25\%} &  \multicolumn{2}{c|}{100\%} & \multicolumn{2}{c|}{50\%} & \multicolumn{2}{c}{25\%}
	\tabularnewline		
	
	& \small{FID} &  \small{LPIPS}  &  \small{FID} &  \small{LPIPS} & \small{FID} & \small{LPIPS} &  \small{FID} &  \small{LPIPS} &  \small{FID} & \small{LPIPS}  &  \small{FID} & \small{LPIPS} \tabularnewline
	
	\hline 	\hline 	
	
	FastGAN  & {113.2} & {0.62}   &  {125.1} &  {0.62} & {98.28} & {0.61} & {90.65} &   {0.58} &  {121.4} &  {0.58} &   {114.1} &  {0.56}  \tabularnewline

	SIV-GAN+  & \textbf{{88.46}} &  \textbf{{0.64}}  &  \textbf{{82.89}} &  \textbf{{0.63}} & \textbf{{52.96}} & \textbf{{0.63}} &  \textbf{{85.01}} &  \textbf{{0.60}} &  \textbf{{103.8}} &  \textbf{{0.60}} &  \textbf{{90.10}} &  \textbf{{0.59}} \tabularnewline
		
	\end{tabular}

	\label{table:few-shot_outdoor} %
\end{table}

The quantitative comparison between SIV-GAN+ and FastGAN is shown in Table~\ref{table:few-shot_outdoor}. Our model outperforms FastGAN in different data regimes (100, 50, 25 images) in both quality and diversity. Notably, the structure of the ADE-Outdoors and LSUN-Church datasets provides potential to generate novel compositions of objects which were not seen in the training data. We show examples of interesting scene compositions produced by our model in Fig. \ref{fig:few-shot_outdoor}). Being trained only on 100 images of outdoor landscapes or churches, SIV-GAN+ does not memorize the training examples, generating novel compositions of mountains or exchanging towers of different churches. In the meantime, FastGAN suffers from instabilities in this setting, struggling to generate images with fine textures.
