# Supplementary material for: Generating Novel Scene Compositions from Single Images and Videos
Source: arXiv:2103.13389 source file (2023-12-13)
Supplement: Supplementary file 7 [file con_lay_embeddings.tex]

\begin{figure}[t]
	%\vspace{-1.5em}
	%\hfill{}%
	\begin{tabular}{@{}c@{\hskip 0.005in}c@{}}	
		\includegraphics[width=0.99\linewidth]{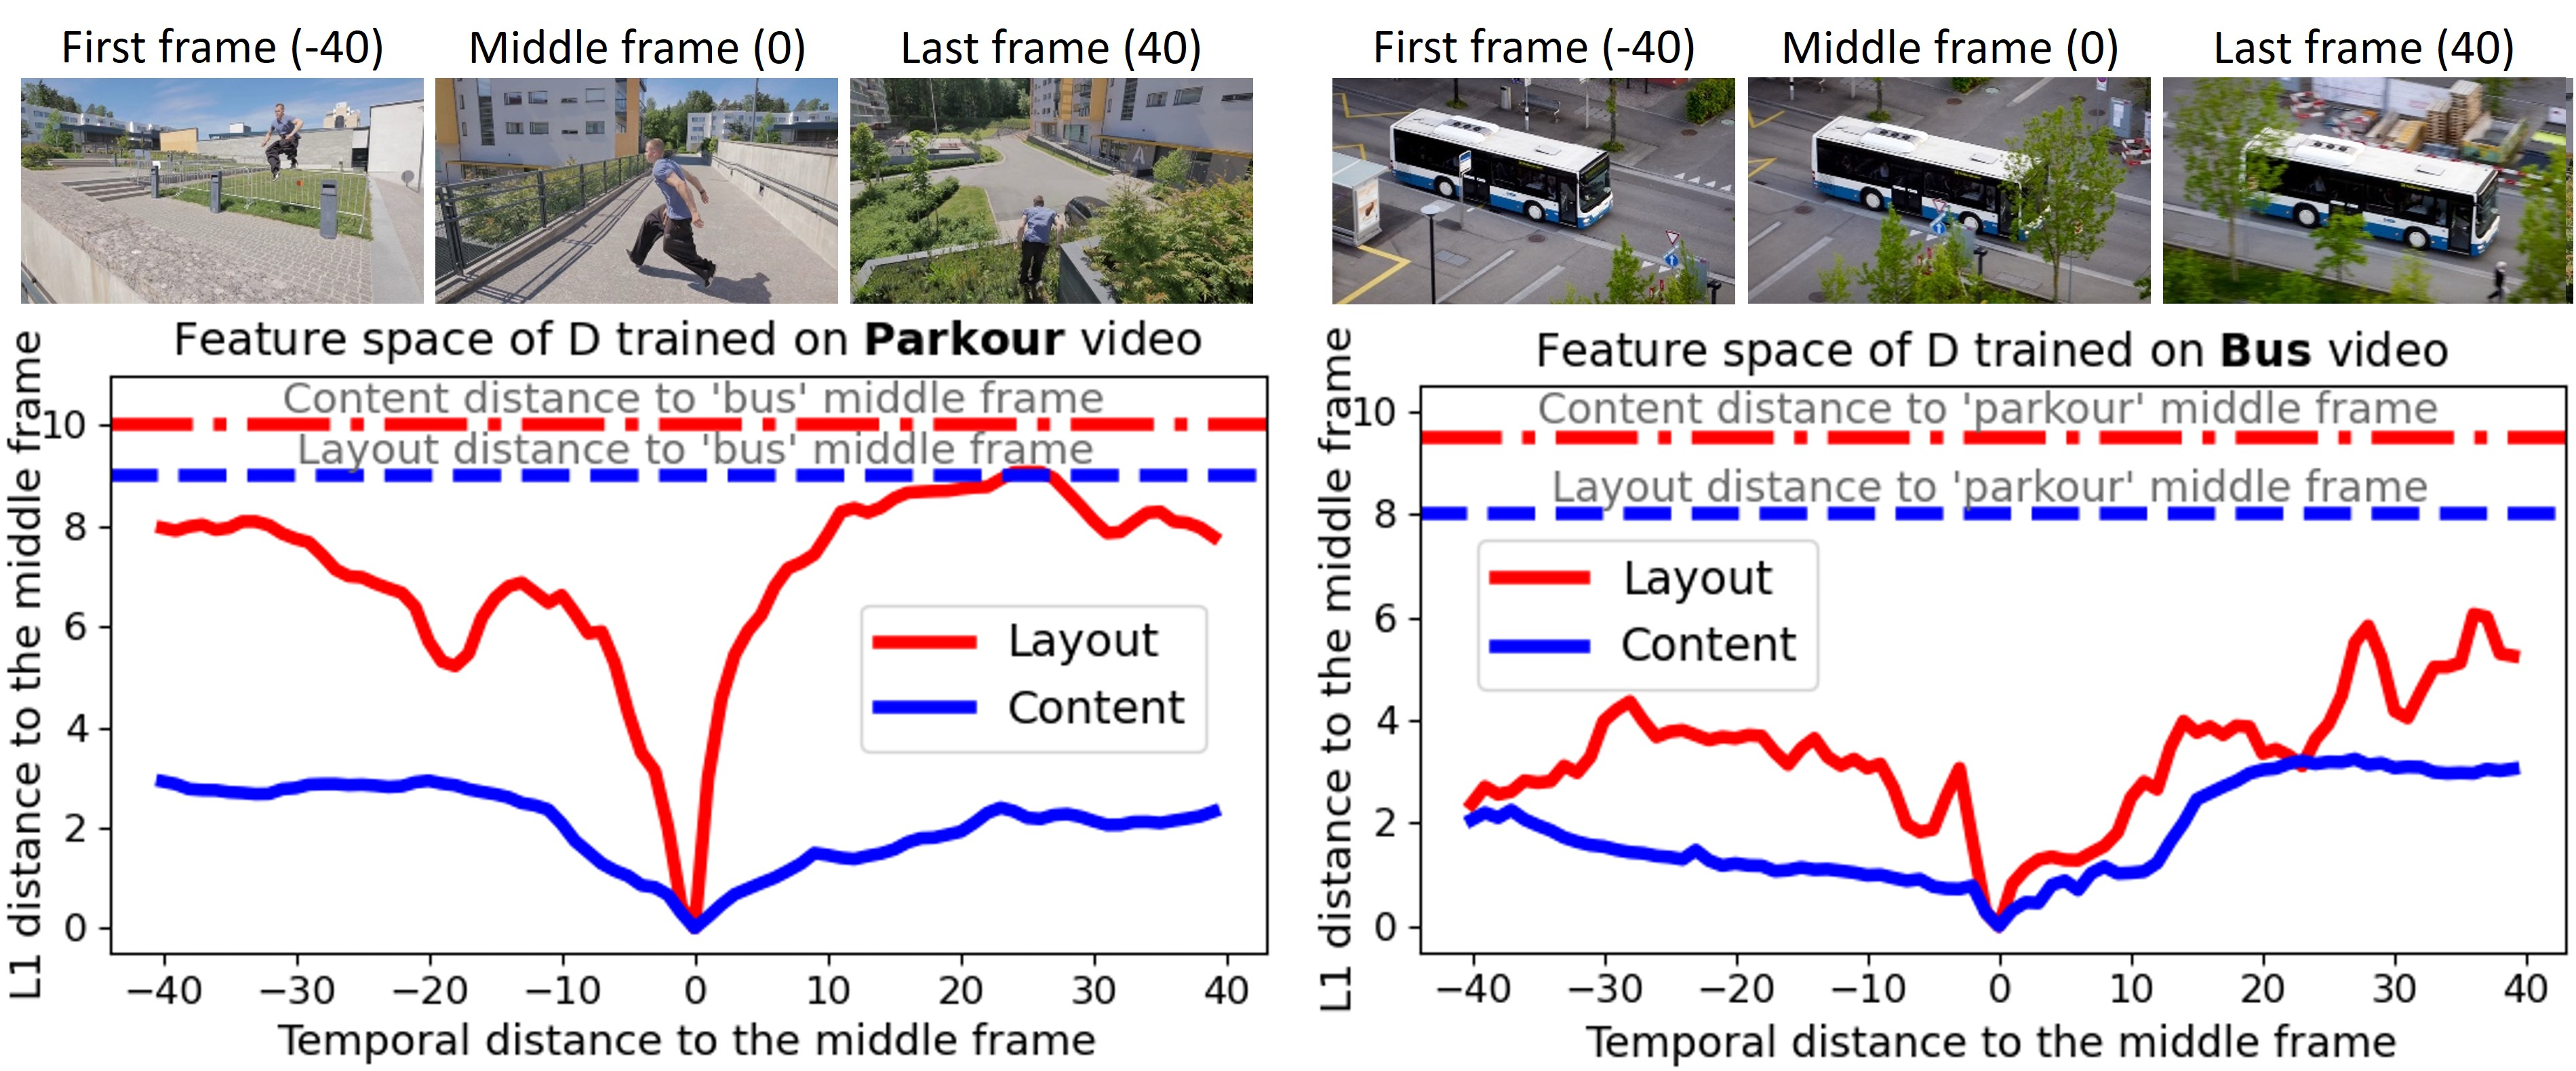} 
	\end{tabular}
	\vspace{-0.8ex}
	\caption{\label{fig:con_lay_embeddings} Feature distances from video frames to middle frame. The layout embedding distances (solid red) between “bus” frames are lower than for the “parkour” video. The content embedding distances between frames of the same sequence (solid blue) are significantly lower than the distance between middle frames of different videos (dashed blue).}
	\vspace{-1.7em}
\end{figure}
