# Supplementary material for: Generating Novel Scene Compositions from Single Images and Videos
Source: arXiv:2103.13389 source file (2023-12-13)
Supplement: Supplementary file 8 [file few-shot.tex]

\begin{figure}[t]
\begin{centering}
\setlength{\tabcolsep}{0.1em}

\par\end{centering}
\begin{centering}

\hfill{}%
\begin{tabular}{l@{\hskip 0.05in}l@{\hskip 0.05in}l@{\hskip 0.12in}l@{\hskip 0.05in}l@{\hskip 0.05in}l}
	
\multicolumn{3}{c}{FastGAN, trained on \textbf{full dataset} (389 images)} &
\multicolumn{3}{c}{SIV-GAN+, trained on \textbf{full dataset} (389 images)}
\tabularnewline
 
\includegraphics[width=0.157\linewidth]{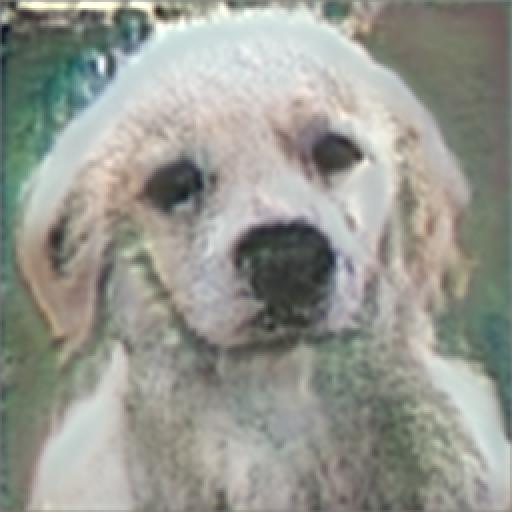} &
\includegraphics[width=0.157\linewidth]{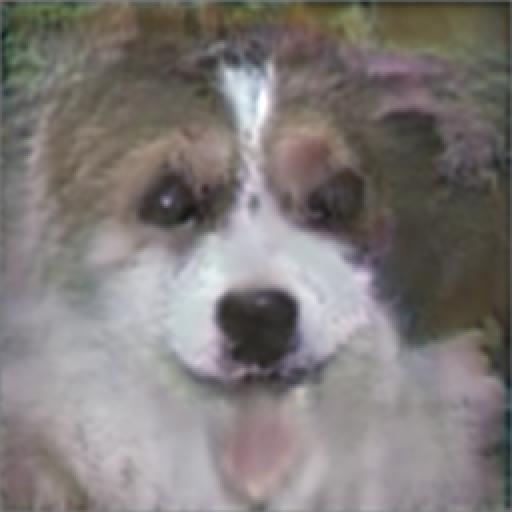} &
\includegraphics[width=0.157\linewidth]{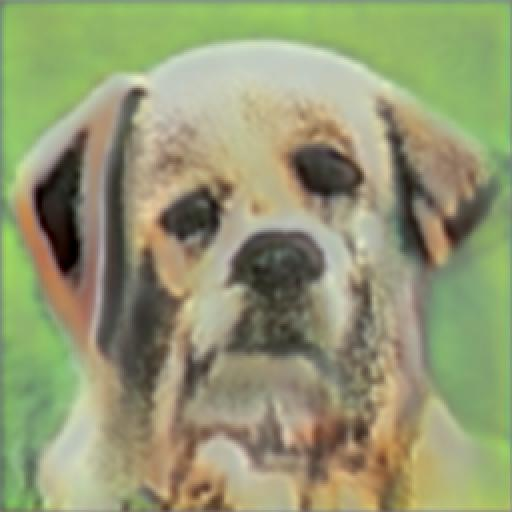} &
\includegraphics[width=0.157\linewidth]{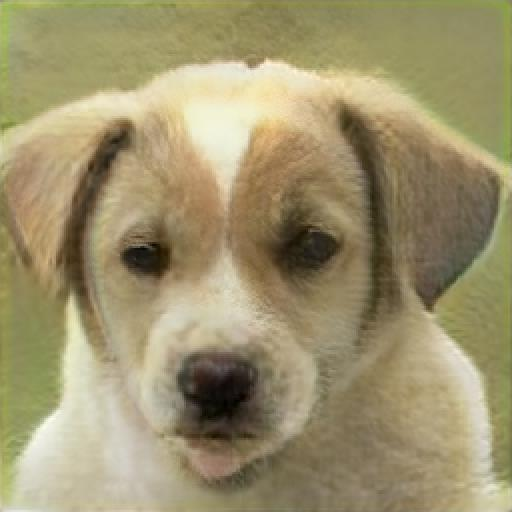} &
\includegraphics[width=0.157\linewidth]{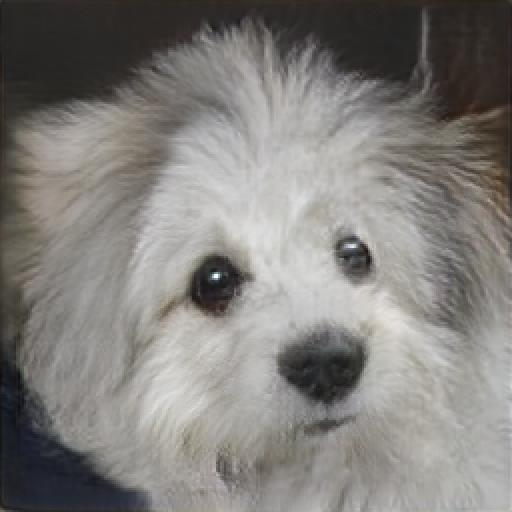} &
\includegraphics[width=0.157\linewidth]{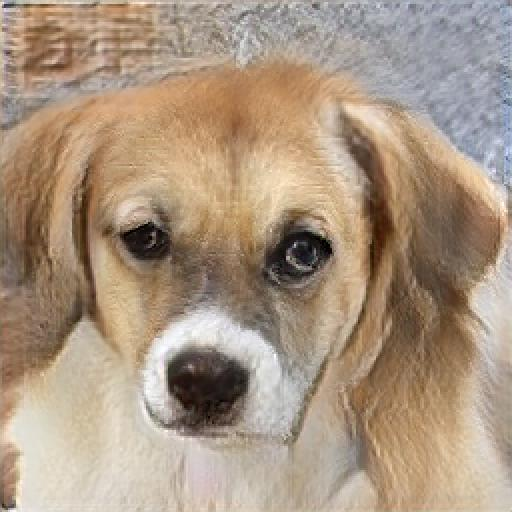} 
\tabularnewline

\includegraphics[width=0.157\linewidth]{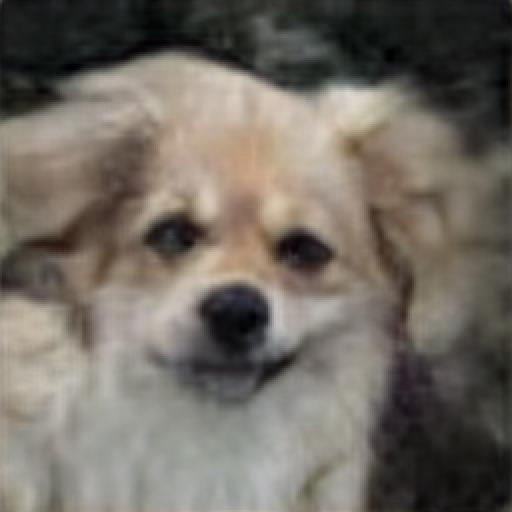} &
\includegraphics[width=0.157\linewidth]{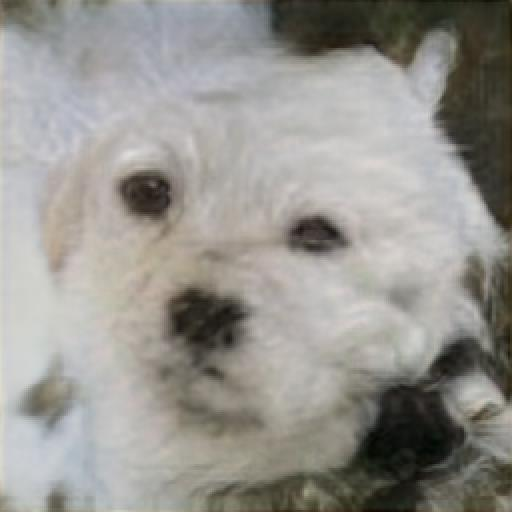} &
\includegraphics[width=0.157\linewidth]{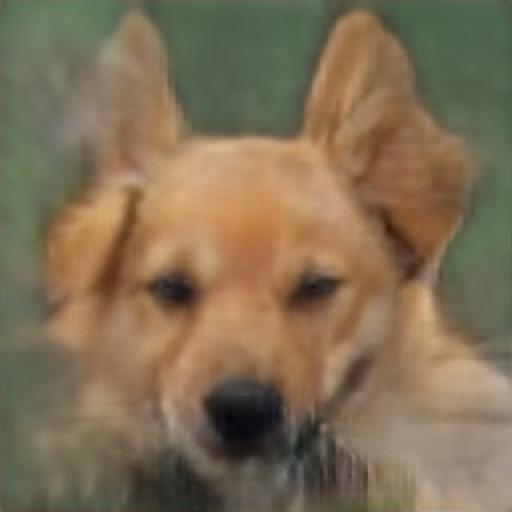} &
\includegraphics[width=0.157\linewidth]{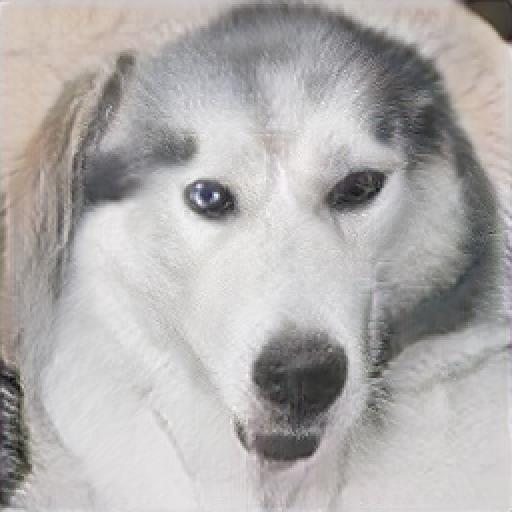} &
\includegraphics[width=0.157\linewidth]{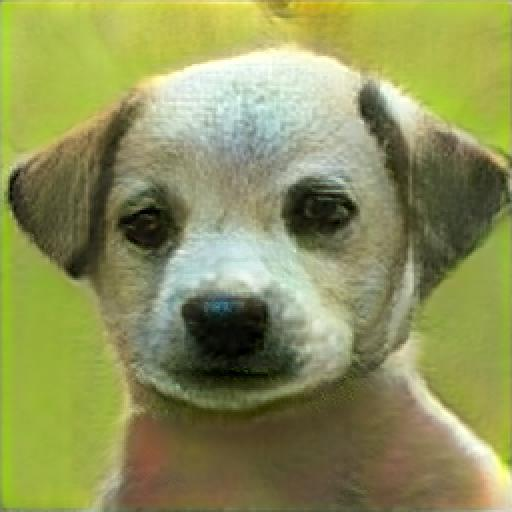} &
\includegraphics[width=0.157\linewidth]{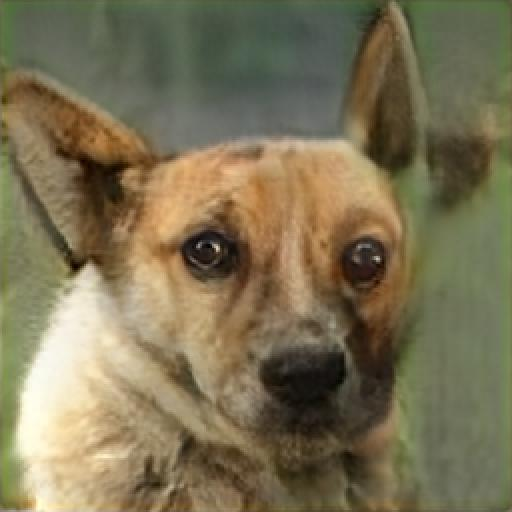} 
\tabularnewline
 
\includegraphics[width=0.157\linewidth]{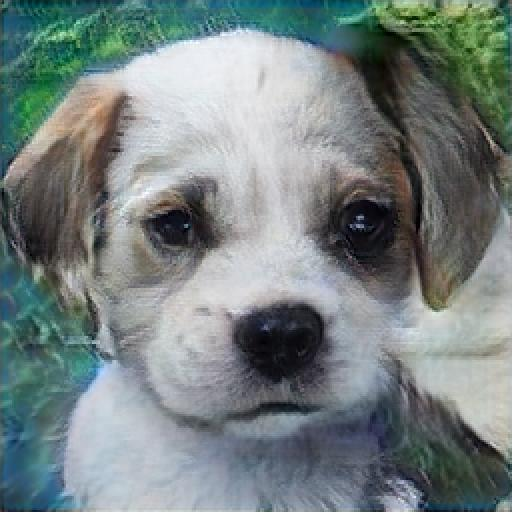} &
\includegraphics[width=0.157\linewidth]{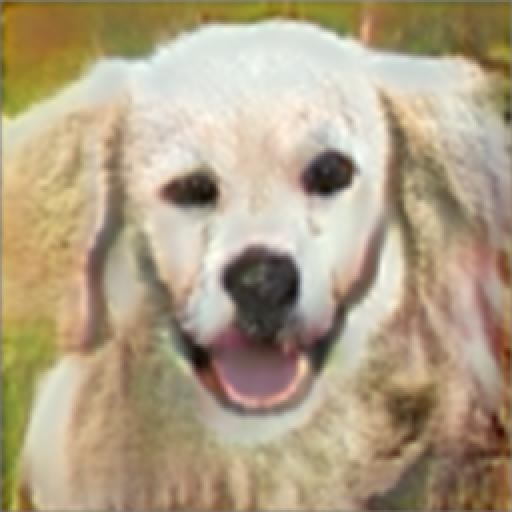} &
\includegraphics[width=0.157\linewidth]{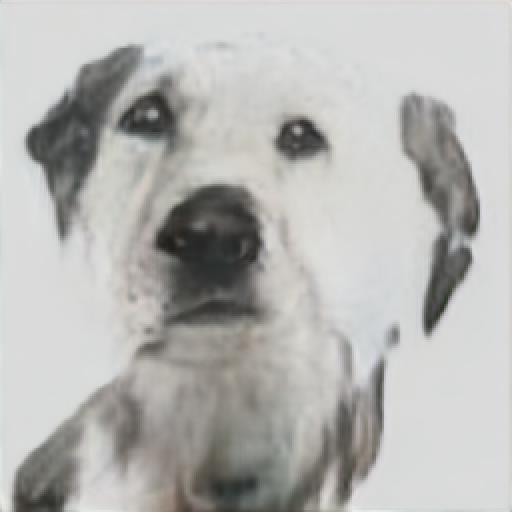} &
\includegraphics[width=0.157\linewidth]{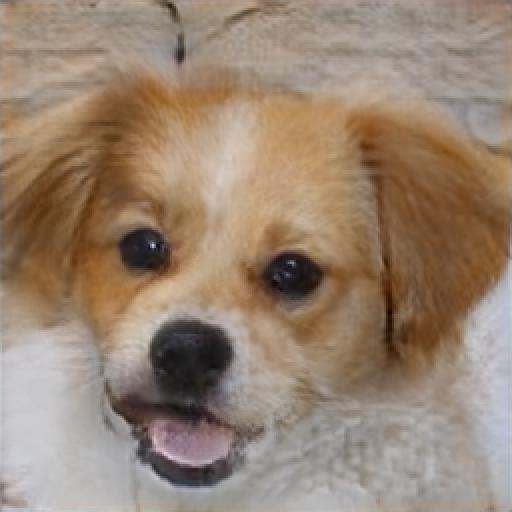} &
\includegraphics[width=0.157\linewidth]{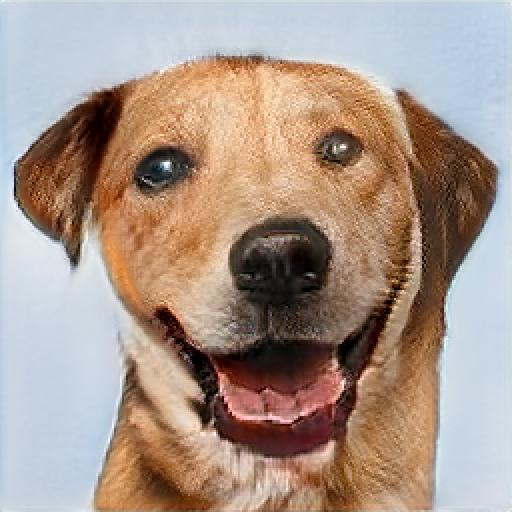} &
\includegraphics[width=0.157\linewidth]{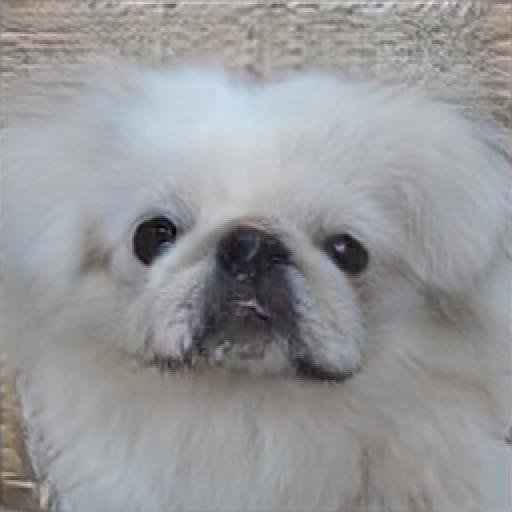} 

\tabularnewline
\tabularnewline

\multicolumn{3}{c}{FastGAN, trained on \textbf{25\% of data} (98 images)} &
\multicolumn{3}{c}{SIV-GAN+, trained on \textbf{25\% of data} (98 images)}
\tabularnewline

\includegraphics[width=0.157\linewidth]{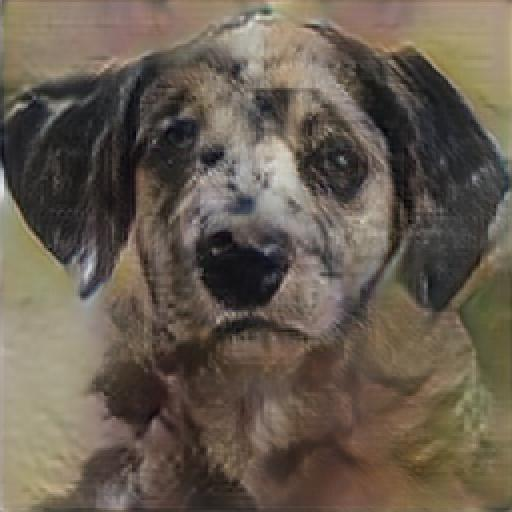} &
\includegraphics[width=0.157\linewidth]{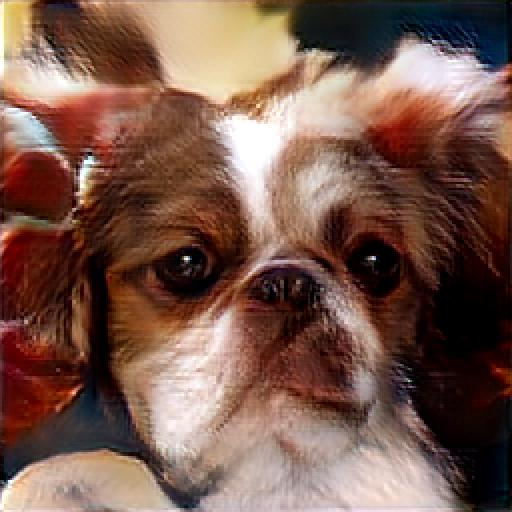} &
\includegraphics[width=0.157\linewidth]{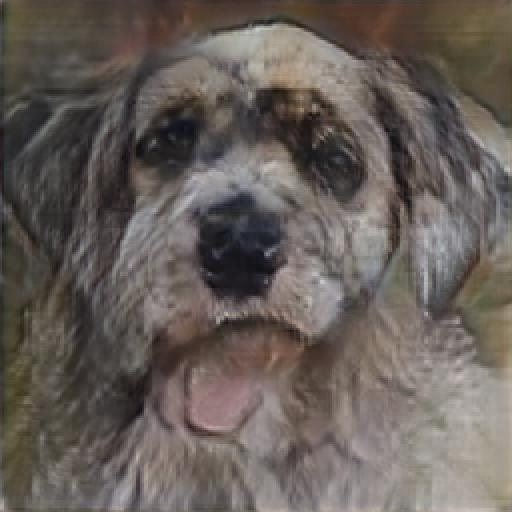} &
\includegraphics[width=0.157\linewidth]{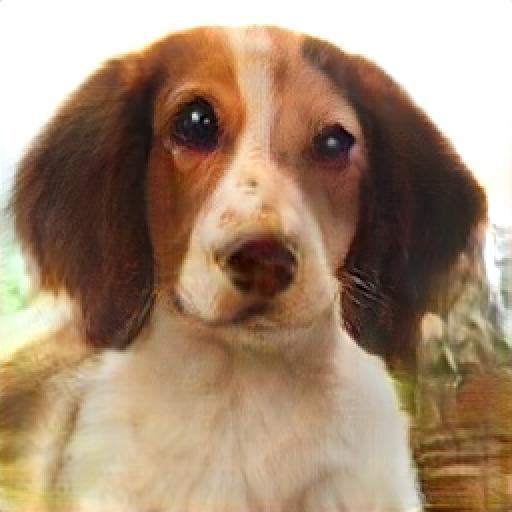} &
\includegraphics[width=0.157\linewidth]{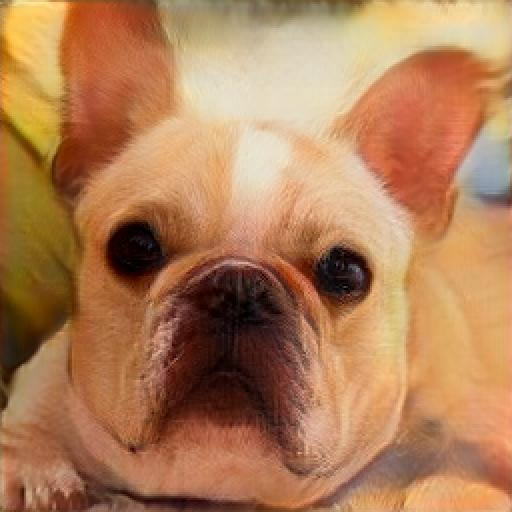} &
\includegraphics[width=0.157\linewidth]{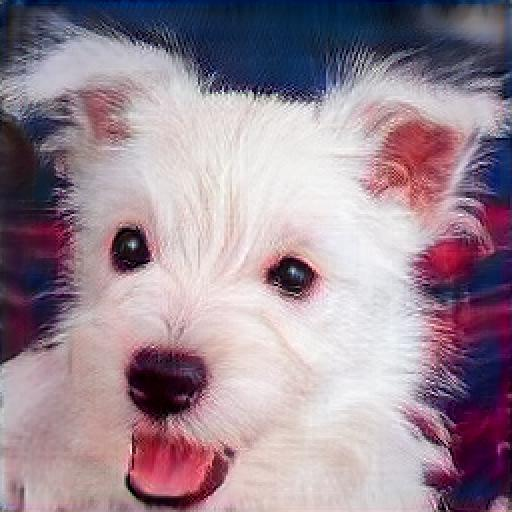} 
\tabularnewline

\includegraphics[width=0.157\linewidth]{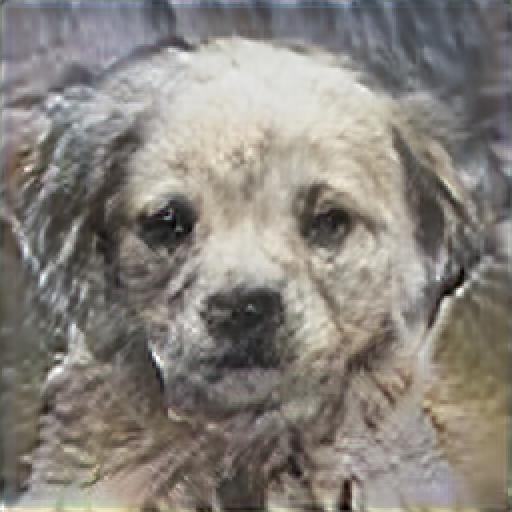} &
\includegraphics[width=0.157\linewidth]{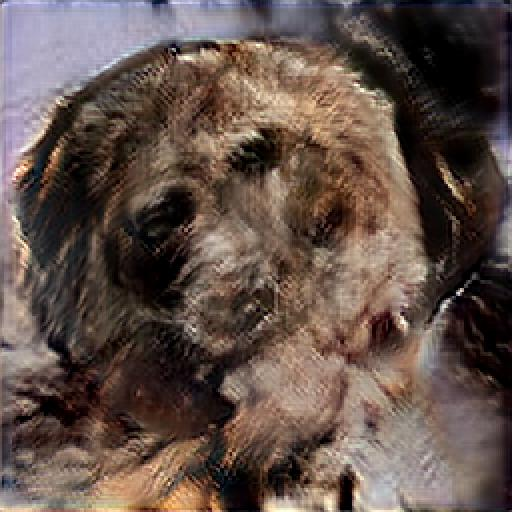} &
\includegraphics[width=0.157\linewidth]{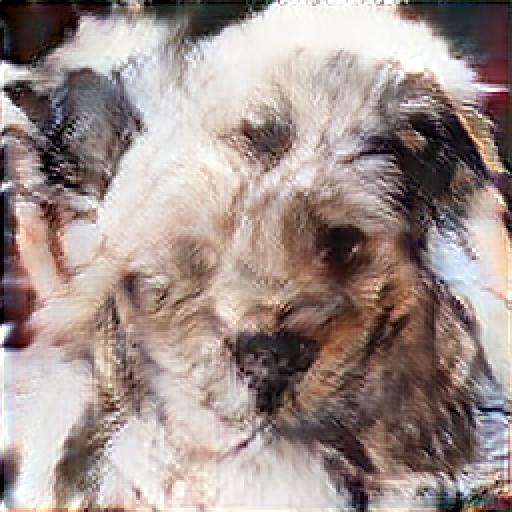} &
\includegraphics[width=0.157\linewidth]{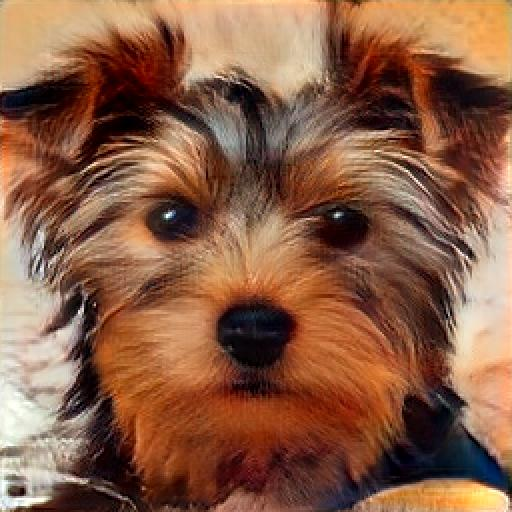} &
\includegraphics[width=0.157\linewidth]{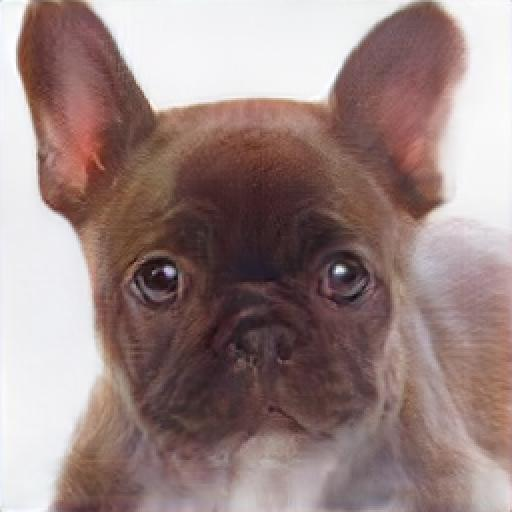} &
\includegraphics[width=0.157\linewidth]{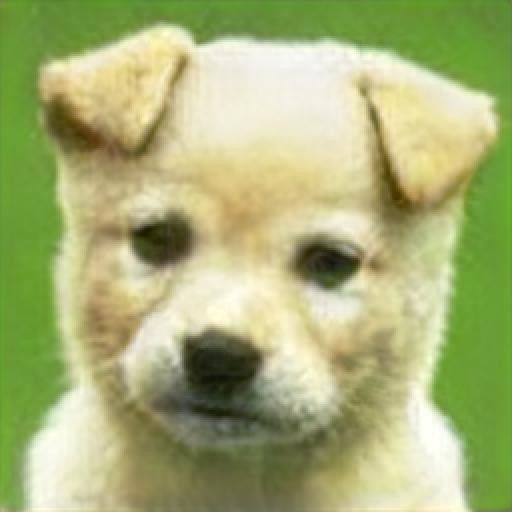} 
\tabularnewline

\includegraphics[width=0.157\linewidth]{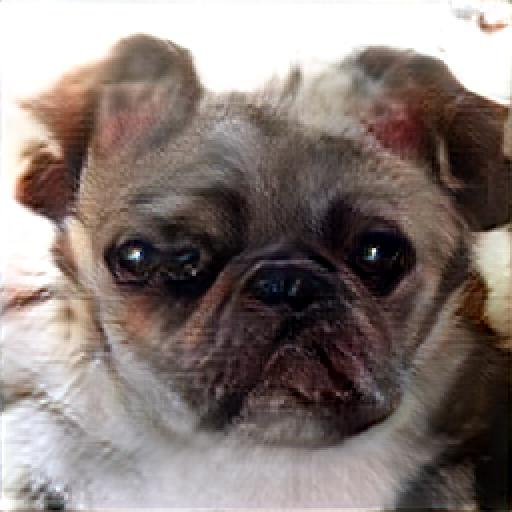} &
\includegraphics[width=0.157\linewidth]{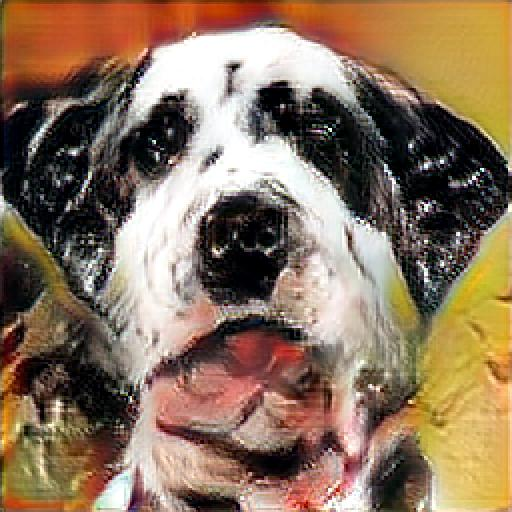} &
\includegraphics[width=0.157\linewidth]{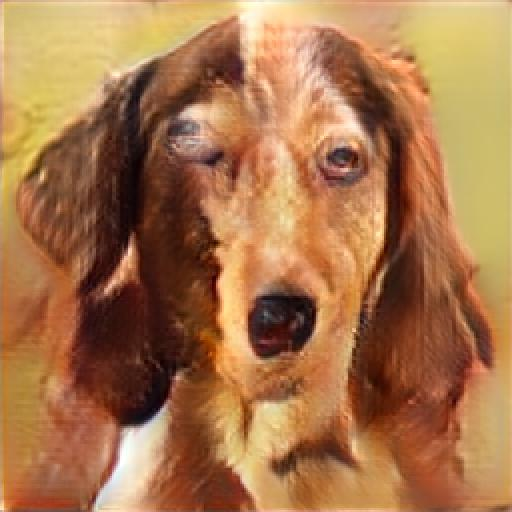} &
\includegraphics[width=0.157\linewidth]{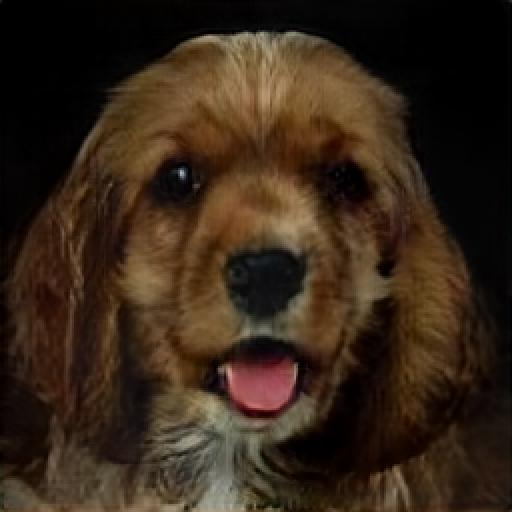} &
\includegraphics[width=0.157\linewidth]{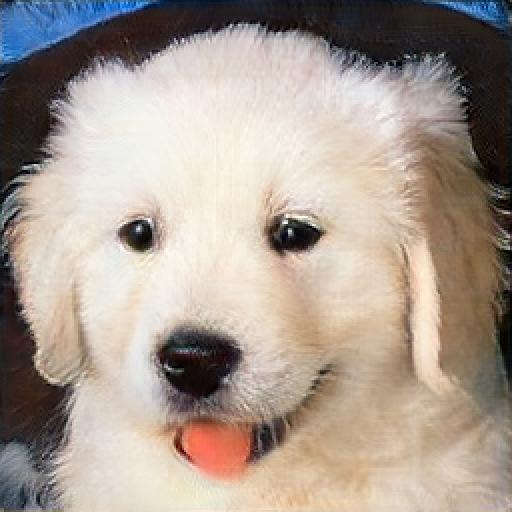} &
\includegraphics[width=0.157\linewidth]{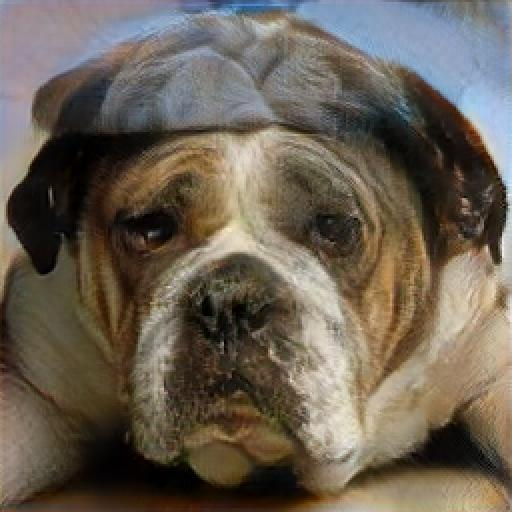}

\end{tabular}\hfill{}
\par\end{centering}
\caption{Visual results in the few-shot setting on the Face Dog dataset. The two upper blocks show generated images for the models trained on the full dataset (389 images), while the two bottom blocks show the results from training only using 25\% of data (98 images). SIV-GAN+ demonstrates not only superior performance on the standard few-shot setting, but also successfully deals with an extreme few-shot scenario (25\% of data), where FastGAN has a significant drop in performance.}
\label{fig:few-shot} 
\end{figure}
