# Supplementary material for: Generating Novel Scene Compositions from Single Images and Videos
Source: arXiv:2103.13389 source file (2023-12-13)
Supplement: Supplementary file 9 [file few-shot_outdoor.tex]

\begin{figure}[t]
\begin{centering}
\setlength{\tabcolsep}{0.1em}

\par\end{centering}
\begin{centering}

\hfill{}%
\begin{tabular}{cc@{\hskip 0.15in}cc}

SIV-GAN+ & Nearest  & SIV-GAN+  & Nearest  
\tabularnewline
generated images & training frames & generated images & training frames
\tabularnewline

\includegraphics[width=0.28\linewidth]{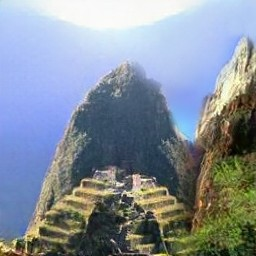} &
\includegraphics[width=0.138\linewidth]{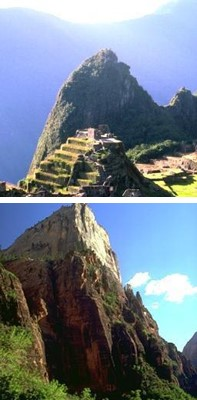} &

\includegraphics[width=0.28\linewidth]{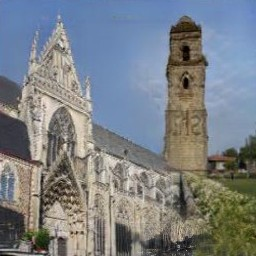} &
\includegraphics[width=0.138\linewidth]{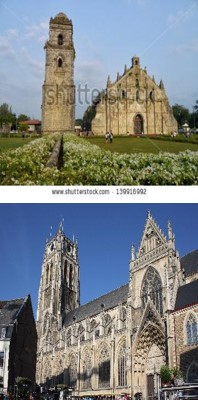} 
\tabularnewline

%\includegraphics[width=0.28\linewidth]{supplementary/figures/outdoors/outd2} &
%\includegraphics[width=0.138\linewidth]{supplementary/figures/outdoors/comb2} &

%\includegraphics[width=0.28\linewidth]{supplementary/figures/outdoors/chur1} &
%\includegraphics[width=0.138\linewidth]{supplementary/figures/outdoors/comb3} 
%\tabularnewline

\tabularnewline 

\multicolumn{4}{c}{SIV-GAN+ generated images}
\tabularnewline
\multicolumn{4}{c}{
	
	~\includegraphics[width=0.14\linewidth]{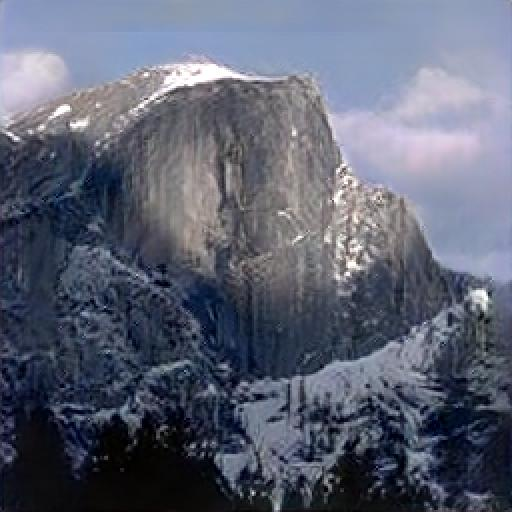}~
	\includegraphics[width=0.14\linewidth]{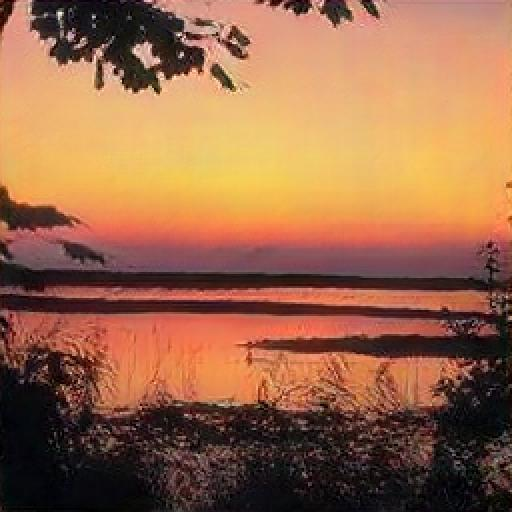}~
	\includegraphics[width=0.14\linewidth]{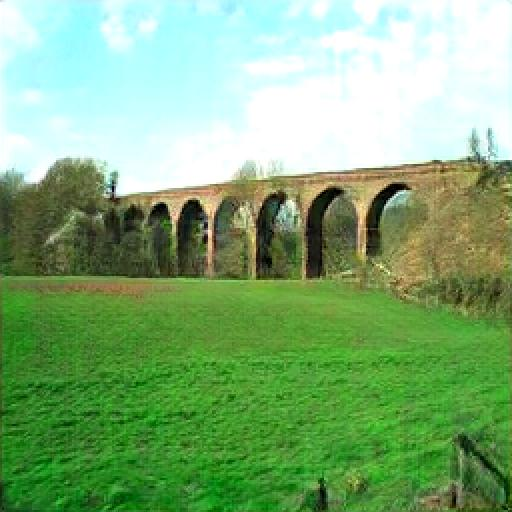}~~
	\includegraphics[width=0.14\linewidth]{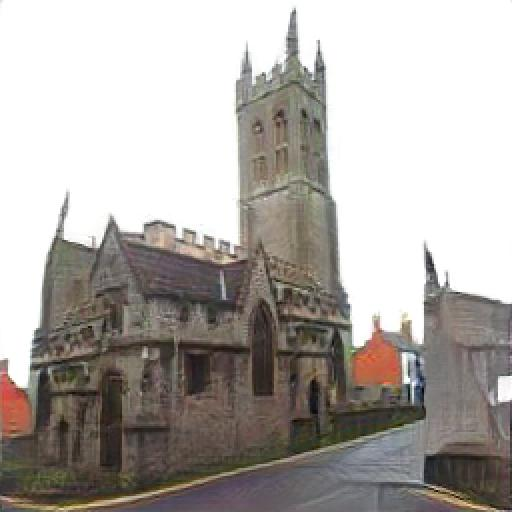}~
	\includegraphics[width=0.14\linewidth]{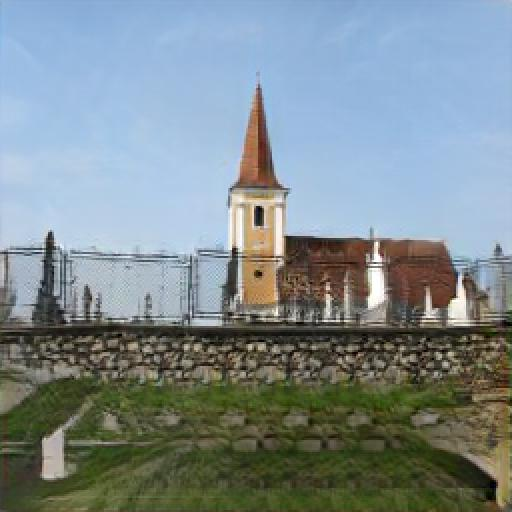}~
	\includegraphics[width=0.14\linewidth]{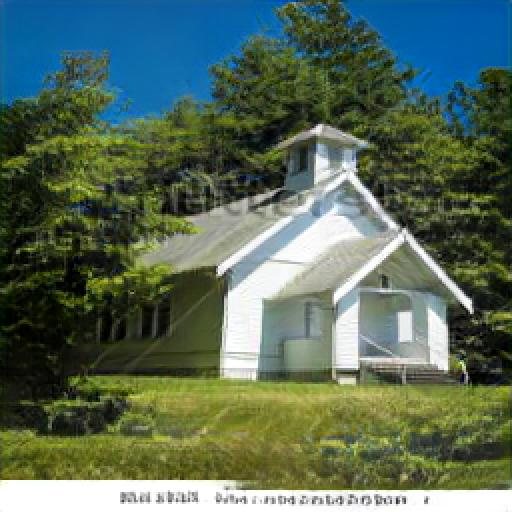}~~
} \tabularnewline \tabularnewline

\multicolumn{4}{c}{FastGAN generated images}
\tabularnewline
\multicolumn{4}{c}{
	
	~\includegraphics[width=0.14\linewidth]{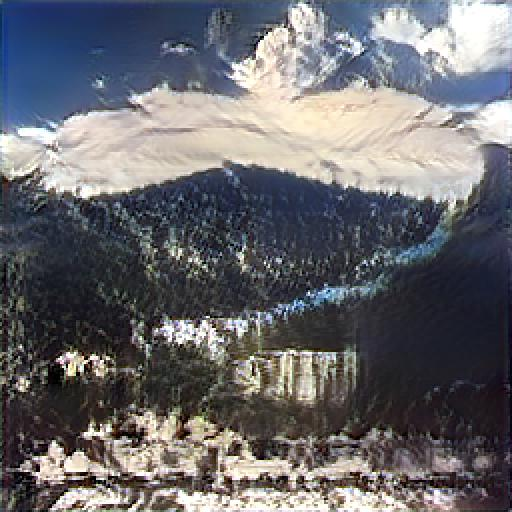}~
	\includegraphics[width=0.14\linewidth]{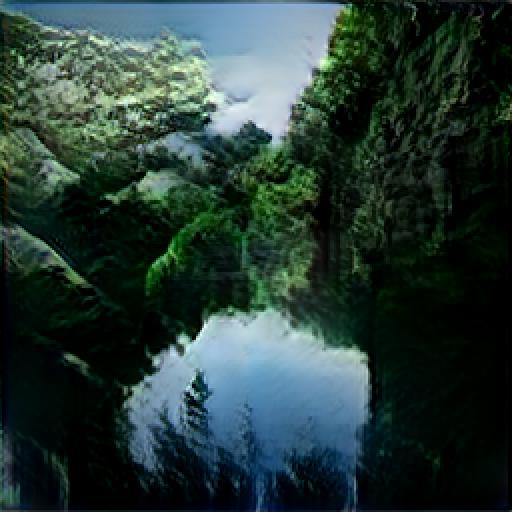}~
	\includegraphics[width=0.14\linewidth]{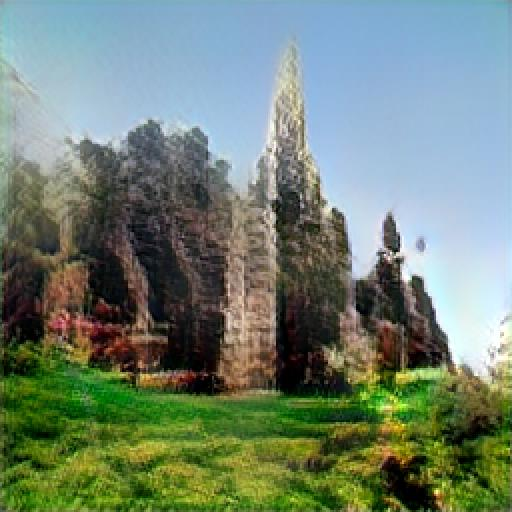}~~
	\includegraphics[width=0.14\linewidth]{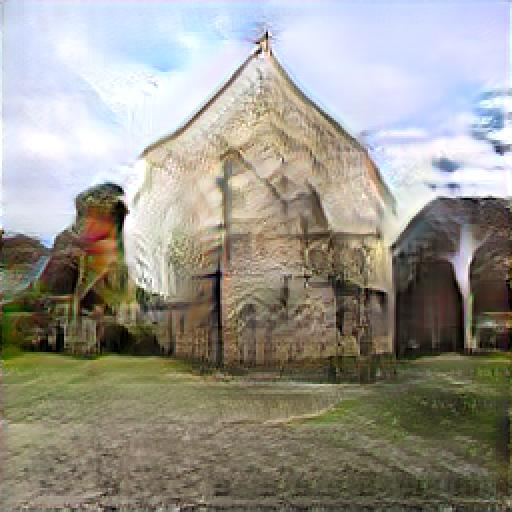}~
	\includegraphics[width=0.14\linewidth]{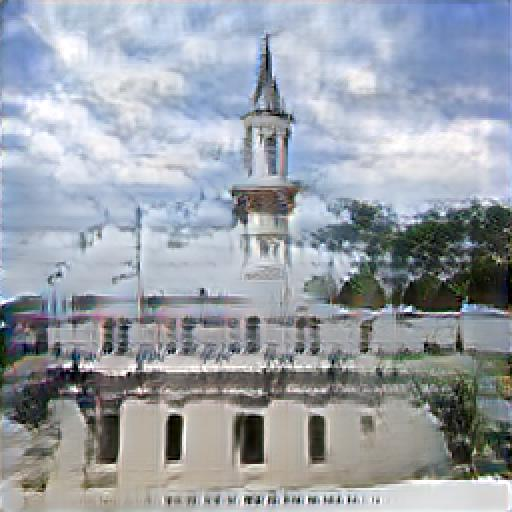}~
	\includegraphics[width=0.14\linewidth]{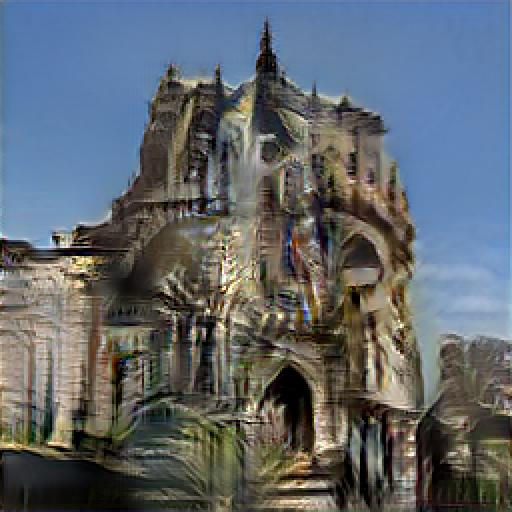}~~
}

\end{tabular}\hfill{}
\par\end{centering}
\caption{Visual examples in the few-shot setting on the ADE-Outdoors and LSUN Church datasets. Despite being trained only on 100 images, SIV-GAN+ does not suffer from memorization issues and achieves an astonishing capability to combine objects from different training images, preserving the global coherency of scenes. In contrast, FastGAN does not achieve high-quality synthesis, struggling to generate coherent images with fine textures.}
%Next to each generated example, two perceptually closest images from the training set are shown.
\label{fig:few-shot_outdoor} 
\end{figure}
