# Supplementary material for: Generating Novel Scene Compositions from Single Images and Videos
Source: arXiv:2103.13389 source file (2023-12-13)
Supplement: Supplementary file 11 [file interpolations.tex]

\begin{wrapfigure}{R}{0.5\textwidth}
	\begin{centering}
		\setlength{\tabcolsep}{0.0em}
		
		\par\end{centering}
	\begin{centering}
		\vspace{-1em}
		%\hfill{}%
		\begin{tabular}{@{}c@{\hskip 0.01in}c@{\hskip 0.05in}c@{}}
		 &\multicolumn{2}{c}{\hspace{-0.1in} \small Progressive upsampling}  
			\tabularnewline	
	 \multirow{-2}{*}{\begin{tabular}{c}  Training image \\ 	\includegraphics[width=0.3\linewidth, height=0.07\textheight]{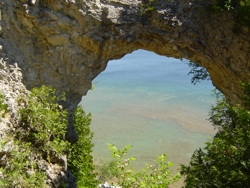}\end{tabular}  } & 
			\includegraphics[width=0.3\linewidth, height=0.07\textheight]{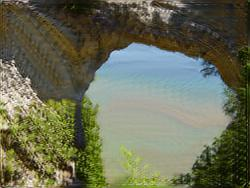} & 
			\includegraphics[width=0.3\linewidth, height=0.07\textheight]{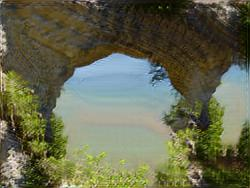} 	\tabularnewline
			& \multicolumn{2}{c}{ \hspace{-0.1in}  \small Adjusted noise} \tabularnewline
			
			& \includegraphics[width=0.3\linewidth, height=0.07\textheight]{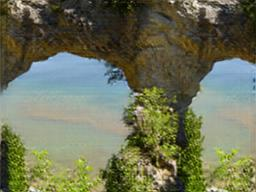} & 
			\includegraphics[width=0.3\linewidth, height=0.07\textheight]{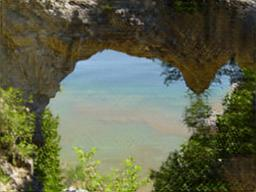}
		% & 	\includegraphics[width=0.3\linewidth]{figures/singan_failures/col3}
			
			\tabularnewline

		\end{tabular}\hfill{}
		\par\end{centering}
	\vspace{-0.5em}
	\caption{\label{fig:interpolations} Different strategies to achieve rectangular shapes. Using progressive upsampling, as in \citep{Shaham2019SinGANLA}, leads to artifacts in textures (e.g. chequered "waves" on the rock). Controlling output image resolution through adjusting noise shape helps to overcome this issue and generate textures of good quality.
		%	As the middle and latest stages cannot correct the layout decision of the first scale generators, without a careful balancing the model falls into producing images of very low diversity or generating incoherent layouts.
	}
	\vspace{-1em}
\end{wrapfigure}
