# Supplementary material for: Generating Novel Scene Compositions from Single Images and Videos
Source: arXiv:2103.13389 source file (2023-12-13)
Supplement: Supplementary file 12 [file qual_ablation_video.tex]

\begin{figure}[t]
\begin{centering}
\setlength{\tabcolsep}{0.1em}

\par\end{centering}
\begin{centering}
\vspace{-1em}
\hfill{}%
\begin{tabular}{@{\hskip -0.05in}c@{\hskip 0.05in}c@{\hskip 0.05in}c@{\hskip 0.05in}c@{\hskip 0.05in}|c@{\hskip 0.05in}c@{\hskip 0.05in}c@{\hskip 0.05in}c}

\rotatebox{90}{ \hspace{0.5ex}\begin{tabular}{c} \small Video \\ \small frames\end{tabular}} &  \multicolumn{3}{c|}{\hspace{-2.05ex} \includegraphics[width=0.463\linewidth, height=0.075\textheight]{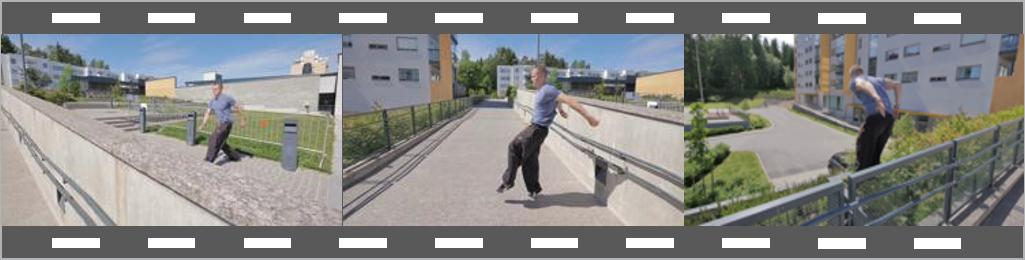} } &
\multicolumn{3}{c}{\includegraphics[width=0.463\linewidth, height=0.075\textheight]{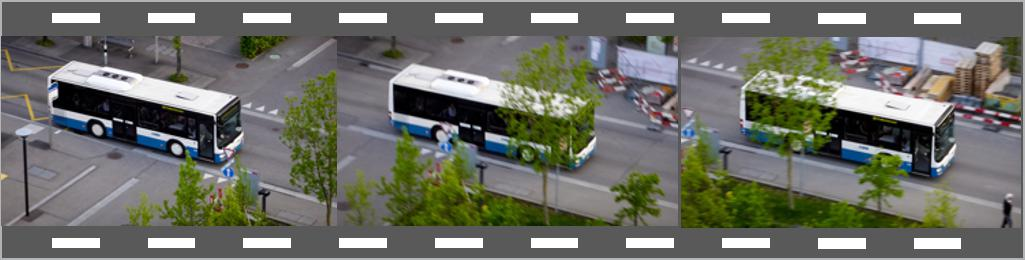}} \tabularnewline

\rotatebox{90}{\hspace{-.9ex}\begin{tabular}{c} \small No \\ \small branches \end{tabular}}&
\includegraphics[width=0.15\linewidth, height=0.06\textheight]{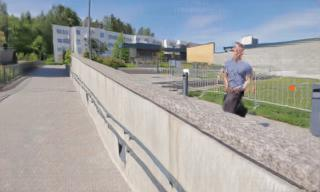} &
\includegraphics[width=0.15\linewidth, height=0.06\textheight]{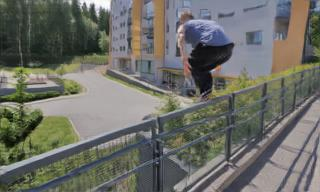} & 
\includegraphics[width=0.15\linewidth, height=0.06\textheight]{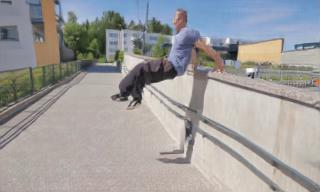} & 
\includegraphics[width=0.15\linewidth, height=0.06\textheight]{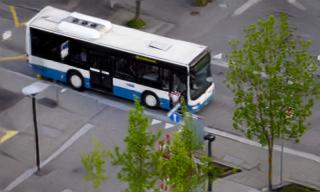} &
\includegraphics[width=0.15\linewidth, height=0.06\textheight]{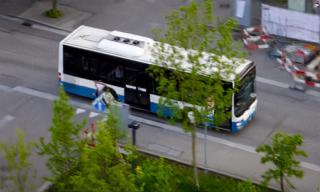} & 
\includegraphics[width=0.15\linewidth, height=0.06\textheight]{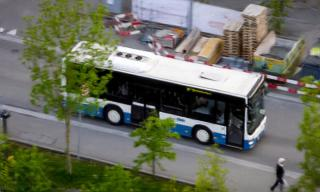} \tabularnewline

\rotatebox{90}{\hspace{-.7ex}\begin{tabular}{c} \small No \\ \small layout \end{tabular}}&
\includegraphics[width=0.15\linewidth, height=0.06\textheight]{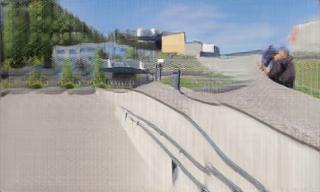} & 
\includegraphics[width=0.15\linewidth, height=0.06\textheight]{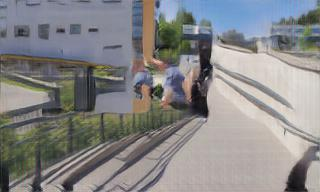} & 
\includegraphics[width=0.15\linewidth, height=0.06\textheight]{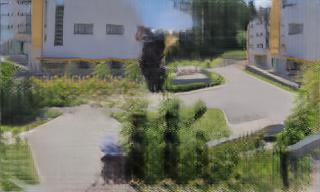} &
\includegraphics[width=0.15\linewidth, height=0.06\textheight]{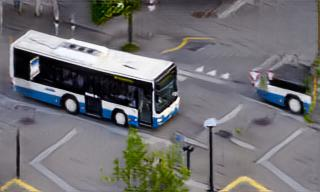} & 
\includegraphics[width=0.15\linewidth, height=0.06\textheight]{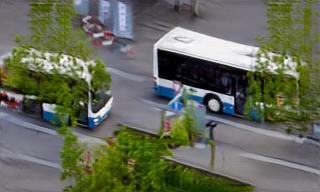} &
\includegraphics[width=0.15\linewidth, height=0.06\textheight]{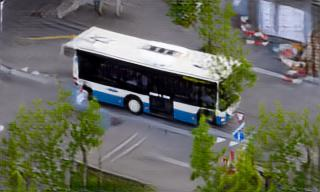}\tabularnewline

\rotatebox{90}{\hspace{-.8ex}\begin{tabular}{c} \small No \\\small content \end{tabular}}&
\includegraphics[width=0.15\linewidth, height=0.06\textheight]{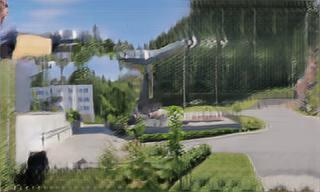} & 
\includegraphics[width=0.15\linewidth, height=0.06\textheight]{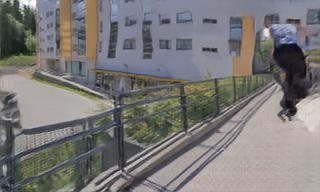} & 
\includegraphics[width=0.15\linewidth, height=0.06\textheight]{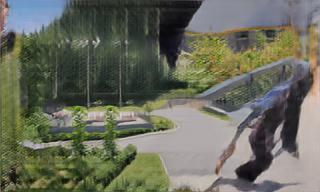} & 
\includegraphics[width=0.15\linewidth, height=0.06\textheight]{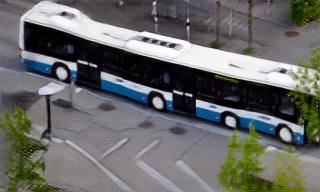} &
\includegraphics[width=0.15\linewidth, height=0.06\textheight]{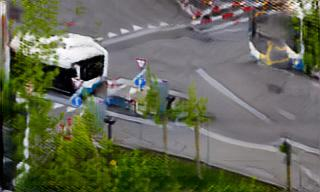} & 
\includegraphics[width=0.15\linewidth, height=0.06\textheight]{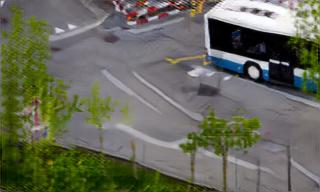}\tabularnewline

\rotatebox{90}{\hspace{-.7ex}\begin{tabular}{c} \small Both \\ \small branches \end{tabular}}&
\includegraphics[width=0.15\linewidth, height=0.06\textheight]{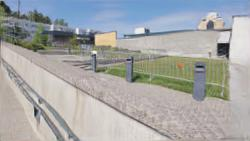} & 
\includegraphics[width=0.15\linewidth, height=0.06\textheight]{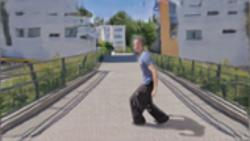} & 
\includegraphics[width=0.15\linewidth, height=0.06\textheight]{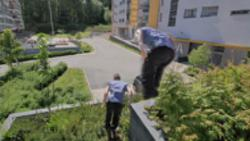} &
\includegraphics[width=0.15\linewidth, height=0.06\textheight]{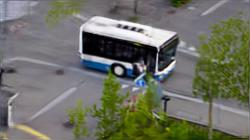} & 
\includegraphics[width=0.15\linewidth, height=0.06\textheight]{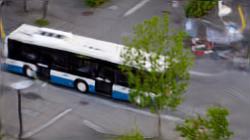} &
\includegraphics[width=0.15\linewidth, height=0.06\textheight]{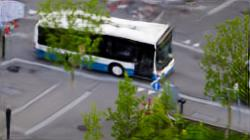}\tabularnewline

\end{tabular}\hfill{}
\par\end{centering}
\vspace{-0.5em}
\caption{\label{fig:qual_abl_video} Visual effects of using content and layout branches in the discriminator in the Single Video setting. 
The model with a standard GAN discriminator (No branches) memorizes the training video frames. The model without the layout branch is prone to cutting objects' contours, generating globally incoherent layouts. The absence of the content branch leads to failures in appearances of objects, such as trees. Finally, the model with both branches generates diverse images maintaining realistic content and layouts.
See Table \ref{table:main_ablation} for qualitative comparison and App.~\ref{supp:qual_ablations_d} for the discussion.
%\anna{add here description of the visual results}
 }
\vspace{-1.0em}
\end{figure}
