# Supplementary material for: Generating Novel Scene Compositions from Single Images and Videos
Source: arXiv:2103.13389 source file (2023-12-13)
Supplement: Supplementary file 14 [file qual_results_image_fastgan.tex]

\begin{figure}[h!]
\begin{centering}
\setlength{\tabcolsep}{0.0em}

\par\end{centering}
\begin{centering}
%\vspace{-1.5em}
%\hfill{}%
\begin{tabular}{@{\hskip -0.03in}c@{\hskip 0.0in}c@{\hskip 0.05in}c@{\hskip 0.11in}c@{\hskip 0.05in}c@{\hskip 0.11in}c@{\hskip 0.05in}c@{}}
 & \multicolumn{2}{c}{SinGAN} &\multicolumn{2}{c}{FastGAN}  & \multicolumn{2}{c}{SIV-GAN}  
\tabularnewline

\multirow{-2}{*}{\begin{tabular}{c}  Training image \\\includegraphics[width=0.13\linewidth, height=0.07\textheight]{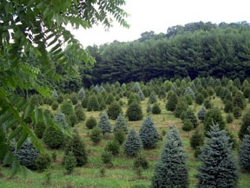} \end{tabular}} &
\includegraphics[width=0.13\linewidth, height=0.07\textheight]{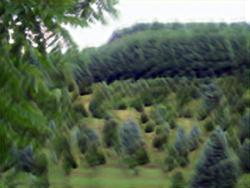} & 
\includegraphics[width=0.13\linewidth, height=0.07\textheight]{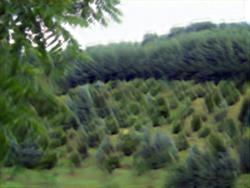} & 
\includegraphics[width=0.13\linewidth, height=0.07\textheight]{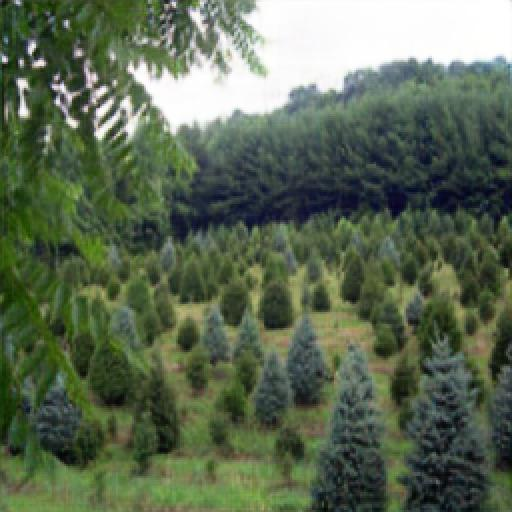} & 
\includegraphics[width=0.13\linewidth, height=0.07\textheight]{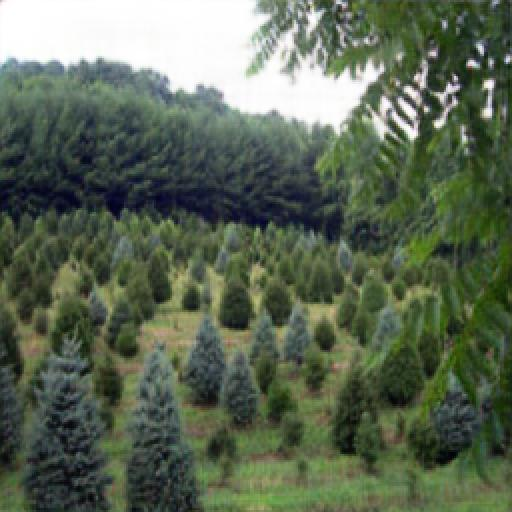} & 
\includegraphics[width=0.13\linewidth, height=0.07\textheight]{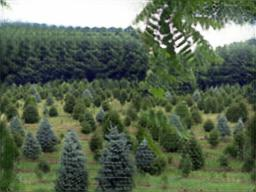} & 
\includegraphics[width=0.13\linewidth, height=0.07\textheight]{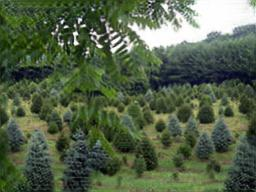}
\tabularnewline
&
\includegraphics[width=0.13\linewidth, height=0.07\textheight]{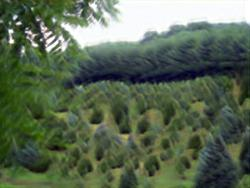} & 
\includegraphics[width=0.13\linewidth, height=0.07\textheight]{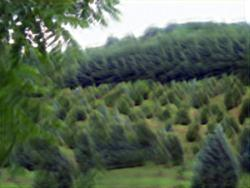} & 
\includegraphics[width=0.13\linewidth, height=0.07\textheight]{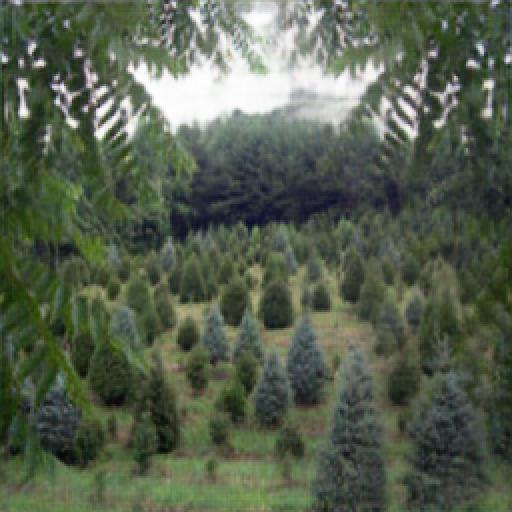} & 
\includegraphics[width=0.13\linewidth, height=0.07\textheight]{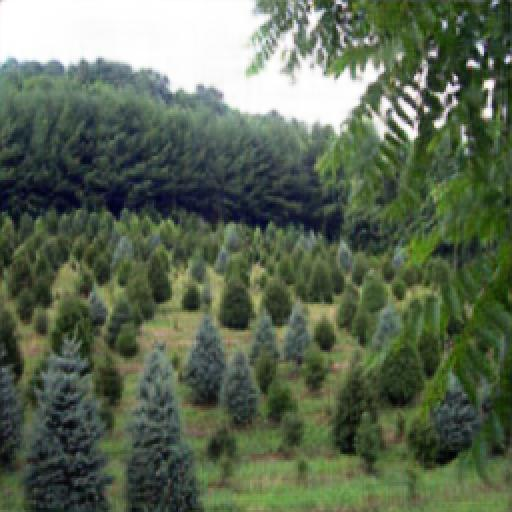} & 
\includegraphics[width=0.13\linewidth, height=0.07\textheight]{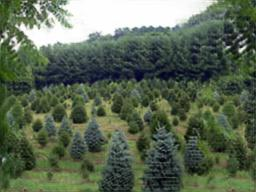} & 
\includegraphics[width=0.13\linewidth, height=0.07\textheight]{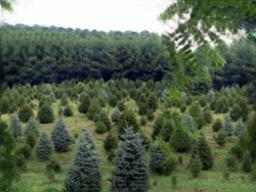} \tabularnewline \tabularnewline

 & \multicolumn{2}{c}{SinGAN} &\multicolumn{2}{c}{FastGAN}  & \multicolumn{2}{c}{SIV-GAN} \tabularnewline

 \multirow{-2}{*}{\begin{tabular}{c}  Training image \\\includegraphics[width=0.13\linewidth, height=0.07\textheight]{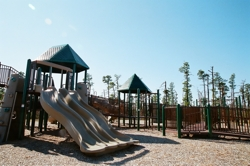} \end{tabular}} &
 \includegraphics[width=0.13\linewidth, height=0.07\textheight]{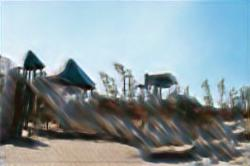} & 
 \includegraphics[width=0.13\linewidth, height=0.07\textheight]{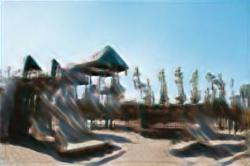} & 
 \includegraphics[width=0.13\linewidth, height=0.07\textheight]{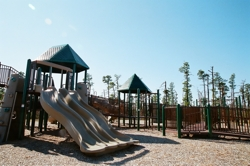} & 
 \includegraphics[width=0.13\linewidth, height=0.07\textheight]{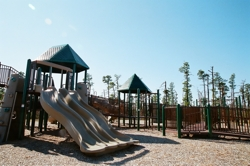} & 
 \includegraphics[width=0.13\linewidth, height=0.07\textheight]{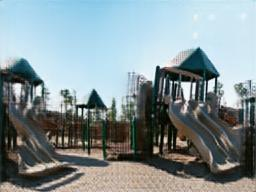} & 
 \includegraphics[width=0.13\linewidth, height=0.07\textheight]{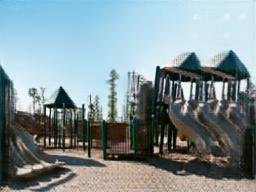}
 \tabularnewline
 &
 \includegraphics[width=0.13\linewidth, height=0.07\textheight]{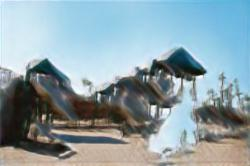} & 
 \includegraphics[width=0.13\linewidth, height=0.07\textheight]{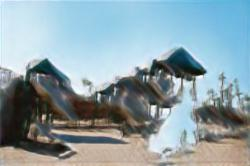} & 
 \includegraphics[width=0.13\linewidth, height=0.07\textheight]{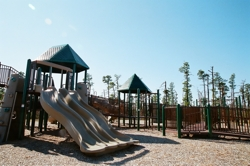} & 
 \includegraphics[width=0.13\linewidth, height=0.07\textheight]{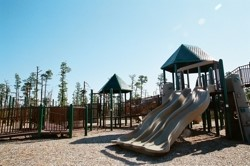} & 
 \includegraphics[width=0.13\linewidth, height=0.07\textheight]{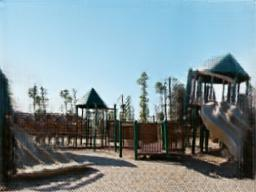} & 
 \includegraphics[width=0.13\linewidth, height=0.07\textheight]{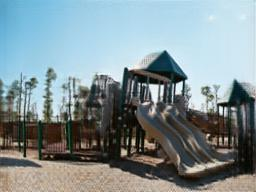} \tabularnewline \tabularnewline
 
 & \multicolumn{2}{c}{SinGAN} &\multicolumn{2}{c}{FastGAN}  & \multicolumn{2}{c}{SIV-GAN} \tabularnewline

\multirow{-2}{*}{\begin{tabular}{c}  Training image \\\includegraphics[width=0.13\linewidth, height=0.07\textheight]{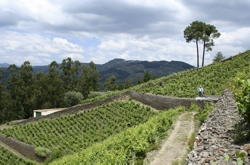} \end{tabular}} &
\includegraphics[width=0.13\linewidth, height=0.07\textheight]{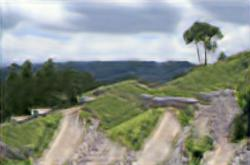} & 
\includegraphics[width=0.13\linewidth, height=0.07\textheight]{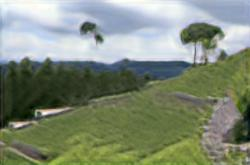} & 
\includegraphics[width=0.13\linewidth, height=0.07\textheight]{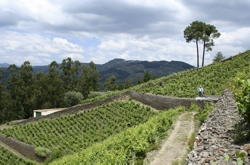} & 
\includegraphics[width=0.13\linewidth, height=0.07\textheight]{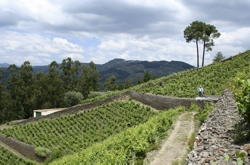} & 
\includegraphics[width=0.13\linewidth, height=0.07\textheight]{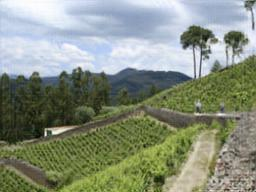} & 
\includegraphics[width=0.13\linewidth, height=0.07\textheight]{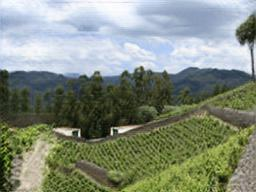}
\tabularnewline
&
\includegraphics[width=0.13\linewidth, height=0.07\textheight]{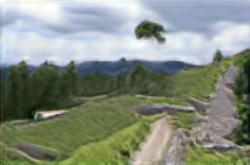} & 
\includegraphics[width=0.13\linewidth, height=0.07\textheight]{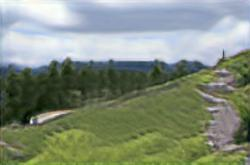} & 
\includegraphics[width=0.13\linewidth, height=0.07\textheight]{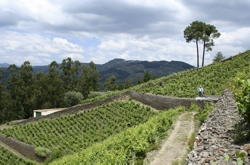} & 
\includegraphics[width=0.13\linewidth, height=0.07\textheight]{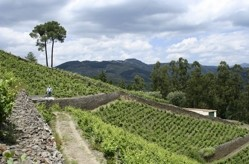} & 
\includegraphics[width=0.13\linewidth, height=0.07\textheight]{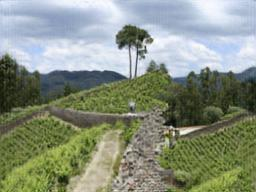} & 
\includegraphics[width=0.13\linewidth, height=0.07\textheight]{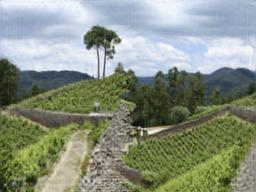} \tabularnewline \tabularnewline

 & \multicolumn{2}{c}{SinGAN} &\multicolumn{2}{c}{FastGAN}  & \multicolumn{2}{c}{SIV-GAN} \tabularnewline

\multirow{-2}{*}{\begin{tabular}{c}  Training image \\\includegraphics[width=0.13\linewidth, height=0.07\textheight]{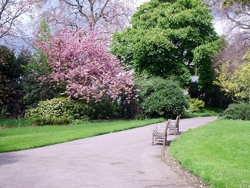} \end{tabular}} &
\includegraphics[width=0.13\linewidth, height=0.07\textheight]{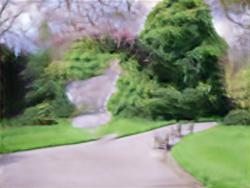} & 
\includegraphics[width=0.13\linewidth, height=0.07\textheight]{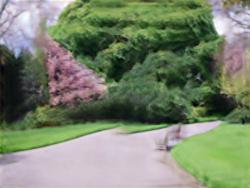} & 
\includegraphics[width=0.13\linewidth, height=0.07\textheight]{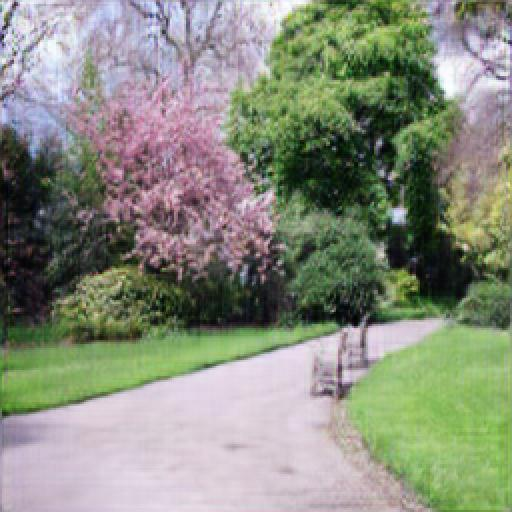} & 
\includegraphics[width=0.13\linewidth, height=0.07\textheight]{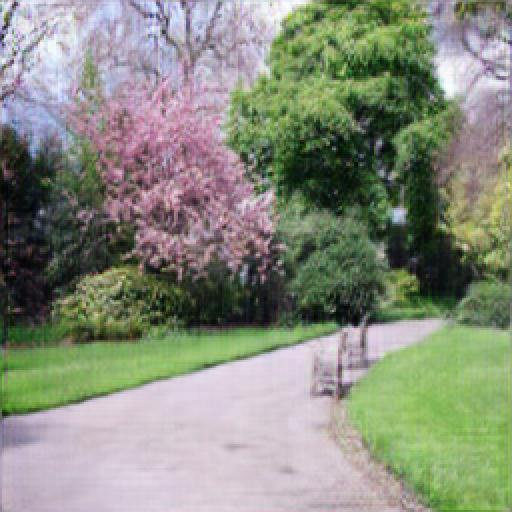} & 
\includegraphics[width=0.13\linewidth, height=0.07\textheight]{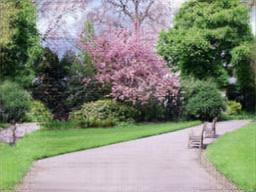} & 
\includegraphics[width=0.13\linewidth, height=0.07\textheight]{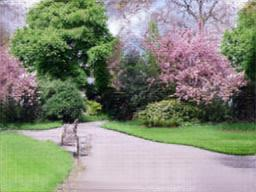}
\tabularnewline
&
\includegraphics[width=0.13\linewidth, height=0.07\textheight]{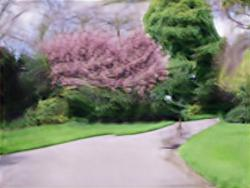} & 
\includegraphics[width=0.13\linewidth, height=0.07\textheight]{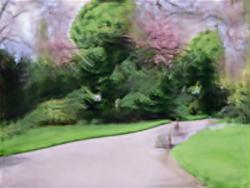} & 
\includegraphics[width=0.13\linewidth, height=0.07\textheight]{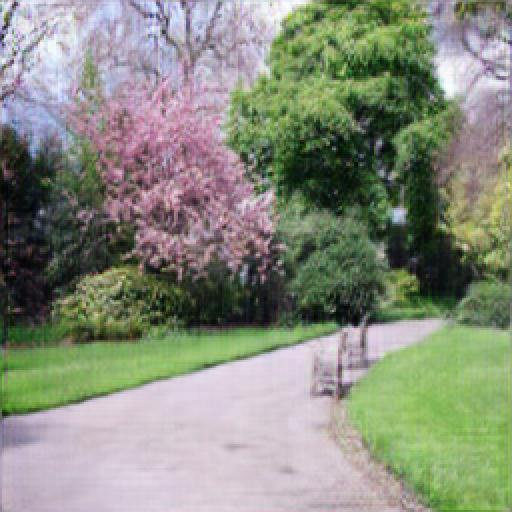} & 
\includegraphics[width=0.13\linewidth, height=0.07\textheight]{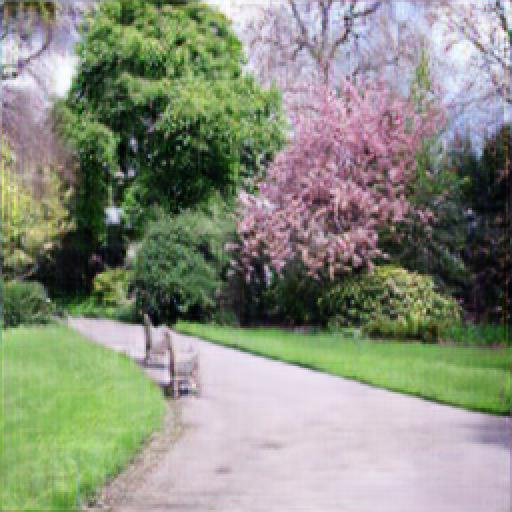} & 
\includegraphics[width=0.13\linewidth, height=0.07\textheight]{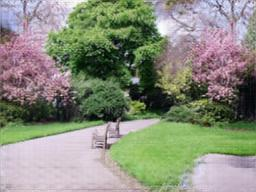} & 
\includegraphics[width=0.13\linewidth, height=0.07\textheight]{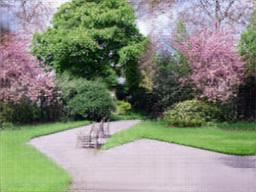} \tabularnewline \tabularnewline

& \multicolumn{2}{c}{SinGAN} &\multicolumn{2}{c}{FastGAN}  & \multicolumn{2}{c}{SIV-GAN} \tabularnewline

\multirow{-2}{*}{\begin{tabular}{c}  Training image \\\includegraphics[width=0.13\linewidth, height=0.07\textheight]{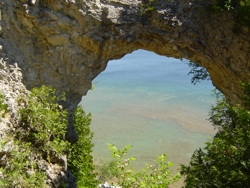} \end{tabular}} &
\includegraphics[width=0.13\linewidth, height=0.07\textheight]{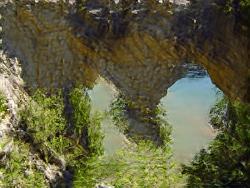} & 
\includegraphics[width=0.13\linewidth, height=0.07\textheight]{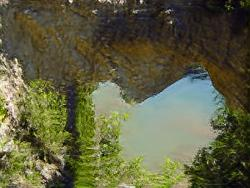} & 
\includegraphics[width=0.13\linewidth, height=0.07\textheight]{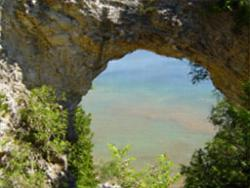} & 
\includegraphics[width=0.13\linewidth, height=0.07\textheight]{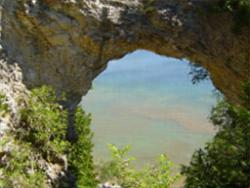} & 
\includegraphics[width=0.13\linewidth, height=0.07\textheight]{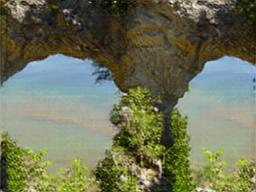} & 
\includegraphics[width=0.13\linewidth, height=0.07\textheight]{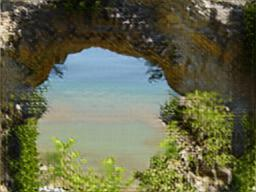}
\tabularnewline
&
\includegraphics[width=0.13\linewidth, height=0.07\textheight]{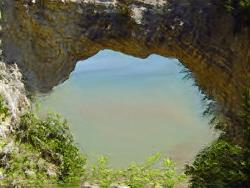} & 
\includegraphics[width=0.13\linewidth, height=0.07\textheight]{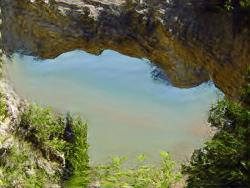} & 
\includegraphics[width=0.13\linewidth, height=0.07\textheight]{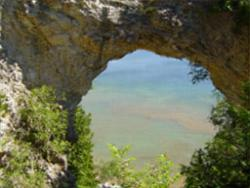} & 
\includegraphics[width=0.13\linewidth, height=0.07\textheight]{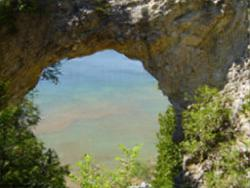} & 
\includegraphics[width=0.13\linewidth, height=0.07\textheight]{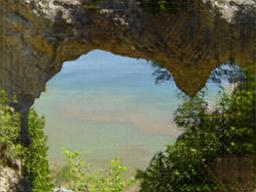} & 
\includegraphics[width=0.13\linewidth, height=0.07\textheight]{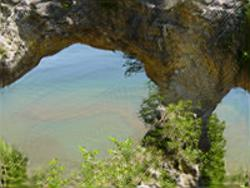} \tabularnewline

\end{tabular}\hfill{}
\par\end{centering}
\vspace{-0.5em}
\caption{\label{fig:qual_image_app_f} Comparison with other methods in the Single Image setting on Places. The single-image GAN of~\citep{Shaham2019SinGANLA} is prone to incoherently shuffle image patches, and the few-shot FastGAN model \citep{anonymous2021towards} reproduces the training image or its flipped version. In contrast, SIV-GAN produces diverse images, preserving the appearance of objects.}
%\vspace{-1em}
\end{figure}
