# Supplementary material for: Generating Novel Scene Compositions from Single Images and Videos
Source: arXiv:2103.13389 source file (2023-12-13)
Supplement: Supplementary file 15 [file qual_results_video.tex]

\begin{figure}[h!]
\begin{centering}
\setlength{\tabcolsep}{0.0em}

\par\end{centering}
\begin{centering}
%\hfill{}%
\centering
\begin{tabular}{c@{\hskip 0.05in}c@{\hskip 0.05in}c@{\hskip 0.05in}c@{\hskip 0.05in}c@{\hskip 0.05in}c}

\multicolumn{6}{c}{
\includegraphics[width=1.00\linewidth]{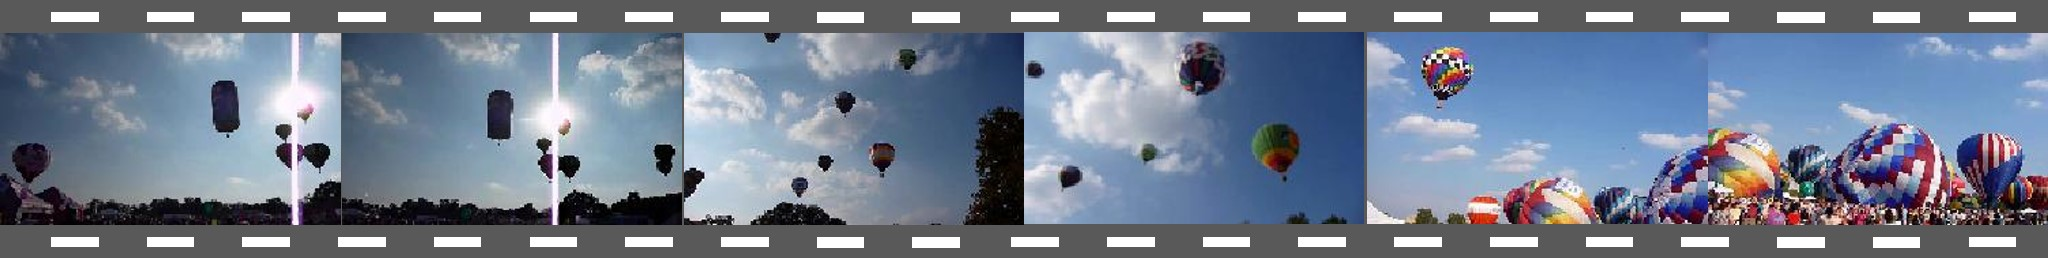}
}

\tabularnewline

\includegraphics[width=0.16\linewidth]{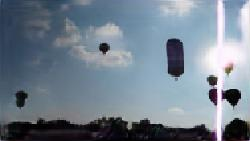} & 
\includegraphics[width=0.16\linewidth]{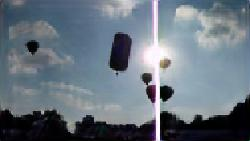} & 
\includegraphics[width=0.16\linewidth]{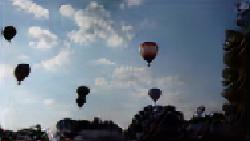} & 
\includegraphics[width=0.16\linewidth]{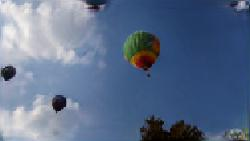} & 
\includegraphics[width=0.16\linewidth]{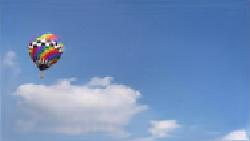} & 
\includegraphics[width=0.16\linewidth]{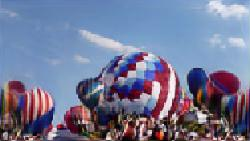} \tabularnewline \tabularnewline

\multicolumn{6}{c}{
	\includegraphics[width=1.00\linewidth]{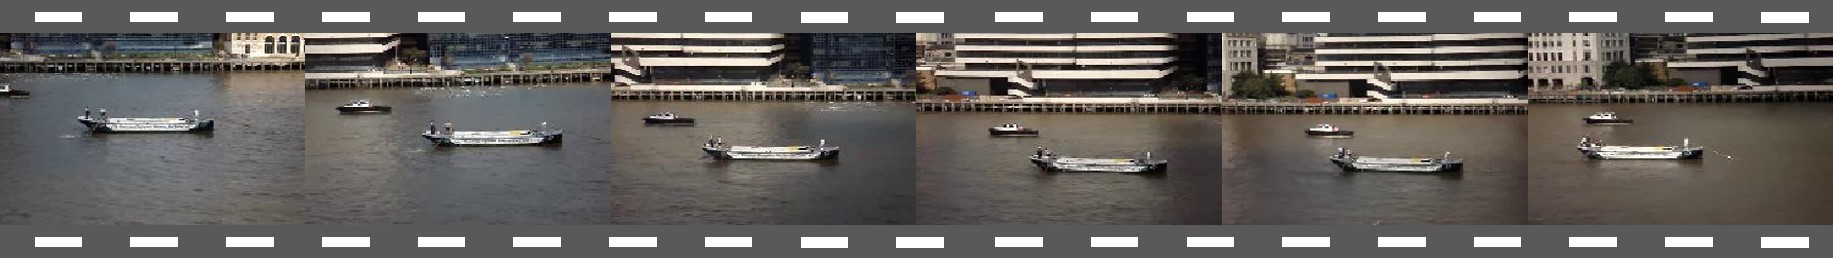}
}

\tabularnewline

\includegraphics[width=0.16\linewidth]{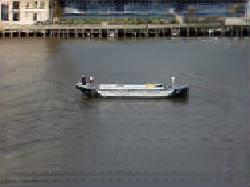} & 
\includegraphics[width=0.16\linewidth]{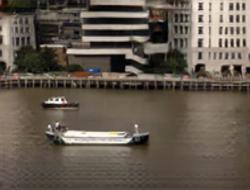} & 
\includegraphics[width=0.16\linewidth]{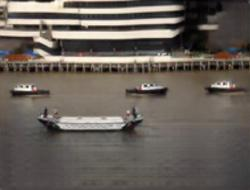} & 
\includegraphics[width=0.16\linewidth]{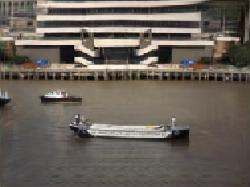} & 
\includegraphics[width=0.16\linewidth]{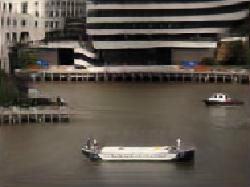} & 
\includegraphics[width=0.16\linewidth]{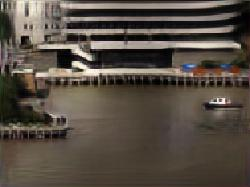} \tabularnewline \tabularnewline

\multicolumn{6}{c}{
	\includegraphics[width=1.00\linewidth]{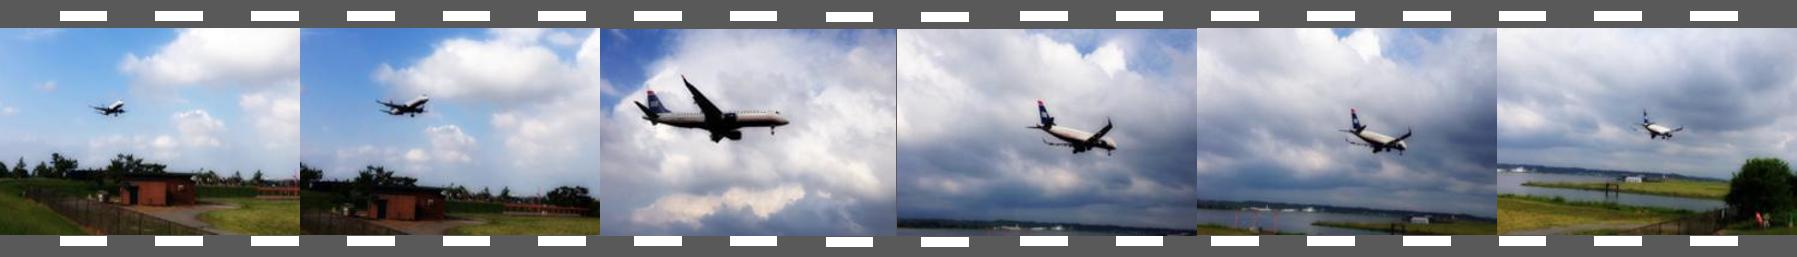}
}

\tabularnewline

\includegraphics[width=0.16\linewidth]{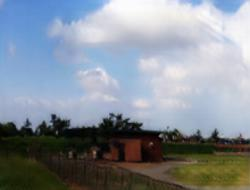} & 
\includegraphics[width=0.16\linewidth]{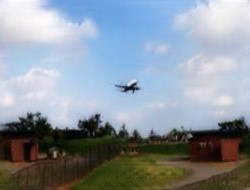} & 
\includegraphics[width=0.16\linewidth]{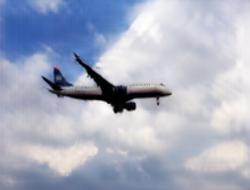} & 
\includegraphics[width=0.16\linewidth]{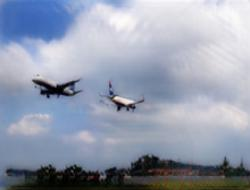} & 
\includegraphics[width=0.16\linewidth]{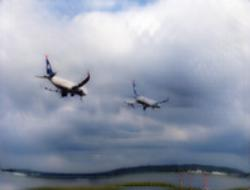} & 
\includegraphics[width=0.16\linewidth]{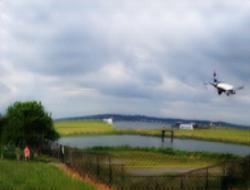} \tabularnewline \tabularnewline

\multicolumn{6}{c}{
	\includegraphics[width=1.00\linewidth]{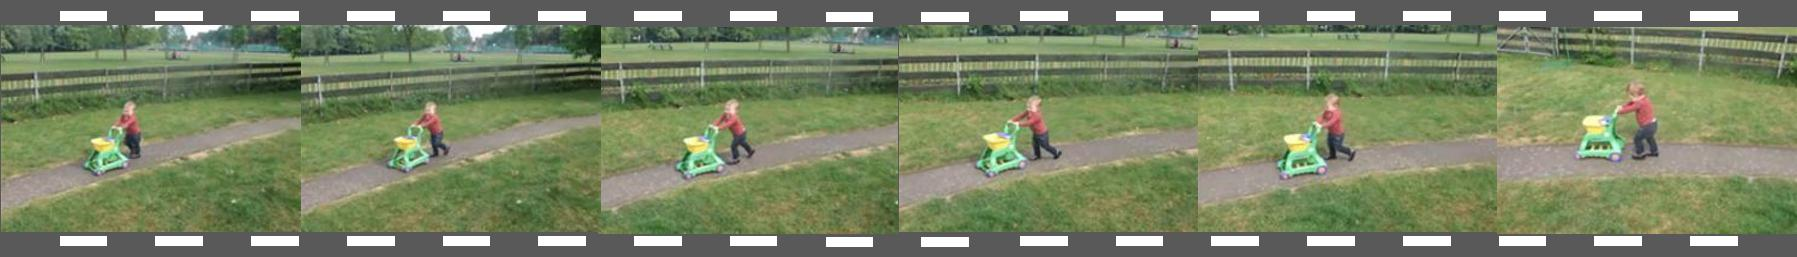}
}

\tabularnewline

\includegraphics[width=0.16\linewidth]{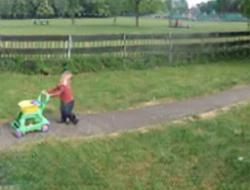} & 
\includegraphics[width=0.16\linewidth]{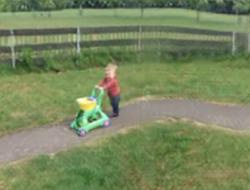} & 
\includegraphics[width=0.16\linewidth]{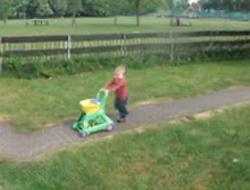} & 
\includegraphics[width=0.16\linewidth]{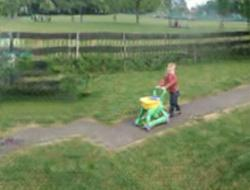} & 
\includegraphics[width=0.16\linewidth]{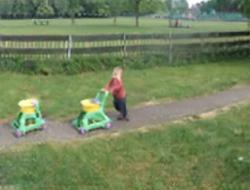} & 
\includegraphics[width=0.16\linewidth]{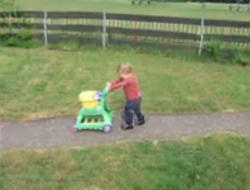} \tabularnewline \tabularnewline

\end{tabular}\hfill{}
\par\end{centering}
\caption{\label{fig:qual_video_app} Additional qualitative results in the Single Video setting. The training sequences are shown in grey frames. Given a single video for training, our SIV-GAN produces images that are different to the training frames. For example, for a video with air balloons, the generated images have different number of balloons, while for a video with a boat, the model generates novel combinations of boats and buildings not seen during training.}
\vspace{1em}
\end{figure}
