# Supplementary material for: Generating Novel Scene Compositions from Single Images and Videos
Source: arXiv:2103.13389 source file (2023-12-13)
Supplement: Supplementary file 16 [file compare_im_vid.tex]

\begin{table}[b]

	\setlength{\tabcolsep}{0.25em}
	
	\centering
			\caption{Comparison of the diversity among the images generated in the Single Image and the Single Video settings on the DAVIS-YFCC100M dataset.}
	\vspace{0.5em}
	\begin{tabular}{c|c|c}
{\normalsize{} Data setting } & { LPIPS~$\uparrow$ } & { MS-SSIM~$\downarrow$}   \tabularnewline
	
	\hline 	\hline 	
	
	{ Single Image  }  & 0.33  & 0.63 \tabularnewline

	{ Single Video  }  & \textbf{0.43}  & \textbf{0.54}

	%\vspace{-0.5em}
	\end{tabular}

	\label{table:compare_im_vid} %
\end{table}
