# Supplementary material for: Generating Novel Scene Compositions from Single Images and Videos
Source: arXiv:2103.13389 source file (2023-12-13)
Supplement: Supplementary file 17 [file d_blocks.tex]

\begin{table}[h!]
	\setlength{\tabcolsep}{0.25em}

\centering
\centering
	\caption{The SIV-GAN discriminator. In this example, the configuration is presented for the input noise of size $(3\times 5)$ and the final resolution of $(192\times320)$, corresponding to training on the DAVIS-YFCC100M dataset in the Single Video setting.}

\vspace{0.5em}

	\begin{tabular}{l|l l|l l}
		 Operation  & Input  & Size &  Output  & Size  \tabularnewline
		\hline
		\hline
		\multicolumn{5}{c}{Low-level features $D_{low-level}$} \\ \hline
		Conv2D & \texttt{image\_0} & (3,192,320)              & \texttt{feat\_0}  & (32,192,320)\\\hline 
		Conv2D & \texttt{image\_1} & (3,96,160)              & \texttt{feat\_1}  & (8,96,160)\\\hline 
		Conv2D & \texttt{image\_2} & (3,48,80)              & \texttt{feat\_2}  & (16,48,80)\\\hline 		
{ResBlock-Down} & 
		\texttt{feat\_0} & (32,192,320) & {\texttt{down\_0}} & {(64,96,160)} \\ \hline
		\multirow{2}{*}{ResBlock-Down} & \texttt{down\_0} & (64,96,160) & \multirow{2}{*}{\texttt{down\_1}} & \multirow{2}{*}{(128,48,80)} \\
& \texttt{feat\_1} & (8, 96, 160) & & \\ \hline
		\multirow{2}{*}{ResBlock-Down} & \texttt{down\_1} & (128,48,80) & \multirow{2}{*}{\texttt{F}} & \multirow{2}{*}{(256,24,40)} \\
& \texttt{feat\_2} & (16,48, 80) & & \\ \hline \hline
		\multicolumn{5}{c}{Content branch $D_{content}$} \\ \hline
		AvgPool & \texttt{F} & (256,24,40)   & \texttt{F\_con} & (256,1,1) \\\hline
		ResBlock-Down & \texttt{F\_con} & (256,1,1)   & \texttt{cont\_0} & (256,1,1) \\\hline
		ResBlock-Down & \texttt{cont\_0} & (256,1,1)   & \texttt{cont\_1} & (256,1,1) \\\hline
		ResBlock-Down & \texttt{cont\_1} & (256,1,1)   & \texttt{cont\_2} & (256,1,1) \\\hline
		ResBlock-Down & \texttt{cont\_2} & (256,1,1)     & \texttt{cont\_3} & (256,1,1) \\ \hline \hline
		\multicolumn{5}{c}{Layout branch $D_{layout}$} \\ \hline
		Conv2D & \texttt{F} & (256,24,40)   & \texttt{F\_lay} & (1,24,40) \\\hline
	ResBlock-Down & \texttt{F\_lay} & (1,24,40)   & \texttt{lay\_0} & (1,12,20) \\\hline
	ResBlock-Down & \texttt{lay\_0} & (1,12,20)   & \texttt{lay\_1} & (1,6,10) \\\hline
	ResBlock-Down & \texttt{lay\_1} & (1,6,10)   & \texttt{lay\_2} & (1,3,5) \\\hline
	ResBlock-Down & \texttt{lay\_2} & (1,3,5)     & \texttt{lay\_3} & (1,3,5) \\ \hline \hline

	\end{tabular}
\centering

\label{table:d_arch} %

%\end{minipage}%
%\hfill
%\begin{minipage}{.42\linewidth}
%\vspace{-1em}
%\hfill
%\includegraphics[width=0.43\textwidth]{figures/colors-textures/texture_pdf6}
%\hfill
%\vspace{0.2em}
%\captionof{figure}{{Histogram distances to real data.}}	\label{fig:color-texture} %
%\end{minipage}%

		%	\vspace{-0.5em}
\end{table}
