# Supplementary material for: Generating Novel Scene Compositions from Single Images and Videos
Source: arXiv:2103.13389 source file (2023-12-13)
Supplement: Supplementary file 18 [file few-shot.tex]

\begin{table}
	\setlength{\tabcolsep}{0.4em}
	
	\centering

	\caption{Results on the few-shot image synthesis task. The FID is computed between 5000 generated images and the whole training set.  \textbf{Bold} and \underline{underlined} indicate first and second best scores. Our SIV-GAN+ achieves better FID scores compared to FastGAN on all few-shot datasets, also outperforming the model from LeCam~\citep{tseng2021regularizing} on four out of five datasets.}
	\vspace{0.5em}
	\begin{tabular}{l|l|c@{\hskip 0.10in}c@{\hskip 0.10in}c@{\hskip 0.10in}c@{\hskip 0.10in}c}
%	  & \multicolumn{5}{c}{FID~$\downarrow$}  \tabularnewline		\cline{2-6}

	 \multirow{2}{*}{FID~$\downarrow$} & \multicolumn{1}{c|}{ Dataset:} & {} Obama & {} Grumpy Cat & {} Panda & {} Face Cat & {} Face Dog  \tabularnewline \cline{2-7}
	 
	& \multicolumn{1}{c|}{ Number of images:} & {} 100 & {} 100  & {} 100  & {} 160  & {} 389   \tabularnewline
	\hline \hline 
		
		\multicolumn{2}{l|}{Scale/Shift \citep{Noguchi2019ImageGF} \hfill $\circlearrowright$}  &  {50.72}  &  {34.20} & {21.38} &  {54.83} &  {83.04}  \tabularnewline
		\multicolumn{2}{l|}{MineGAN  \citep{Wang2020MineGANEK} \hfill $\circlearrowright$}  &  {50.63}  &  {34.54} & {14.84} &  {54.45} &  {93.08}  \tabularnewline
		\multicolumn{2}{l|}{TransferGAN \citep{Wang2018TransferringGG} \hfill $\circlearrowright$}  &  {48.73}  &  {34.06} & {23.20} &  {52.61} &  {82.38}  \tabularnewline
		%{} TransferGAN + DA  & {} \cmark &  {39.85}  &  {29.77} & {17.12} &  {49.10} &  {65.57}  \tabularnewline
		\multicolumn{2}{l|}{FreezeD \citep{Mo2020FreezeDA} \hfill $\circlearrowright$}  &  {41.87}  &  {31.22} & {17.95} &  {47.70} &  {70.46}  \tabularnewline \hline
		%{} TransferGAN + DA  & {} \cmark &  {35.75}  &  {29.32} & {14.50} &  {46.07} &  {61.03}  \tabularnewline
		%\hline 
		%{} StyleGANv2  &  &  {80.45}  &  {48.63} & {34.07} &  {69.84} &  {129.9}  \tabularnewline
		%{} StyleGANv2 + DA  &  &  {47.09}  &  {27.21} & {12.13} &  {42.40} &  {58.47}  \tabularnewline
		\multicolumn{2}{l|}{LeCam \citep{tseng2021regularizing}}  &  \textbf{{33.16}}  &  \underline{{24.93}} & {10.16} &  {34.18} &  {54.88}  \tabularnewline
		 
		\multicolumn{2}{l|}{FastGAN \citep{anonymous2021towards}}   &  {38.59}  &  {27.08} & \underline{{9.63}} &  \underline{{33.50}} &  \underline{{53.39}}  \tabularnewline
		\multicolumn{2}{l|}{SIV-GAN+}  &  \underline{{35.10}}  &  \textbf{{23.79}} & \textbf{{9.22}} &  \textbf{{31.24}} &  \textbf{{50.05}}  \tabularnewline
		\multicolumn{7}{r}{$\circlearrowright$ - models which use pre-training}
		
	\end{tabular}
	\vspace{-1.5em}
	\label{table:few-shot} %
\end{table}
