# Supplementary material for: Generating Novel Scene Compositions from Single Images and Videos
Source: arXiv:2103.13389 source file (2023-12-13)
Supplement: Supplementary file 19 [file few-shot_extreme.tex]

\begin{table}
	\setlength{\tabcolsep}{0.044in}
	
	\centering
	\caption{Results in the extremely low few-shot data setting, where the models are trained only on subsets of standard few-shot datasets. Our model outperforms the baseline in all data regimes both in quality and diversity, and does not suffer from training instabilities even in extreme cases, such as using only 25\% of the training set. Collapsed runs with a high FID for Fast-GAN are shown in red.}
	\vspace{0.5em}
	
	\begin{tabular}{l|cc|cc|cc|cc|cc|cc}

	 \multirow{3}{*}{Method} & \multicolumn{6}{c|}{Panda (100)} & \multicolumn{6}{c}{Face Dog (389)}  \tabularnewline
	 
	 & \multicolumn{2}{c|}{100\%} & \multicolumn{2}{c|}{50\%} & \multicolumn{2}{c|}{25\%} &  \multicolumn{2}{c|}{100\%} & \multicolumn{2}{c|}{50\%} & \multicolumn{2}{c}{25\%}
	 \tabularnewline		
	 
	 & \small{FID} &  \small{LPIPS}  &  \small{FID} &  \small{LPIPS} & \small{FID} & \small{LPIPS} &  \small{FID} &  \small{LPIPS} &  \small{FID} & \small{LPIPS}  &  \small{FID} & \small{LPIPS} \tabularnewline
	
		\hline 	\hline 	
		
	FastGAN  & {9.63} & {0.48}   &  {13.97} &  {0.49} & \color{darkred} {16.08} & {0.47} & {53.39} &   {0.62} &  {77.57} &  {0.61} &  \color{darkred} {96.86} &  {0.61}  \tabularnewline

	SIV-GAN+  & \textbf{{9.22}} &  \textbf{{0.51}}  &  \textbf{{11.57}} &  \textbf{{0.51}} & \textbf{{9.58}} & \textbf{{0.50}} &  \textbf{{50.05}} &  \textbf{{0.63}} &  \textbf{{64.21}} &  \textbf{{0.62}} &  \textbf{{62.61}} &  \textbf{{0.62}} \tabularnewline

	\end{tabular}

	\label{table:few-shot_extreme} %
\end{table}
