# Supplementary material for: Generating Novel Scene Compositions from Single Images and Videos
Source: arXiv:2103.13389 source file (2023-12-13)
Supplement: Supplementary file 20 [file few-shot_outdoor.tex]

\begin{table}[t]
	\setlength{\tabcolsep}{0.038in}

	\centering
	
	\caption{Results on few-shot datasets with a non-object-centric structure. Our model outperforms FastGAN both in quality and diversity on both datasets.}
	\vspace{0.5em}
	
	\begin{tabular}{l|cc|cc|cc|cc|cc|cc}

	\multirow{3}{*}{Method} & \multicolumn{6}{c|}{ADE-Outdoor (100)} & \multicolumn{6}{c}{LSUN Church (100)}  \tabularnewline
	
	& \multicolumn{2}{c|}{100\%} & \multicolumn{2}{c|}{50\%} & \multicolumn{2}{c|}{25\%} &  \multicolumn{2}{c|}{100\%} & \multicolumn{2}{c|}{50\%} & \multicolumn{2}{c}{25\%}
	\tabularnewline		
	
	& \small{FID} &  \small{LPIPS}  &  \small{FID} &  \small{LPIPS} & \small{FID} & \small{LPIPS} &  \small{FID} &  \small{LPIPS} &  \small{FID} & \small{LPIPS}  &  \small{FID} & \small{LPIPS} \tabularnewline
	
	\hline 	\hline 	
	
	FastGAN  & {113.2} & {0.62}   &  {125.1} &  {0.62} & {98.28} & {0.61} & {90.65} &   {0.58} &  {121.4} &  {0.58} &   {114.1} &  {0.56}  \tabularnewline

	SIV-GAN+  & \textbf{{88.46}} &  \textbf{{0.64}}  &  \textbf{{82.89}} &  \textbf{{0.63}} & \textbf{{52.96}} & \textbf{{0.63}} &  \textbf{{85.01}} &  \textbf{{0.60}} &  \textbf{{103.8}} &  \textbf{{0.60}} &  \textbf{{90.10}} &  \textbf{{0.59}} \tabularnewline
		
	\end{tabular}

	\label{table:few-shot_outdoor} %
\end{table}
