# Supplementary material for: Generating Novel Scene Compositions from Single Images and Videos
Source: arXiv:2103.13389 source file (2023-12-13)
Supplement: Supplementary file 21 [file g_blocks.tex]

\begin{table}[h!]
	
	\setlength{\tabcolsep}{0.25em}
	
	\centering
	\centering
	\caption{The SIV-GAN generator. In this example, the configuration is presented for the input noise of size $(3\times 5)$ and the final resolution of $(192\times320)$, corresponding to training on the DAVIS-YFCC100M dataset in the Single Video setting.}
	
	\vspace{0.5em}
	\begin{tabular}{l|l l|l l}
		 Operation  & Input  & Size &  Output  & Size  \tabularnewline
		\hline
		\hline
{ConvTransp2D} & \texttt{z} & (64,1,1)          & {\texttt{up\_0}}  & {(256,3,5)}\\ \hline
		{ResBlock-Up} & \texttt{up\_0}  & (256,3,5)   & {\texttt{up\_1}} & {(256,3,5)} \\ 
		\hline
		{ResBlock-Up} & \texttt{up\_1}  & (256,3,5)   & {\texttt{up\_2}} & {(256,6,10)} \\ 
		\hline
		{ResBlock-Up} & \texttt{up\_2}  & (256,6,10)   & {\texttt{up\_2}} & {(256,12,20)} \\ 
		\hline
		{ResBlock-Up} & \texttt{up\_3}  & (256,12,20)   & {\texttt{up\_3}} & {(256,24,40)} \\ \hline
		{ResBlock-Up} & \texttt{up\_4}  & (256,24,40)   & {\texttt{up\_4}} & {(256,48,80)} \\ \hline
        {ResBlock-Up} & \texttt{up\_5}  & (256,48,80)   & {\texttt{up\_5}} & {(128,96,160)} \\ \hline
		{ResBlock-Up} & \texttt{up\_6}  & (128,96,160)   & {\texttt{up\_6}} & {(64,192,320)} \\ \hline \hline
		Conv2D, TanH           & \texttt{up\_5} & (128,48,80)     & \texttt{image\_2}  & (3,48,80)\\\hline
		Conv2D, TanH           & \texttt{up\_6} & (64,96,160)     & \texttt{image\_1}  & (3,96,160)\\\hline
		Conv2D, TanH           & \texttt{up\_7} & (32,192,320)     & \texttt{image\_0}  & (3,192,320)\\\hline

	\end{tabular}

\label{table:g_arch} %

\end{table}
