# Supplementary material for: Generating Novel Scene Compositions from Single Images and Videos
Source: arXiv:2103.13389 source file (2023-12-13)
Supplement: Supplementary file 22 [file interpolations.tex]

\begin{table}[b]

	\setlength{\tabcolsep}{0.2em}
	
	\centering
	\caption{Effect of different strategies to match the rectangular shape of the original training image on the DAVIS-YFCC100M dataset. }
	\vspace{0.5em}	
	\begin{tabular}{c|c|c||c|c}
		 \multirow{2}{*}{ Interpolation} & \multicolumn{2}{c||}{Single Image}  & \multicolumn{2}{c}{Single Video}  
		\tabularnewline
		 \small{} & {{} SIFID~$\downarrow$}  & {{} LPIPS~$\uparrow$ } &  {{} SIFID~$\downarrow$} & {{} LPIPS~$\uparrow$ } \tabularnewline

		\hline 	\hline 	
		
		 {} Progressive upsampling & {{0.11}} &  {0.32} &  {0.65} &  {0.42}  \tabularnewline

		 {} Adjusted noise & \textbf{{{0.08}}}  &  \textbf{{0.33}} &  \textbf{{0.55}} &  \textbf{{0.43}}  \tabularnewline
	
		\end{tabular}
	\vspace{-0.5em}

\label{table:interpolations} %

\end{table}
