# Supplementary material for: Generating Novel Scene Compositions from Single Images and Videos
Source: arXiv:2103.13389 source file (2023-12-13)
Supplement: Supplementary file 23 [file layout_width.tex]

\begin{table}[h!]

	\setlength{\tabcolsep}{0.2em}
	
	\centering
	
	\caption{Ablation on the number of channels used for the layout branch feature representation on the DAVIS-YFCC100M dataset. }
	\vspace{0.5em}
	\begin{tabular}{c|c|c||c|c}
		 $F_{layout}$ & \multicolumn{2}{c||}{Single Image}  & \multicolumn{2}{c}{Single Video}  
		\tabularnewline
		 {} channels & {{} SIFID~$\downarrow$}  & {{} LPIPS~$\uparrow$ } &  {{} SIFID~$\downarrow$} & {{} LPIPS~$\uparrow$ } \tabularnewline

		\hline 	\hline

		 1 & {{0.08}}  &  \textbf{{0.33}} &  {0.55} &  \textbf{{0.43}}  \tabularnewline
		 
		 3 & {{0.07}}  &  {0.28} &  {0.54} &  {0.41}  \tabularnewline
		 
		 5 & \textbf{{{0.06}}}  &  {0.25} &  {0.50} &  {0.40}  \tabularnewline
		 
		 10 & \textbf{{0.06}}  &  {0.24} &  \textbf{{0.49}} &  {0.40}  \tabularnewline

		\end{tabular}
%	\vspace{-0.5em}

\label{table:layout_width} %

\end{table}
