# Supplementary material for: Generating Novel Scene Compositions from Single Images and Videos
Source: arXiv:2103.13389 source file (2023-12-13)
Supplement: Supplementary file 24 [file low_level_loss.tex]

\begin{table}
	\vspace{-1.0em}
	\setlength{\tabcolsep}{0.2em}
	
	\centering
	\caption{Ablation on the low-level loss $\mathcal{L}_{D_{low\text{-}level}}$ on DAVIS-YFCC100M dataset. }
	\vspace{0.5em}
	\begin{tabular}{c|c|c||c|c}
		 {} Low-level & \multicolumn{2}{c||}{Single Image}  & \multicolumn{2}{c}{Single Video}  
		\tabularnewline
		 {} loss & {\small{} SIFID~$\downarrow$}  & {{} LPIPS~$\uparrow$ } &  {{} SIFID~$\downarrow$} & {{} LPIPS~$\uparrow$ } \tabularnewline

		\hline 	\hline 	
		
		 \xmark & \textbf{{{0.08}}}  &  {0.27} &  {0.58} &  {0.40}  \tabularnewline
		
		 \cmark & \textbf{{{0.08}}}  &  \textbf{{0.33}} &  \textbf{{0.55}} &  \textbf{{0.43}}  \tabularnewline
	
		\end{tabular}
%	\vspace{-0.5em}

\label{table:low_level_loss} %

\end{table}
