# Supplementary material for: Generating Novel Scene Compositions from Single Images and Videos
Source: arXiv:2103.13389 source file (2023-12-13)
Supplement: Supplementary file 25 [file other_with_dr.tex]

\begin{table}
	\vspace{-0.5em}
	\setlength{\tabcolsep}{0.35em}
	
	\centering
	\caption{Effect of DR applied to different GAN models in the Single Image setting on DAVIS-YFCC100M.}
	\vspace{0.5em}
	\begin{tabular}{cc|c|c|c|c|c}
		\multirow{2}{*}{{} Method} & {{DR} } & \multirow{2}{*}{{} SIFID~$\downarrow$} & \multirow{2}{*}{{} LPIPS~$\uparrow$ } & \multirow{2}{*}{{} MS-SSIM~$\downarrow$} & {{} Pixel ~$\uparrow$} & {Dist.}  \tabularnewline
		& {$\lambda$} & & & & {} Diversity & to train \tabularnewline
		
		\hline 	\hline 	
		
		{{} \multirow{2}{*}{SinGAN }} & { -} &  \textbf{{{0.13}}}  &  \textbf{{0.26}} & {0.69} &  {0.54} &  {0.24} \tabularnewline
		 & { 0.15} &  {{0.15}}  &   \textbf{{0.26}} &  \textbf{{0.68}} &  \textbf{{0.55}}  &  \textbf{0.26} \tabularnewline 	\hline

		{{} \multirow{2}{*}{ConSinGAN }} & { -} &  \textbf{{{0.09}}}  &   {0.29} &  {0.65} &  {0.59}  &  {0.25} \tabularnewline
& { 0.05} &  {{0.11}}  &   \textbf{{0.30}} &  \textbf{{0.63}} &  \textbf{{0.60}}  &  \textbf{0.28}  \tabularnewline 	\hline 
		
		{{} \multirow{2}{*}{FastGAN  }} & { -} &  \textbf{{{0.13}}}  &   {0.18} &  {0.77} &{0.49}  &  {0.08}  \tabularnewline
& { 0.15} &  {{0.14}}  &   \textbf{{0.21}} &  \textbf{{0.74}} &  \textbf{{0.52}}  &  \textbf{0.13}  \tabularnewline 	\hline 
	
		{{} \multirow{2}{*}{SIV-GAN  }} & { -} &  \textbf{{{0.05}}}  &  {0.04} & {0.95} & {0.33}  &  {0.06}  \tabularnewline
& { 0.15} &  {{0.08}}  &  \textbf{{0.33}} & \textbf{{0.63}} &  \textbf{{0.66}}  &  \textbf{0.31} \tabularnewline 
		
	\end{tabular}
	%\vspace{-0.5em}
	\label{table:other_with_DR} %
	\vspace{-1em}
\end{table}
