# Supplementary material for: Generating Novel Scene Compositions from Single Images and Videos
Source: arXiv:2103.13389 source file (2023-12-13)
Supplement: Supplementary file 26 [file single_video_div.tex]

\begin{table}[h!]

	\setlength{\tabcolsep}{0.20em}
	
	\centering
	\caption{Comparison of SIFID at different scales on DAVIS-YFCC100M in the Single Image and Single Video settings.}
	\begin{tabular}{c|cccc@{\hskip 0.10in}|@{\hskip 0.10in}cccc}
		
		\multirow{2}{*}{\normalsize{} } &  \multicolumn{4}{c}{{} Single Image} &  \multicolumn{4}{c}{{} Single Video}    \tabularnewline
		
		%\multirow{2}{*}{\normalsize{} Method } &  \multicolumn{4}{c}{{} SIFID~$\downarrow$}    \tabularnewline
		& \footnotesize{$\frac{H\times W}{4}$} & \footnotesize{$\frac{H\times W}{8}$} & \footnotesize{$\frac{H\times W}{16}$} & \footnotesize{$1\times 1$} & \footnotesize{$\frac{H\times W}{4}$} & \footnotesize{$\frac{H\times W}{8}$} & \footnotesize{$\frac{H\times W}{16}$} & \footnotesize{$1\times 1$} \tabularnewline
		
		\hline 	\hline 	
		
		{{} SinGAN} & {0.13}  & {4.93}    &  {34.52} & {2510} & {2.47}  & {13.61}    &  {96.35} & {411}   \tabularnewline

		{{} ConSinGAN} & {0.09} & {2.94}  &    {27.33} & {1960}  & {2.74} & {14.73}  &    {74.50} & {392}  \tabularnewline
		
		{{} FastGAN}  & {0.13} & {2.89} & {{19.48}} & {1340} & {0.79} & {1.75} & {{9.24}} & {141}  \tabularnewline		
		
		{{} SIV-GAN }  & \textbf{{{0.08}}} & \textbf{{1.29}} & \textbf{{16.30}} & \textbf{{1100}} & \textbf{{{0.55}}} & \textbf{{1.32}} & \textbf{{5.14}} & \textbf{{115}}
		
		\tabularnewline 
		%{{} Data augment. }  & {{}} & {} & {} & {}
		%\tabularnewline		
	\end{tabular}
	\vspace{-0.5em}
	\label{table:single_image_fid} %
	
\end{table}
